# Supplementary material for: Towards Automated Discovery of Asymmetric Mempool DoS in Blockchains
Source: arXiv:2312.02642 source file (2025-05-26)
Supplement: Supplementary file 1 [file wellmarked_appendix_bw.tex]

\section{Observations Motivating \textsc{mpfuzz} Design}
\label{sec:motive}

\noindent{\bf
(In)feasibility of code-coverage-only stateless fuzzing}:
To fuzz a mempool, a baseline design is to use a code-coverage-based fuzzer. In each iteration, the fuzzer generates a bit string, parses it into a sequence of transactions and sends them to the tested mempool for execution. Upon each end state, it checks whether the test oracle defined above is satisfied. This design takes code coverage as the only feedback and is stateless because the feedback does not consider the end state. 

The stateless design would be ineffective in fuzzing mempool or finding ADAMS exploits. For example, consider fuzzing a three-slot mempool to find a DETER-X exploit consisting of three future transactions~\cite{DBLP:conf/ccs/LiWT21}. Suppose the current mempool input is a sequence of one future transaction. After mutation, it may try an input of two future transactions, which, however, does not increase code coverage (the second future transaction is executed by the same code path in a mempool as the first future transaction). Thus, the fuzzer discards the two-future-transaction input and misses finding the three-future-transaction exploit. We validate the ineffectiveness of stateless fuzzer by experiments in \S~\ref{sec:eval:fuzz}. 

A more promising design is stateful mempool fuzzing, in which the mempool state is included in the feedback to guide next-iteration fuzzing. In the previous example of finding a three-future-transaction exploit (DETER-X), sending two future transactions leads to a different mempool state than sending one. A simple state-coverage-based fuzzer would view this as positive feedback and further explore this direction toward finding the three-future-transaction exploit.

\noindent{\bf
(In)feasibility of existing consensus fuzzers}: Existing consensus fuzzers~\cite{me:tyr,DBLP:conf/ndss/MaCRZ00L023,DBLP:conf/osdi/YangKC21} cannot detect mempool DoS or ADAMS bugs. Specifically, Loki's test oracle is detecting system crashes, while a successful ADAMS attack does not necessarily trigger system crashes. Using Loki to detect ADAMS would cause many false negatives.

Fluffy detects the unsynchronizable difference of post-consensus states as vulnerability. However, the mempools in two clients, say Geth and Besu under benign transactions, would be different. In other words, post-consensus state differences across clients could indicate insecurity, but the difference in pre-consensus states across clients, like mempool, does not mean insecurity. Using Fluffly to detect ADAMS could cause false positives.

Tyr's test oracle detects property violations on post-consensus states. Particularly, while Tyr models state liveness, their definition ``valid transactions should be executed eventually'' is, unfortunately, over-simplifying and fails to model the legitimate pre-consensus cases in real Ethereum clients; for instance, valid transactions of low Gas price can be dropped by Ethereum mempools and will not be eventually executed. Besides, they model double-spending transactions as the only type of invalid transaction. In Ethereum, double-spending transactions are of the same nonce. And there are many more sophisticated invalid transactions in Ethereum that Tyr does not model, including future transactions, latent overdrafts, etc. 
%Known mempool DoS like DETER already use these sophisticated invalid transactions to construct an attack, and Tyr could not detect it.

We analyze the case of existing consensus fuzzers in detecting known DETER attacks~\cite{DBLP:conf/ccs/LiWT21}. Loki cannot detect DETER because DETER does not cause system crashes. Fluffy does not model future transactions and can not find the DETER attacks that rely on future transactions. Similarly, Tyr that does not model sophisticated invalid transactions would miss detecting DETER attacks.

\noindent{\bf Challenges}:
In stateful mempool fuzzing, the essential design problem is {\it how to generate the next input transaction given a current ``state''}. State $st$ is the collection of transactions in the mempool and those included in the blockchain. 

\subsection{Further Rationale of Symbolization}
\label{appdx:sec:sym:rationale}

%\noindent{\bf Design rationale}: 
We now describe the design rationale of our symbolization technique. 
%We aim to explain why \textsc{mpfuzz} can instantiate a symbol to a much smaller subset (than the defining space), without losing the fuzzing utility (i.e., without missing exploits).

\begin{itemize}
\item
The first observation is that {\it real-world mempools admit transactions based on the symbolic value, not concrete value, of nonce and Ether amount}. Our design reflects this intuition. For instance, symbols of valid transactions, e.g., $\mathcal{P}, \mathcal{C}, \mathcal{N}$, are instantiated by \textsc{mpfuzz} to a minimal amount $1$ Ether. As long as the transferred Ether amount does not exceed the sender balance, transactions remain valid (i.e., no overdraft). Admission decisions remain the same for two valid transactions despite their difference in nonces or Ether amounts.  

Likewise, Symbol $\mathcal{F}$ is instantiated by \textsc{mpfuzz} to fixed nonce $n+1$: As long as the nonce is non-consecutive, no matter what specific value it takes (e.g., $3$ or $m+1$), the mempool would deem it as a future transaction and makes the same admission decision. 

As a side note, the nonce of Symbol $\mathcal{F}$ is fixed at a large nonce $n+1$ (we denote it by far future transactions) instead of a small nonce, say $5$ (we denote it by near future transactions), because near future transactions' nonce could be reconnected as consecutive and lead to duplicated states. 
%For instance, input sequence of transactions $A^5_1, A^5_3, A^5_2$ and sequence of $A^5_1, A^5_2, A^5_3$ lead to the same mempool state.

\item
The second observation is that {\it restricting eviction/replacement victims to only parent transactions can facilitate finding exploits quickly}. Specifically, while any transactions can be evicted/replaced, \textsc{mpfuzz} evicts/replaces only parent transactions; such a strategy can cause maximal damage (i.e., the most child transactions turned) while saving the search space. Our symbol design reflects this idea. For instance, Symbol $\mathcal{R}$ covers any transaction of the same sender and nonce as a transaction in state $st$, but it is instantiated by \textsc{mpfuzz} to only the transaction of nonce $1$ (i.e., replacing a parent transaction).

For another instance, Symbol $\mathcal{C}$ is instantiated to a high Gas price $m+1$, Symbol $\mathcal{P}$ is instantiated to medium price $[4,m]$, and Symbol $\mathcal{N}$ is instantiated to a low price $3$. So, $\mathcal{C}$ can evict $\mathcal{P}$ or $\mathcal{N}$.
\end{itemize}

\section{Case Study: How \textsc{mpfuzz} Finds Exploits}

We describe how \textsc{mpfuzz} finds an exploit that evades the defense. We present a case study on finding $XT_6$ in the latest Geth $\geq{}v1.14.11$. 

{  \noindent{\bf 
Mempool reduction}: Recall that a Geth mempool has a capacity of $m'=6144$ slots, and its transaction-admission policies are characterized by three essential parameters: admitting up to $py_1'=1024$ future transactions and limiting up to $py_2'=16$ pending transactions from any senders when more than $py_3'=5120$ pending transactions are residing in the mempool. 
We set up the MUT to run the same codebase or the same admission policy but with different, smaller parameters: $m=3, py_1=1, py_2=2, py_3=2$ . What follows is a description of how \textsc{mpfuzz} would find a short exploit of $XT_6$ on this MUT.
}

\noindent{\bf 
Fuzzing: How \textsc{mpfuzz} automatically finds exploits}:
Initially, the mempool is filled with $m=3$ normal transactions. That is, the initial symbolized state is $\mathcal{NNN}$.
The seed corpus $sdb$ initially contains an empty string. \textsc{mpfuzz} retrieves the empty string and appends to it with different symbols $\mathcal{L}_0$, $\mathcal{C}_0$, $\mathcal{P}_0$. Because of the initial state $\mathcal{NNN}$, only Symbol $\mathcal{P}_0$ is feasible. It generates the mutated input $\mathcal{P}$ and instantiates it to a parent transaction of a higher fee than normal transactions (as described in \S~\ref{sec:symbolize}). Sending the input to the mempool gets the transaction admitted, leading to transitioned state $st_1=\mathcal{NNP}$. This is a new state that is not in the corpus, and it evicts more normal transactions $\mathcal{N}$ than the previous state $st_0$; the input produces positive feedback, and the associated input-state pair $\langle{}P,st_1=\mathcal{NNP}\rangle{}$ is added to the corpus.

\begin{wrapfigure}{r}{0.26\textwidth}
%\begin{figure}[!bthp]
\centering
\includegraphics[width=0.25\textwidth]{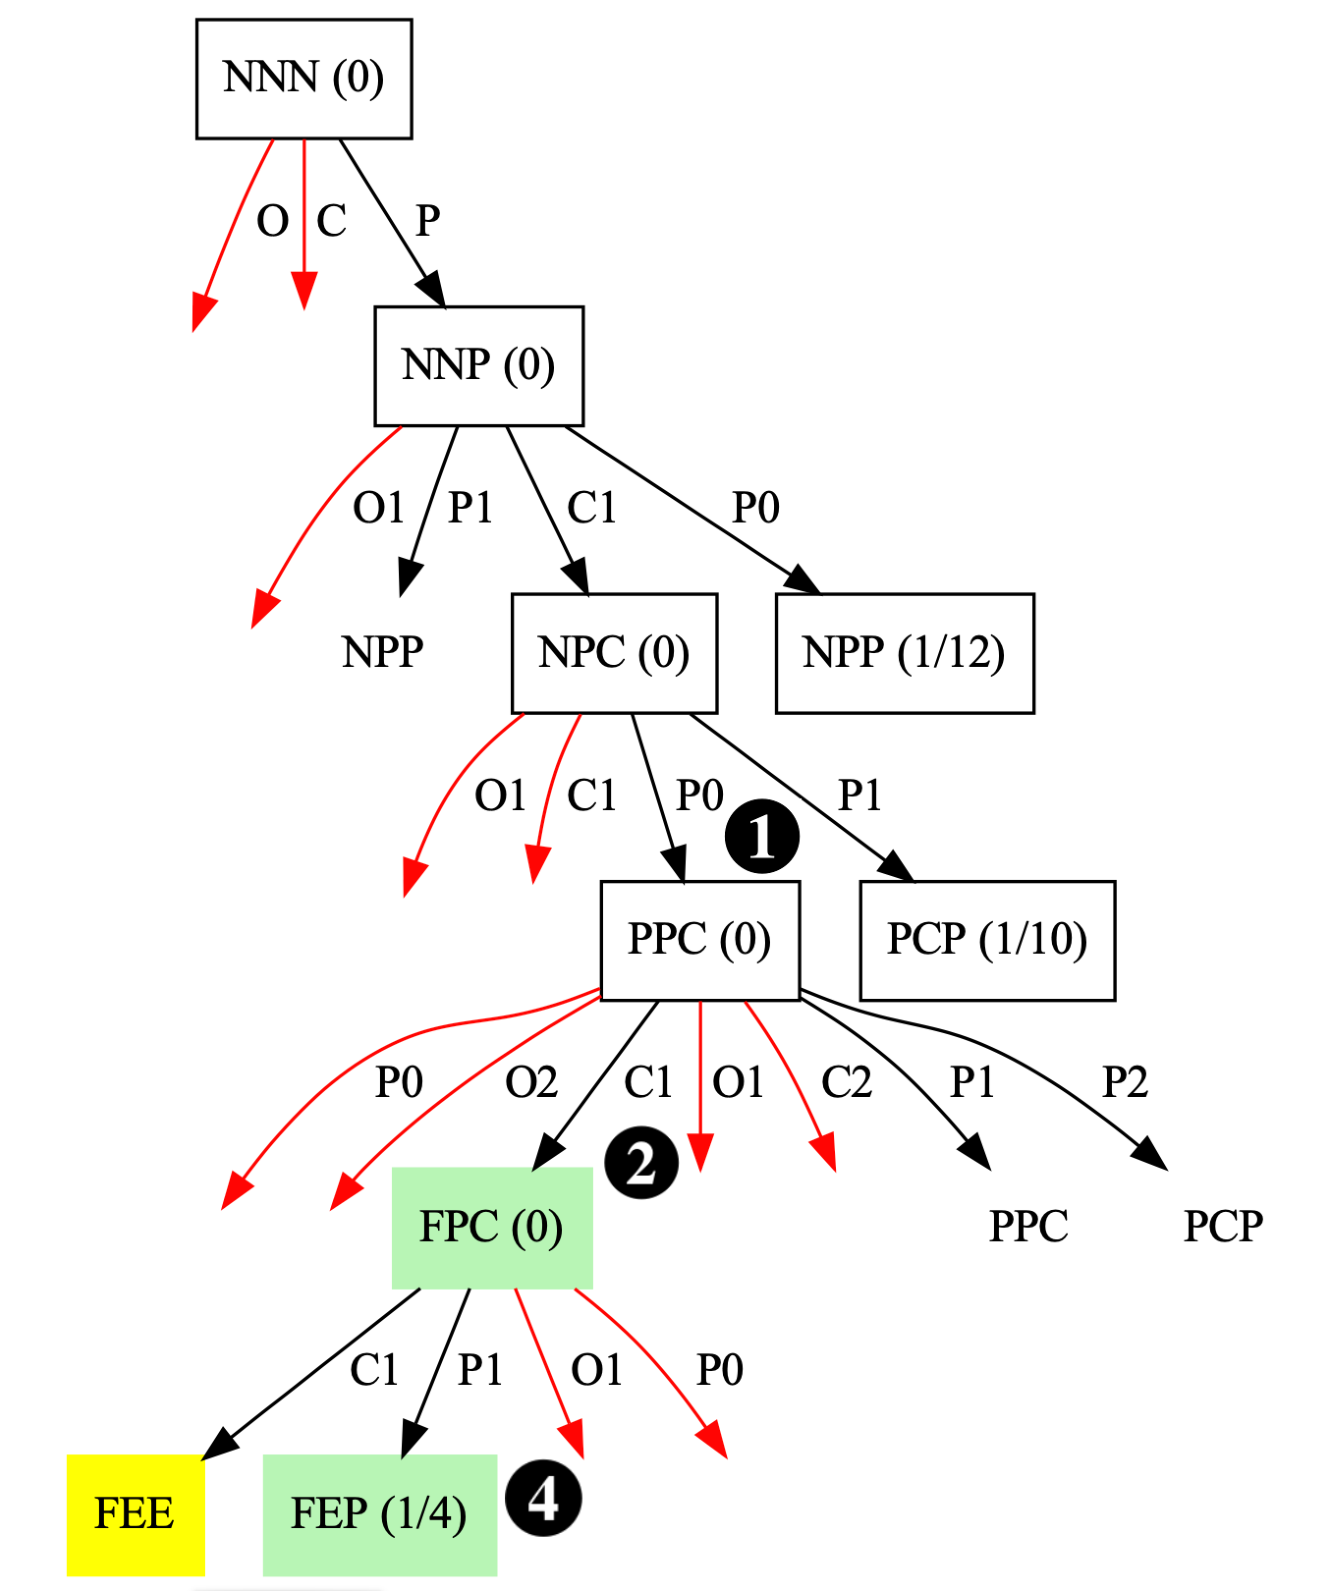}
\caption{Snapshot of the \textsc{mpfuzz} state-search tree when finding Exploit $XT_6$ on Geth $v1.11.4$ .}
\label{fig:fuzzing:ex2}
%\end{figure}
\end{wrapfigure}

Next, \textsc{mpfuzz} retrieves from $sdb$ a seed by high energy. According to Table~\ref{tab:symbols:2}, the energy of state $\mathcal{NNN}$ is $\frac{1}{3*3}*0$, and the energy of state $\mathcal{NNP}$ is $\frac{1}{3*2+4}*1=1/10>0$. Hence, seed $\mathcal{NNP}$ is selected. \textsc{mpfuzz} tries input mutation and appends to the selected input $\mathcal{P}$ one of four new symbols, that is, $\mathcal{L}_1$, $\mathcal{C}_1$, $\mathcal{P}_0$ or $\mathcal{P}_1$. On state $\mathcal{NNP}$, 1) mutation transaction instantiated from symbol $\mathcal{L}_1$ is declined admission. 2) Mutation transaction from $\mathcal{C}_1$ is admitted, transitioning the state to $\mathcal{NPC}$, which produces positive feedback and is added to $sdb$. 3) Likewise, transaction $\mathcal{P}_0$ is admitted and produces state $\mathcal{NPP}$ of positive feedback; the mutated input is also added to $sdb$. 4) Mutation $\mathcal{P}_1$ is admitted but produces an identical state with mutation $\mathcal{P}_0$; thus, the mutated input is not added to $sdb$.

Now, there are four seeds in $sdb$: $\mathcal{NNN} (0)$, $\mathcal{NNP} (0)$, $\mathcal{NPC} (1/8)$, and $\mathcal{NPP} (1/12)$. In parentheses are their energy numbers. The seed of the highest energy $\mathcal{NPC} (1/8)$ is selected (i.e., Step \ballnumber{1} in Figure~\ref{fig:fuzzing:ex2}). \textsc{mpfuzz} then mutates $\mathcal{NPC}$ with four possibilities, that is, $\mathcal{L}_1$, $\mathcal{C}_1$, $\mathcal{P}_0$, and $\mathcal{P}_1$, which produce two end states with positive-feedback, that is, $\mathcal{PPC}$ and $\mathcal{PCP}$. They are added to the $sdb$ with energy $\mathcal{PPC} (1/10)$ and $\mathcal{PCP} (1/10)$. 

Let's say $\mathcal{PPC} (1/10)$ is selected (\ballnumber{2}). \textsc{mpfuzz} then mutates input $\mathcal{P}\mathcal{C}_1\mathcal{P}_0$ with seven mutation transactions, that is, $\mathcal{L}_1, \mathcal{L}_2, \mathcal{C}_1, \mathcal{C}_2, \mathcal{P}_0, \mathcal{P}_1, \mathcal{P}_2$, which produces one end state with positive feedback, that is, mutation $\mathcal{C}_1$ is admitted and transitions state to $\mathcal{FPC} (1/5)$. After being added to the $sdb$, $\mathcal{FPC}$ is the one with the highest energy and is chosen for the next-round fuzzing (\ballnumber{4}). \textsc{mpfuzz} mutates input $\mathcal{P}\mathcal{C}_1\mathcal{P}_0\mathcal{C}_1$ with four mutations and produces two state transitions with positive feedback. That is, upon state $\mathcal{FPC}$, mutation $\mathcal{C}_1$ is admitted and leads to state $\mathcal{FEE}$, which 
satisfies the bug oracle of eviction attacks under $\epsilon=0$. The algorithm then emits the found short exploit: $\langle{}st_0=\mathcal{NNN}, dc_0=\emptyset\rangle{}, ops=\mathcal{P}\mathcal{C}_1\mathcal{P}_0\mathcal{C}_1\mathcal{C}_1$ (recall Definition~\ref{def:timeline}).

Besides, upon state $\mathcal{FPC}$, the mutation $\mathcal{P}_1$ is admitted that transits the state to $\mathcal{FEP} (1/4)$. State $\mathcal{FEP}$ is added to $sdb$ for fuzzing. The snapshot of the state-search tree is depicted in Figure~\ref{fig:fuzzing:ex2}. 

{  
\noindent{\bf Exploit extension}: Given the short exploit automatically found on MUT (with $m=3, py_1=1, py_2=2, py_3=2$), the next step is to extend it to a longer exploit functional on the actual Geth mempool (with $m'=6144, py_1'=1024, py_2'=16, py_3'=5120$).

Exploit extension requires manual efforts: After identifying exploit $\langle{}st_0=\mathcal{NNN}, dc_0=\emptyset\rangle{}, ops=\mathcal{P}\mathcal{C}_1\mathcal{P}_0\mathcal{C}_1\mathcal{C}_1$ is unique, we extend it to the longer exploit by ensuring the same admission event occurs on the actual mempool as on the smaller MUT. 
%XXX
In this process, it tries the next transaction of the same sender with the previous one but with an incremented nonce. If it fails, it switches to the next sender. It also tries transaction fees/prices based on measuring the fees of actual normal transactions, which may not be fixed as $3$ in the \textsc{mpfuzz} setting. 
%Eventually, in the extended exploit, there are first $384$ transaction sequences, each  of $16$ transactions from a distinct sender, and then $384$ transactions; the $384$ transactions evict the $384$ .
}

\section{Additional Eval. of \textsc{mpfuzz} Performance}

\label{appdx:sec:mpfuzzeval:acrossclients}

We further run our \textsc{mpfuzz} on different clients,  including Geth $v1.10.11$, Geth $v1.11.4$, Erigon $v2.42.0$, and Nethermind $v1.18.0$. The tested mempool is configured at $16$ slots. We report the number of exploits found by \textsc{mpfuzz} in a $16$-hour period. 
Figure~\ref{fig:exploits-found} presents the result that \textsc{mpfuzz} finds $4096$ short exploits in the first $8$ hours on Geth-$v1.10.11$. On Geth-$v1.11.4$, \textsc{mpfuzz} quickly finds one exploit (i.e., exploit $XT_6$ as described in \S~\ref{sec:foundevictionattacks}) within $2$ minutes and does not find anymore in the next $16$ hours. On Nethermind, it finds one exploit (exploit $XT_1$) within two minutes and finds the next one (exploit $XT_4$) near the end of $16$-th hour. On Erigon, it finds one exploit ($XT_4$) in the $16$-th hour. 

%The reason that \textsc{mpfuzz} finds exploits much faster on Geth than on other clients is the following: Geth provides a RPC interface to reinitialize a mempool by clearing transactions without restarting the client node, while reinitializing mempools on other clients is more cumbersome (need restarting the node).

%\begin{figure}[!ht]
%  \centering
%   \includegraphics[width=0.25\textwidth]{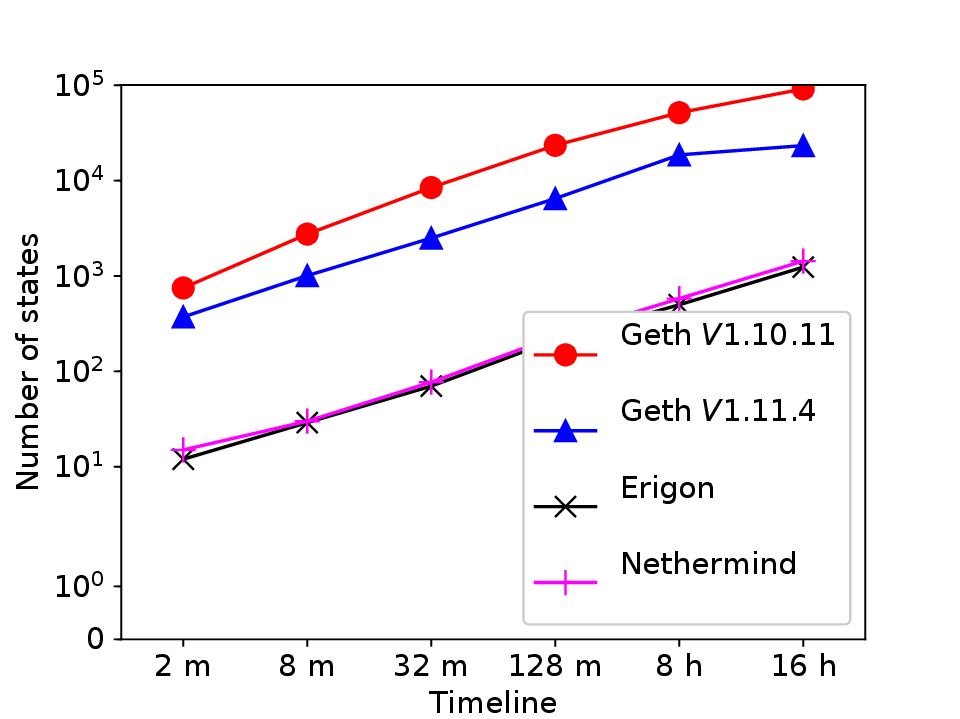}
%  \caption{\textsc{mpfuzz} on different clients: Number of states covered on 16-slot mempool in 16 %hours}%
%  \label{fig:state-covered}
%\end{figure}
\begin{figure}[!htb]
  \begin{minipage}{0.22\textwidth}
    \centering
    \includegraphics[width=.99\linewidth]{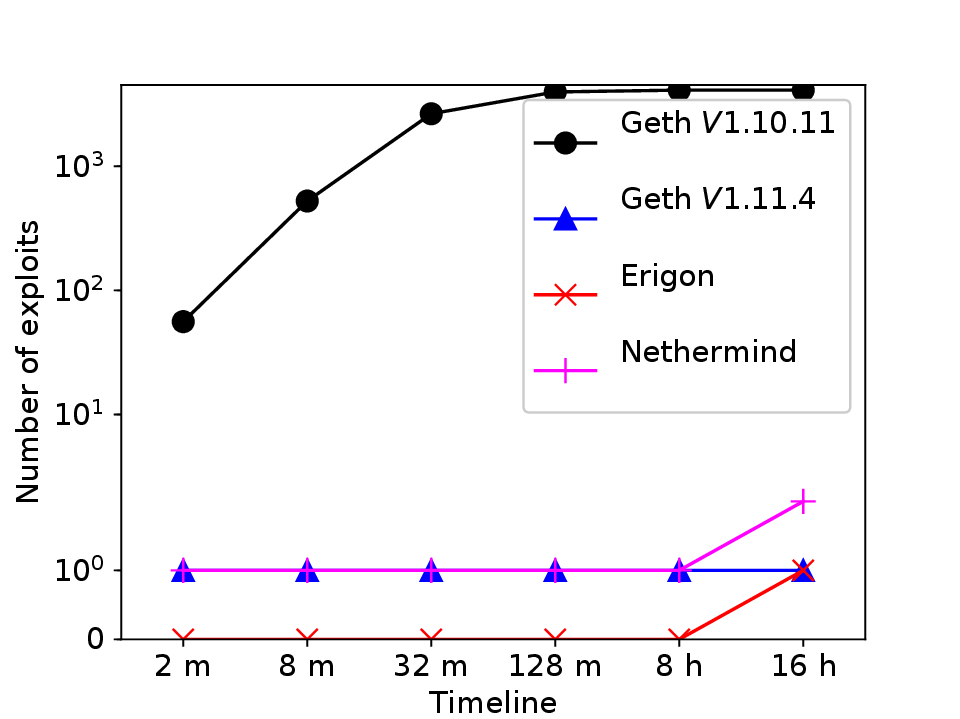}
    %\caption{\textsc{mpfuzz} on different clients: Number of found exploits on 16-slot mempool in 16 hours.}\label{fig:exploits-found}
    \caption{\# exploits found}\label{fig:exploits-found}
  \end{minipage}\hfill
  \begin{minipage}{0.22\textwidth}
    \centering
    \includegraphics[width=.99\linewidth]{figures/fuzz-state.eps}
    %\caption{\textsc{mpfuzz} on different clients: Number of states covered on 16-slot mempool in 16 hours.}\label{fig:state-covered}
    \caption{\# states covered}\label{fig:state-covered}
  \end{minipage}
\end{figure}

Figure~\ref{fig:state-covered} shows the number of states that are explored by \textsc{mpfuzz} on a $16$-slot mempool
in 16 hours. \textsc{mpfuzz} explores $749$ and $91428$ states on Geth $v1.10.11$ in $2$ minutes and $16$ hours respectively. On Geth $v1.11.4$, \textsc{mpfuzz} explores $372$ and $23286$ states in $2$ minutes and $16$ hours respectively. However, the performance of Erigon and Nethermind is much lower than that of Geth. \textsc{mpfuzz} explores $12$ and $1239$ states on Erigon in $2$ minutes and $16$ hours respectively. On Nethermind, \textsc{mpfuzz} explores $15$ and $1433$ states in $2$ minutes and $16$ hours, respectively. 
The reason \textsc{mpfuzz} is more performant on Geth is that we implemented an external API on Geth to initialize the mempool; in each iteration of fuzzing on Geth, \textsc{mpfuzz} calls the API to initialize the mempool. In contrast, on Nethermind and Erigon, \textsc{mpfuzz} restarts the client in each iteration, which is consuming.

%%%OVERPAGE

\section{Additional Attack Evaluation}
\label{appdx:sec:additional-attack-evaluation}

\subsection{Experiment on a Single Victim Node}
\label{sec:setup:singlenode}

\begin{figure}[!bthp]
\centering
\includegraphics[width=0.375\textwidth]{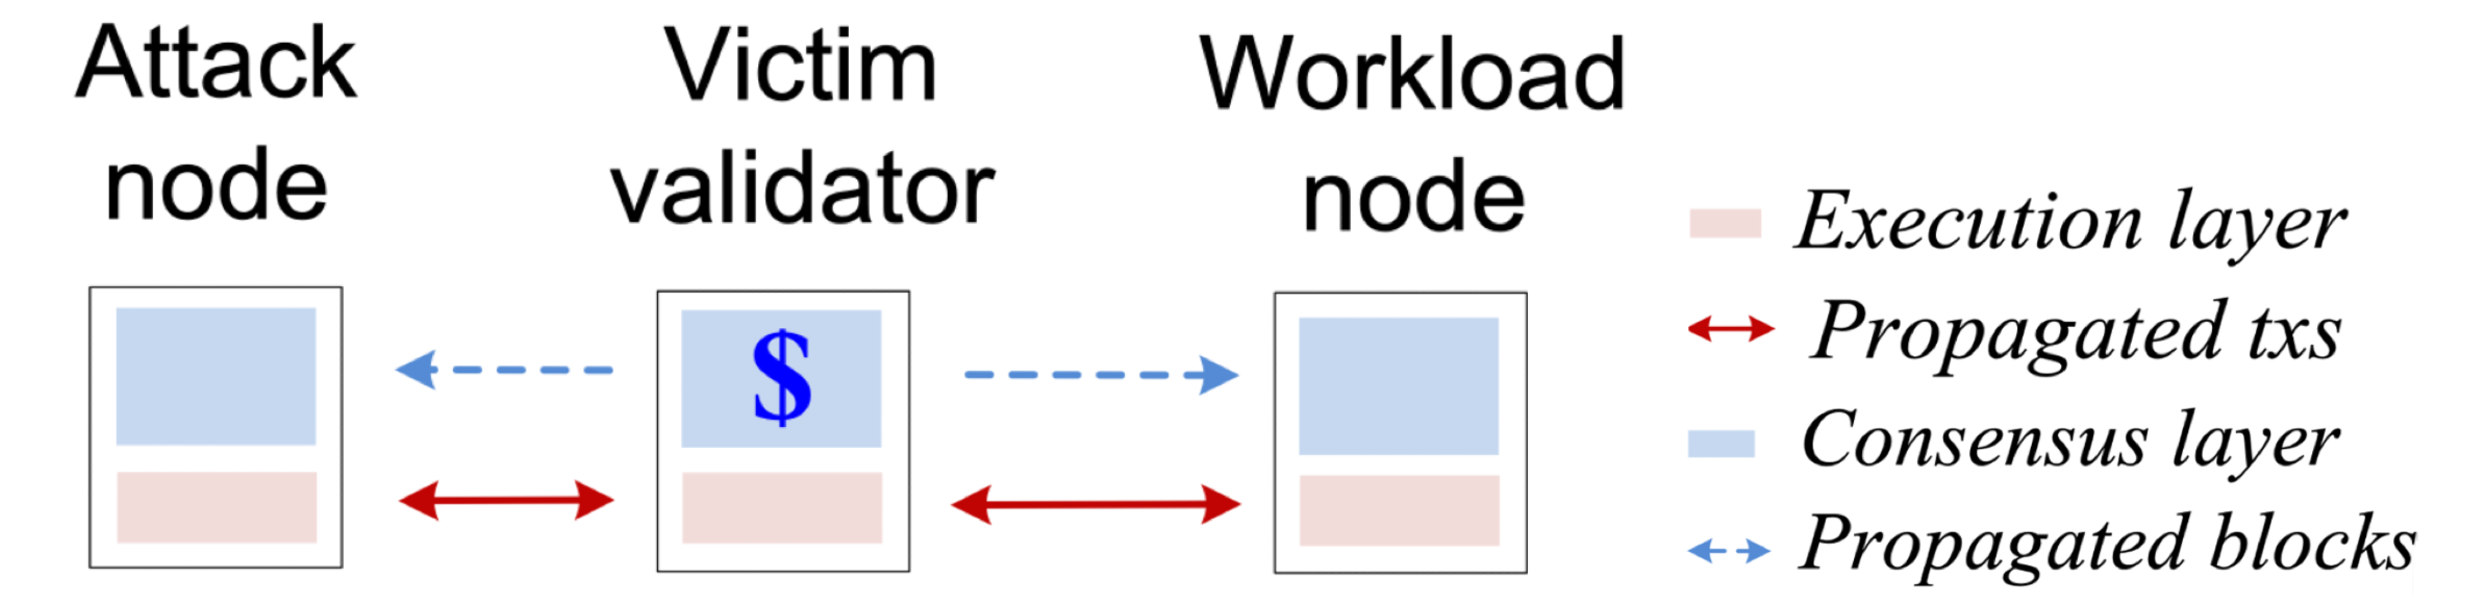}
\caption{Experimental setup}
\label{fig:exp:setup}
\end{figure}

\label{appdx:sec:eval:local:1}
\noindent{\bf Evaluation settings}:
Our goal is to evaluate the success rate and cost of different ADAMS attacks on a single victim node. Because some ADAMS attacks are sensitive to the workload of normal transactions, we first collect transaction workloads from the mainnet. Specifically, we instrumented a Geth client (denoted by Geth-m) to log every message it receives from every neighbor. The logged messages contain transactions, transaction hashes (announcements), and blocks. When the client receives the same message from multiple neighbors, it logs it as multiple message-neighbor pairs. 
We also log the arrival time of a transaction or a block.

{\it Workload collection}: 
We launched a Geth-m node in the mainnet on May 17, 2023, turned on logging for $5$ hours, and collected the transactions propagated to it. We make the collected transactions replayable as follows: We use the account balances and nonces on the mainnet to set up the initial state locally. We then replace the original sender in the collected transactions with the public keys that we generated. By this means, we know the secret keys of transaction senders and are able to send the otherwise same transactions for experiments. 

For experiments, we set up three nodes, an attack node sending crafted transactions, a workload node sending normal transactions collected, and a victim node receiving transactions from the other two nodes. The victim node is connected to both the attack and workload nodes. There is no direct connection between the attack node and the workload node. The attacker node runs an instrumented Geth $v1.11.4$ client (denoted by Geth-a) that can propagate invalid transactions to its neighbors. The victim node runs the tested Ethereum client. The workload node runs a vanilla Geth $v1.11.4$ client. On each node, we also run a Prysm $v3.3.0$ client at the consensus layer. The experiment platform is denoted in Figure~\ref{fig:exp:setup}.
Among the three nodes, we stake Ether to the consensus-layer client on the victim node, so that only the victim node would propose or produce blocks. 

In each experiment, we first run the above ``attacked'' setup (i.e., with victim, attack and workload nodes). We then run a ``regular'' setup that excludes the attack node. Under the regular setup, the workload node sends the normal transactions and blocks to the victim node. We compare the experiment results under the attacked setup and regular setup to show the success of the attack.

%\noindent{\bf {Experiments on Single Node}}

\ignore{
\begin{center}
\fbox{\parbox{0.90\linewidth}{RQ1. What's the success rate and attack cost in mounting turning-based exploits against a victim node running leading clients such as Geth, Erigon and Nethermind? 
}}
\end{center}
}

\noindent{\bf 
Evaluation of eviction/turning attacks on Single Node}:
We set up the experiment platform described in \S~\ref{sec:setup:singlenode}. In each experiment, we drive benign transactions from the workload node. Note that the collected workload contains the timings of both benign transactions and produced blocks. On the $30$-th block, we start the attack. Recall that each attack is configured by delay $d$; the attack node observes the arrival of a produced block and waits for $d$ seconds before sending a round of crafted transactions. 

The attack phase lasts for $40$ blocks; after the $70$-th block, we stop the attack node from sending crafted transactions. We keep running workload and victim nodes for another $50$ blocks and stop the entire process at the $120$-th block. We collect the blocks produced and, given a block, we report two metrics: 1) total fees of benign transactions included, 2) total fees of attack transactions included.

In each experiment, we also re-run the workload and victim nodes with the same setup. In this ``no-attack'', we don't run the attack node. We collect the blocks produced, and, given a block, we report two metrics: 3) total fees of transactions included (denoted as ``Benign ops - no attack''), and 4) the cost of a baseline spamming attack with 100\% success rate (denoted as ``Spamming - analytical''). For the latter, given a block, we select the transaction of the highest price, and report the price multiplied by the Ethereum block Gas limit. 

%We report the results for two representative eviction-based exploits: $XT_6$ which cannot lock the victim mempool, and $XT_4$ that can.

\begin{figure*}[!ht]
  \centering
  \subfloat[$XT_6$ w. $8$-sec. delay (single node)]{%
    \includegraphics[width=0.245\textwidth]{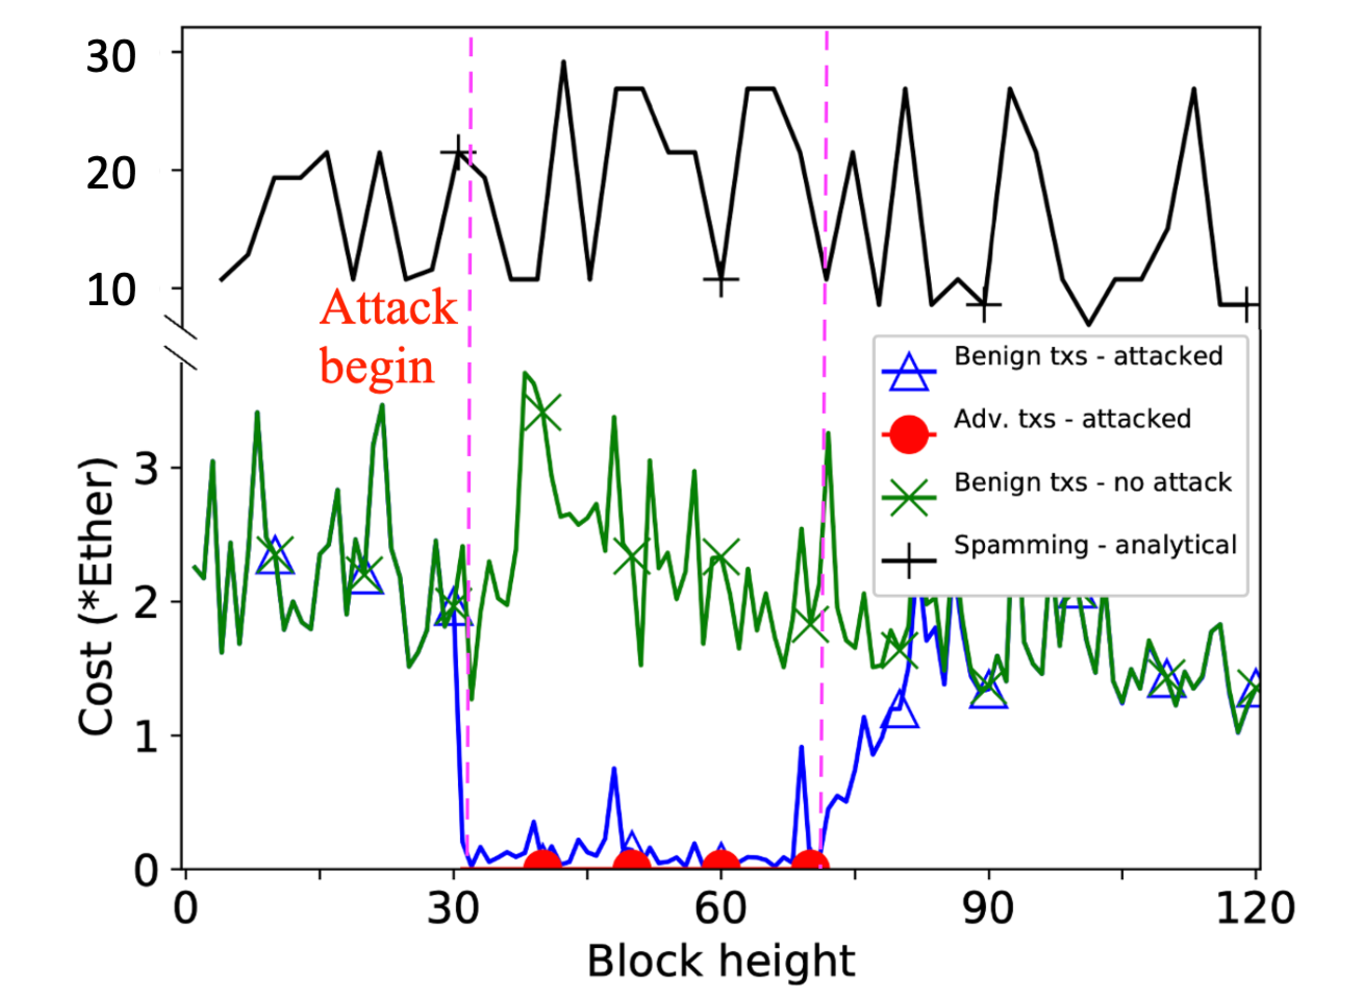}
    \label{fig:successrate-geth}}%
  \subfloat[$XT_6$ w. varying delay (single node)] {%
   \includegraphics[width=0.245\textwidth]{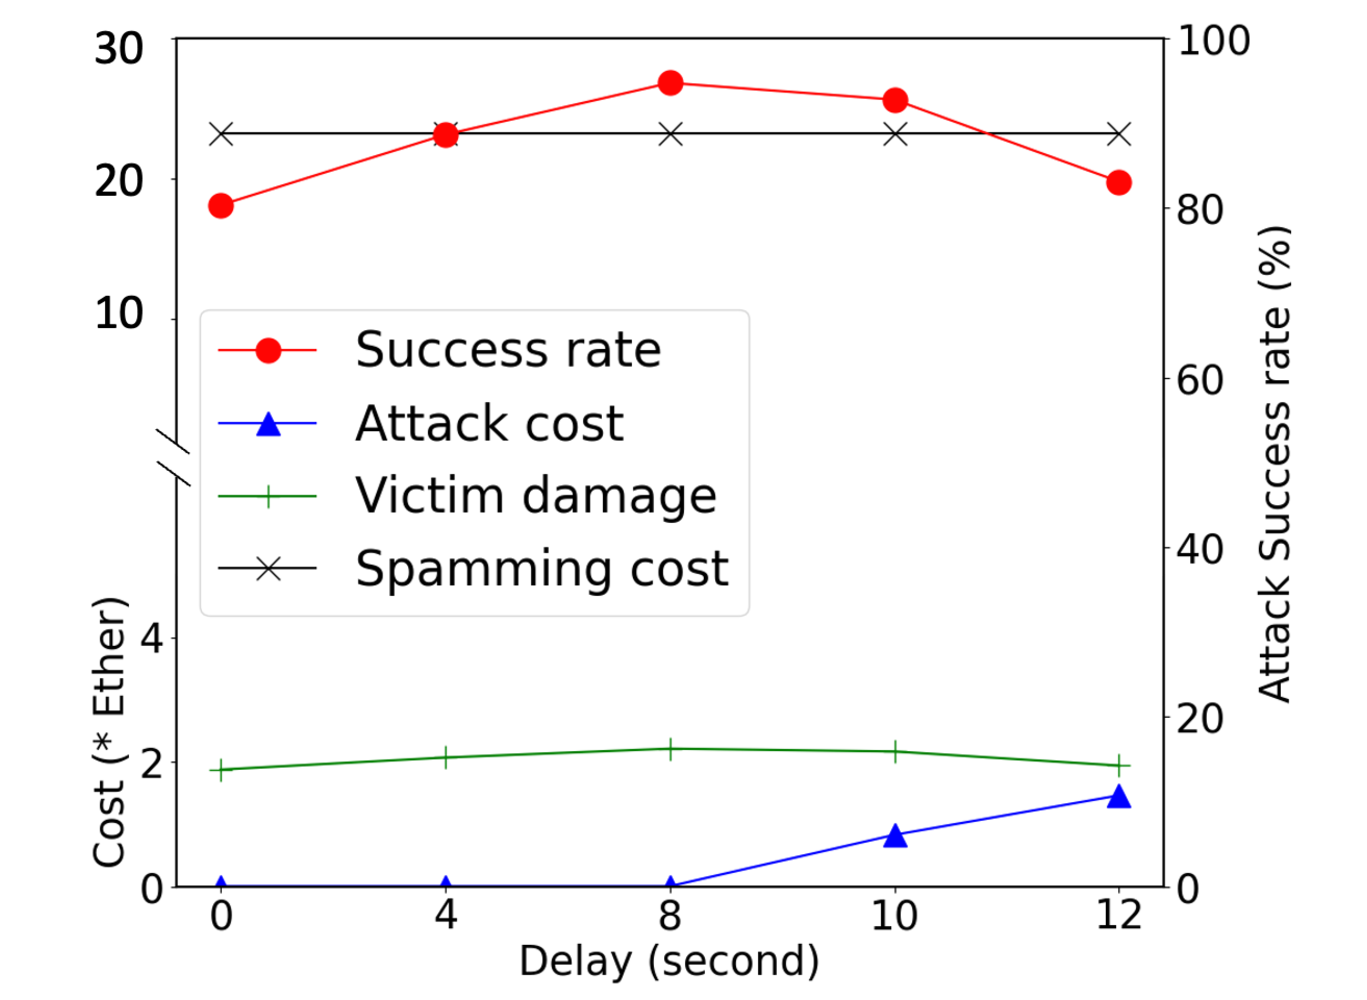}
  \label{fig:delay-geth}}
\ignore{
  \subfloat[Attack with $0$-second delay]{%
   \includegraphics[width=0.245\textwidth]{figures/nethermind-local-new2.eps}
  \label{fig:successrate-nethermind}}%
}
  \subfloat[$XT_4$ on Nethermind w. varying delay (single node)] {%
   \includegraphics[width=0.245\textwidth]{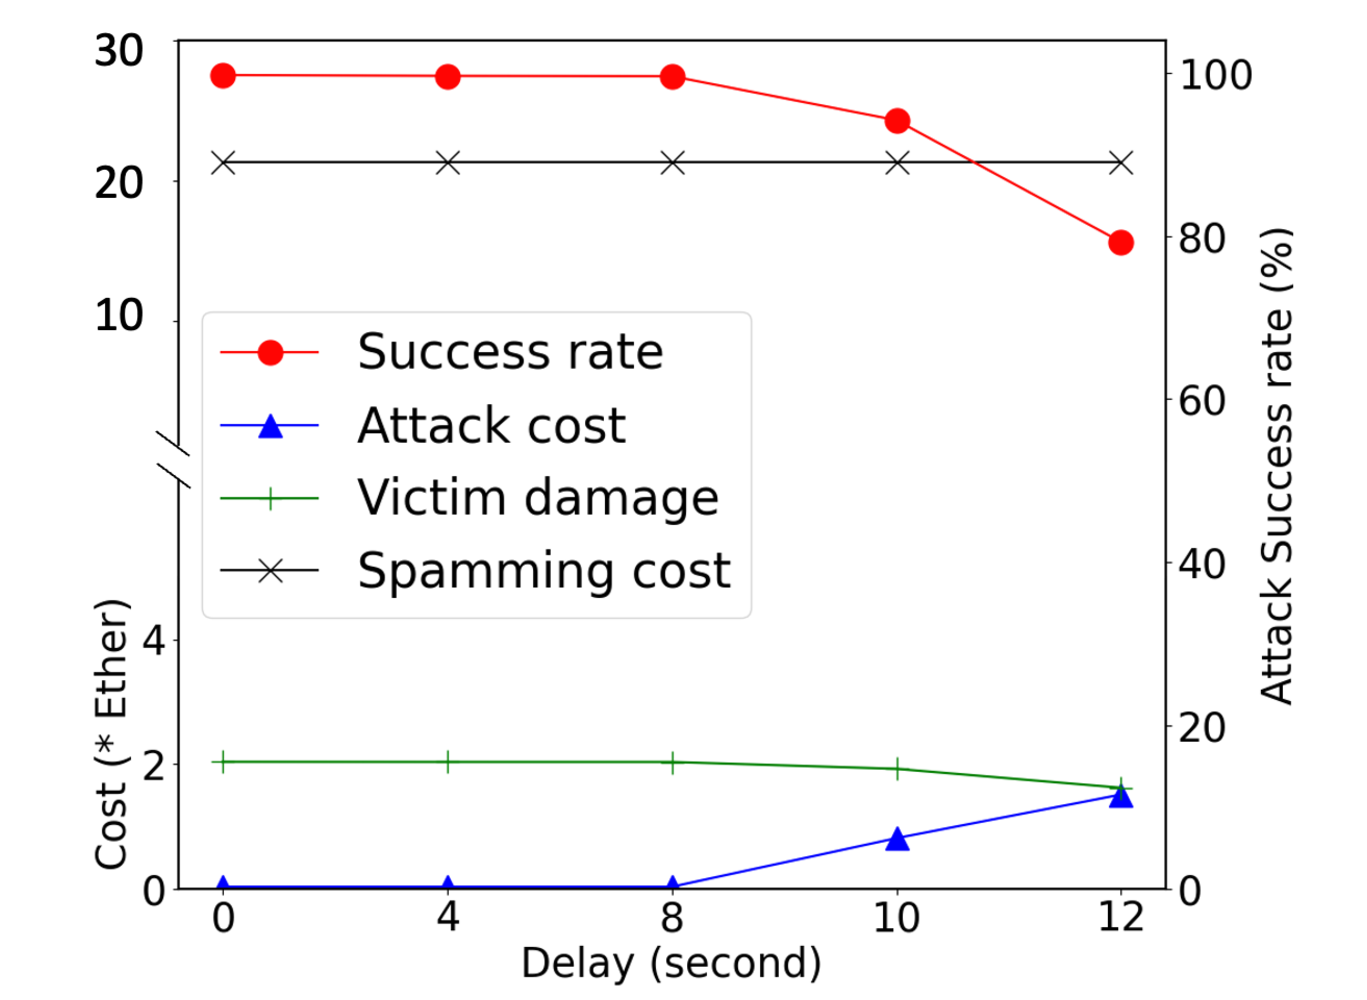}
  \label{fig:delay-nethermind}}
\ignore{
  \subfloat[Propagation Attack with $8$ seconds delay]{%
    \includegraphics[width=0.237\textwidth]{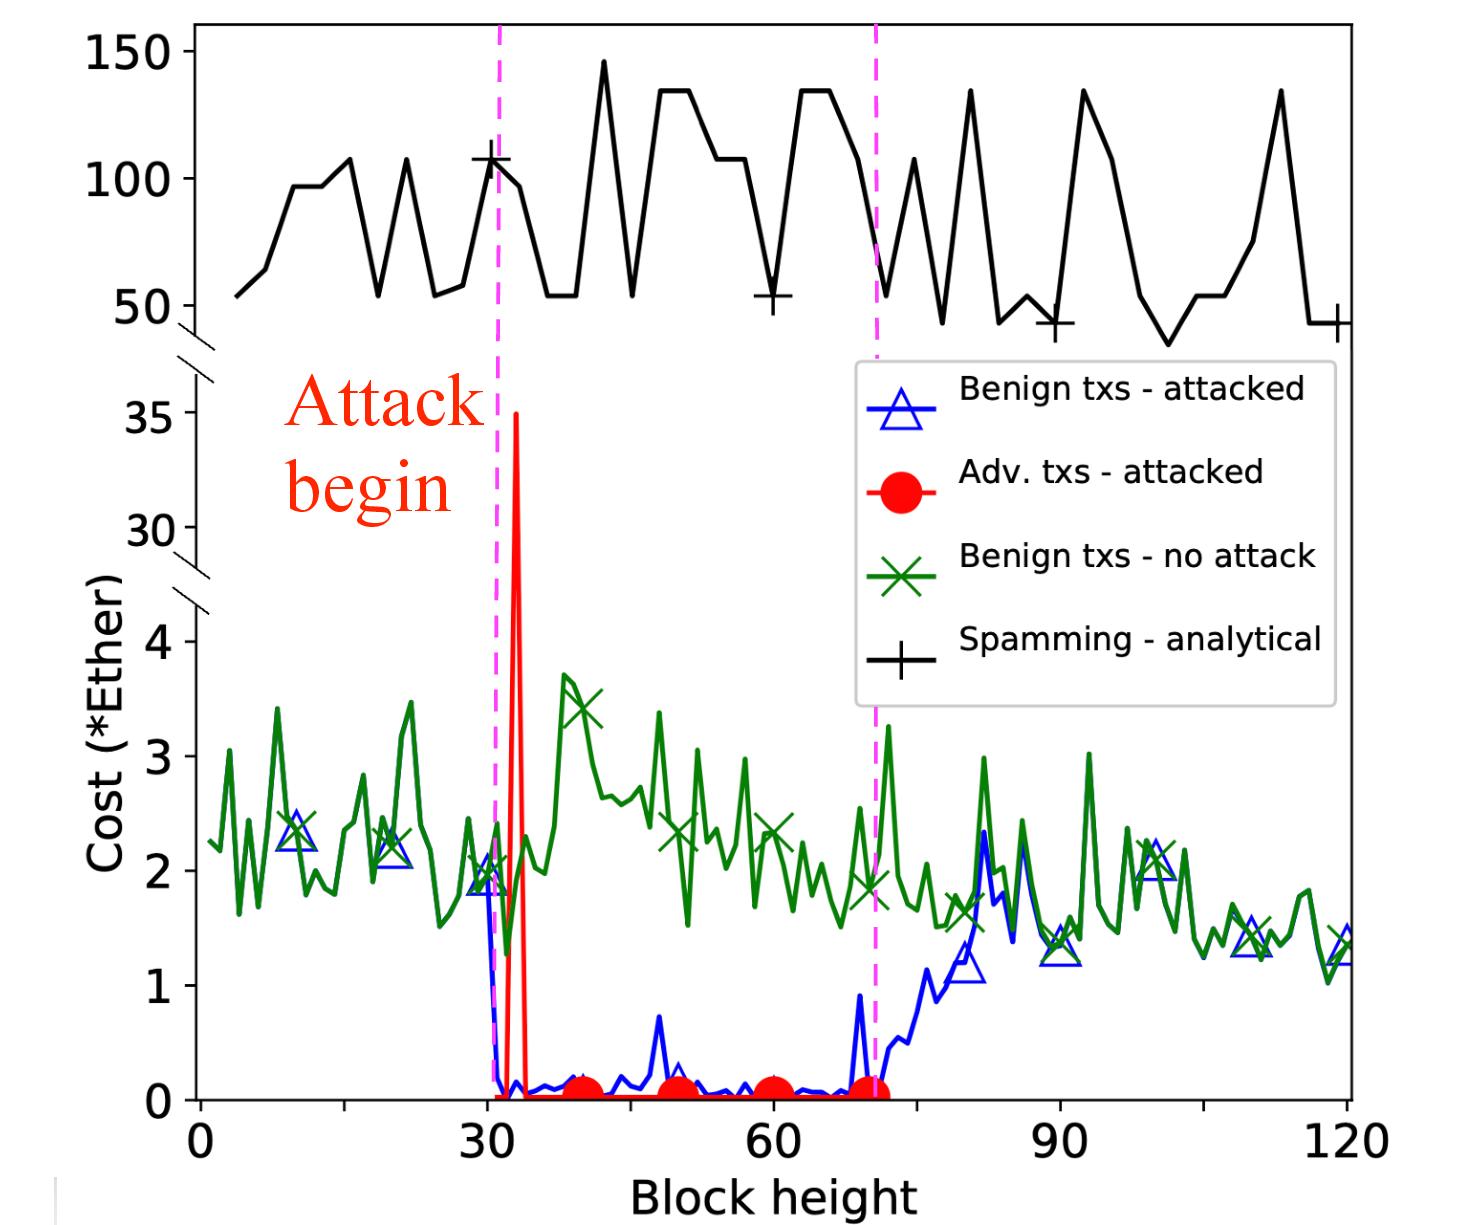}
    \label{fig:successrate-geth-propagate}}%
}
  \subfloat[$XT_6$ w. varying delay ($6$ nodes)] {%
   \includegraphics[width=0.245\textwidth]{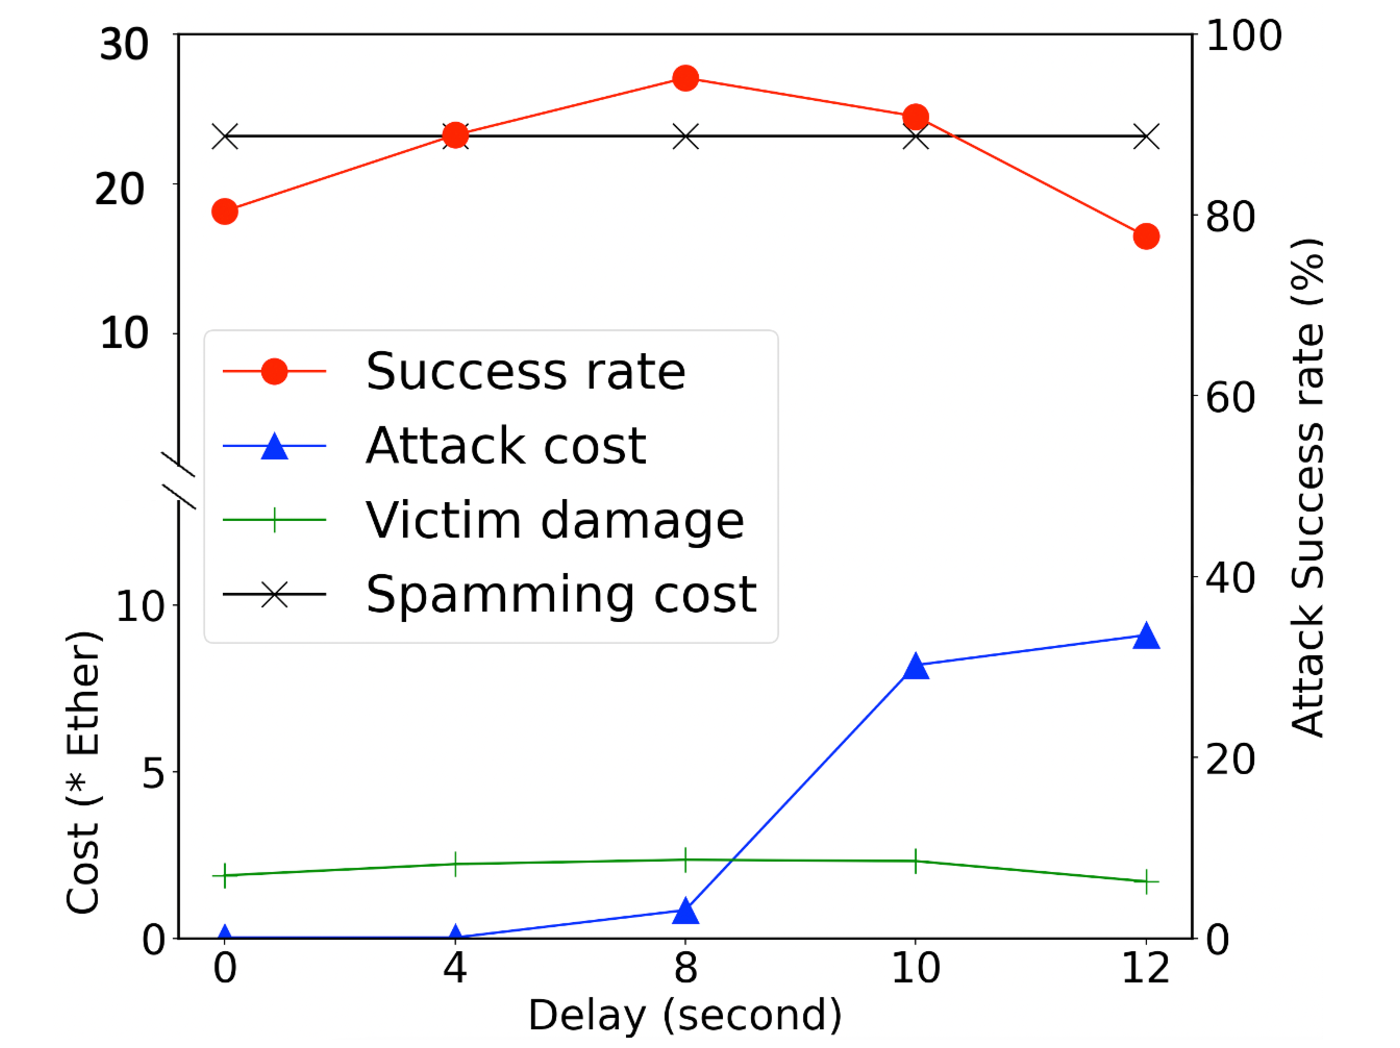}
  \label{fig:delay-geth-propagate}
  \label{fig:turning:multi}
}
\hfill
\bigskip
  \subfloat[$XT_4$ on Geth w. varying delay\\\hspace{\textwidth} (single node)]{%
    \includegraphics[width=0.24\textwidth]{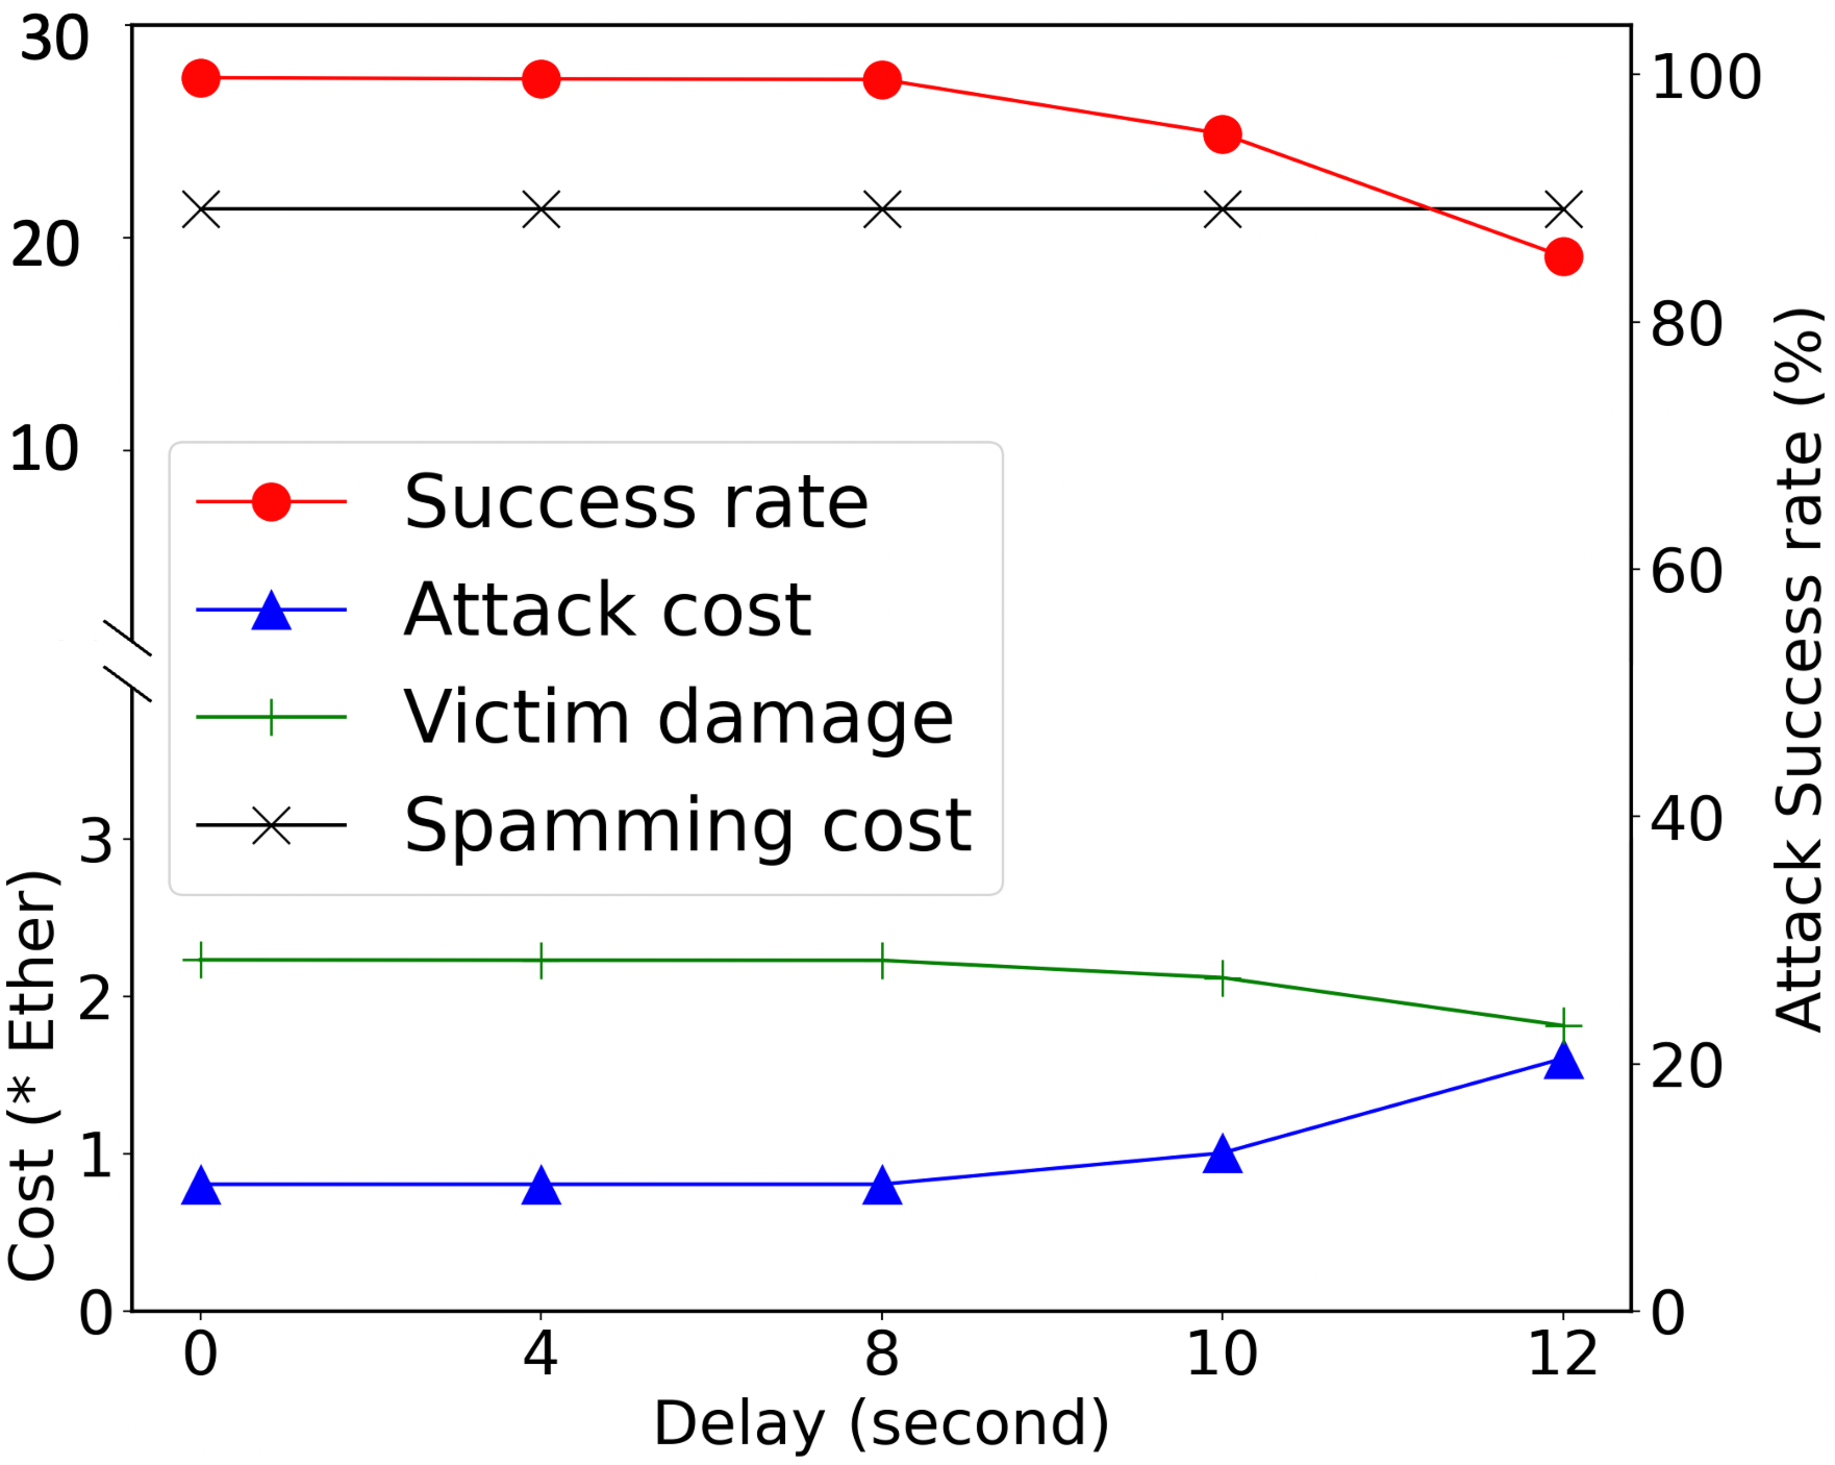}
    \label{fig:trade-off-xt4-geth}}%
  \subfloat[$XT_4$ on Erigon w. varying delay \\\hspace{\textwidth}(single node)] {%
   \includegraphics[width=0.24\textwidth]{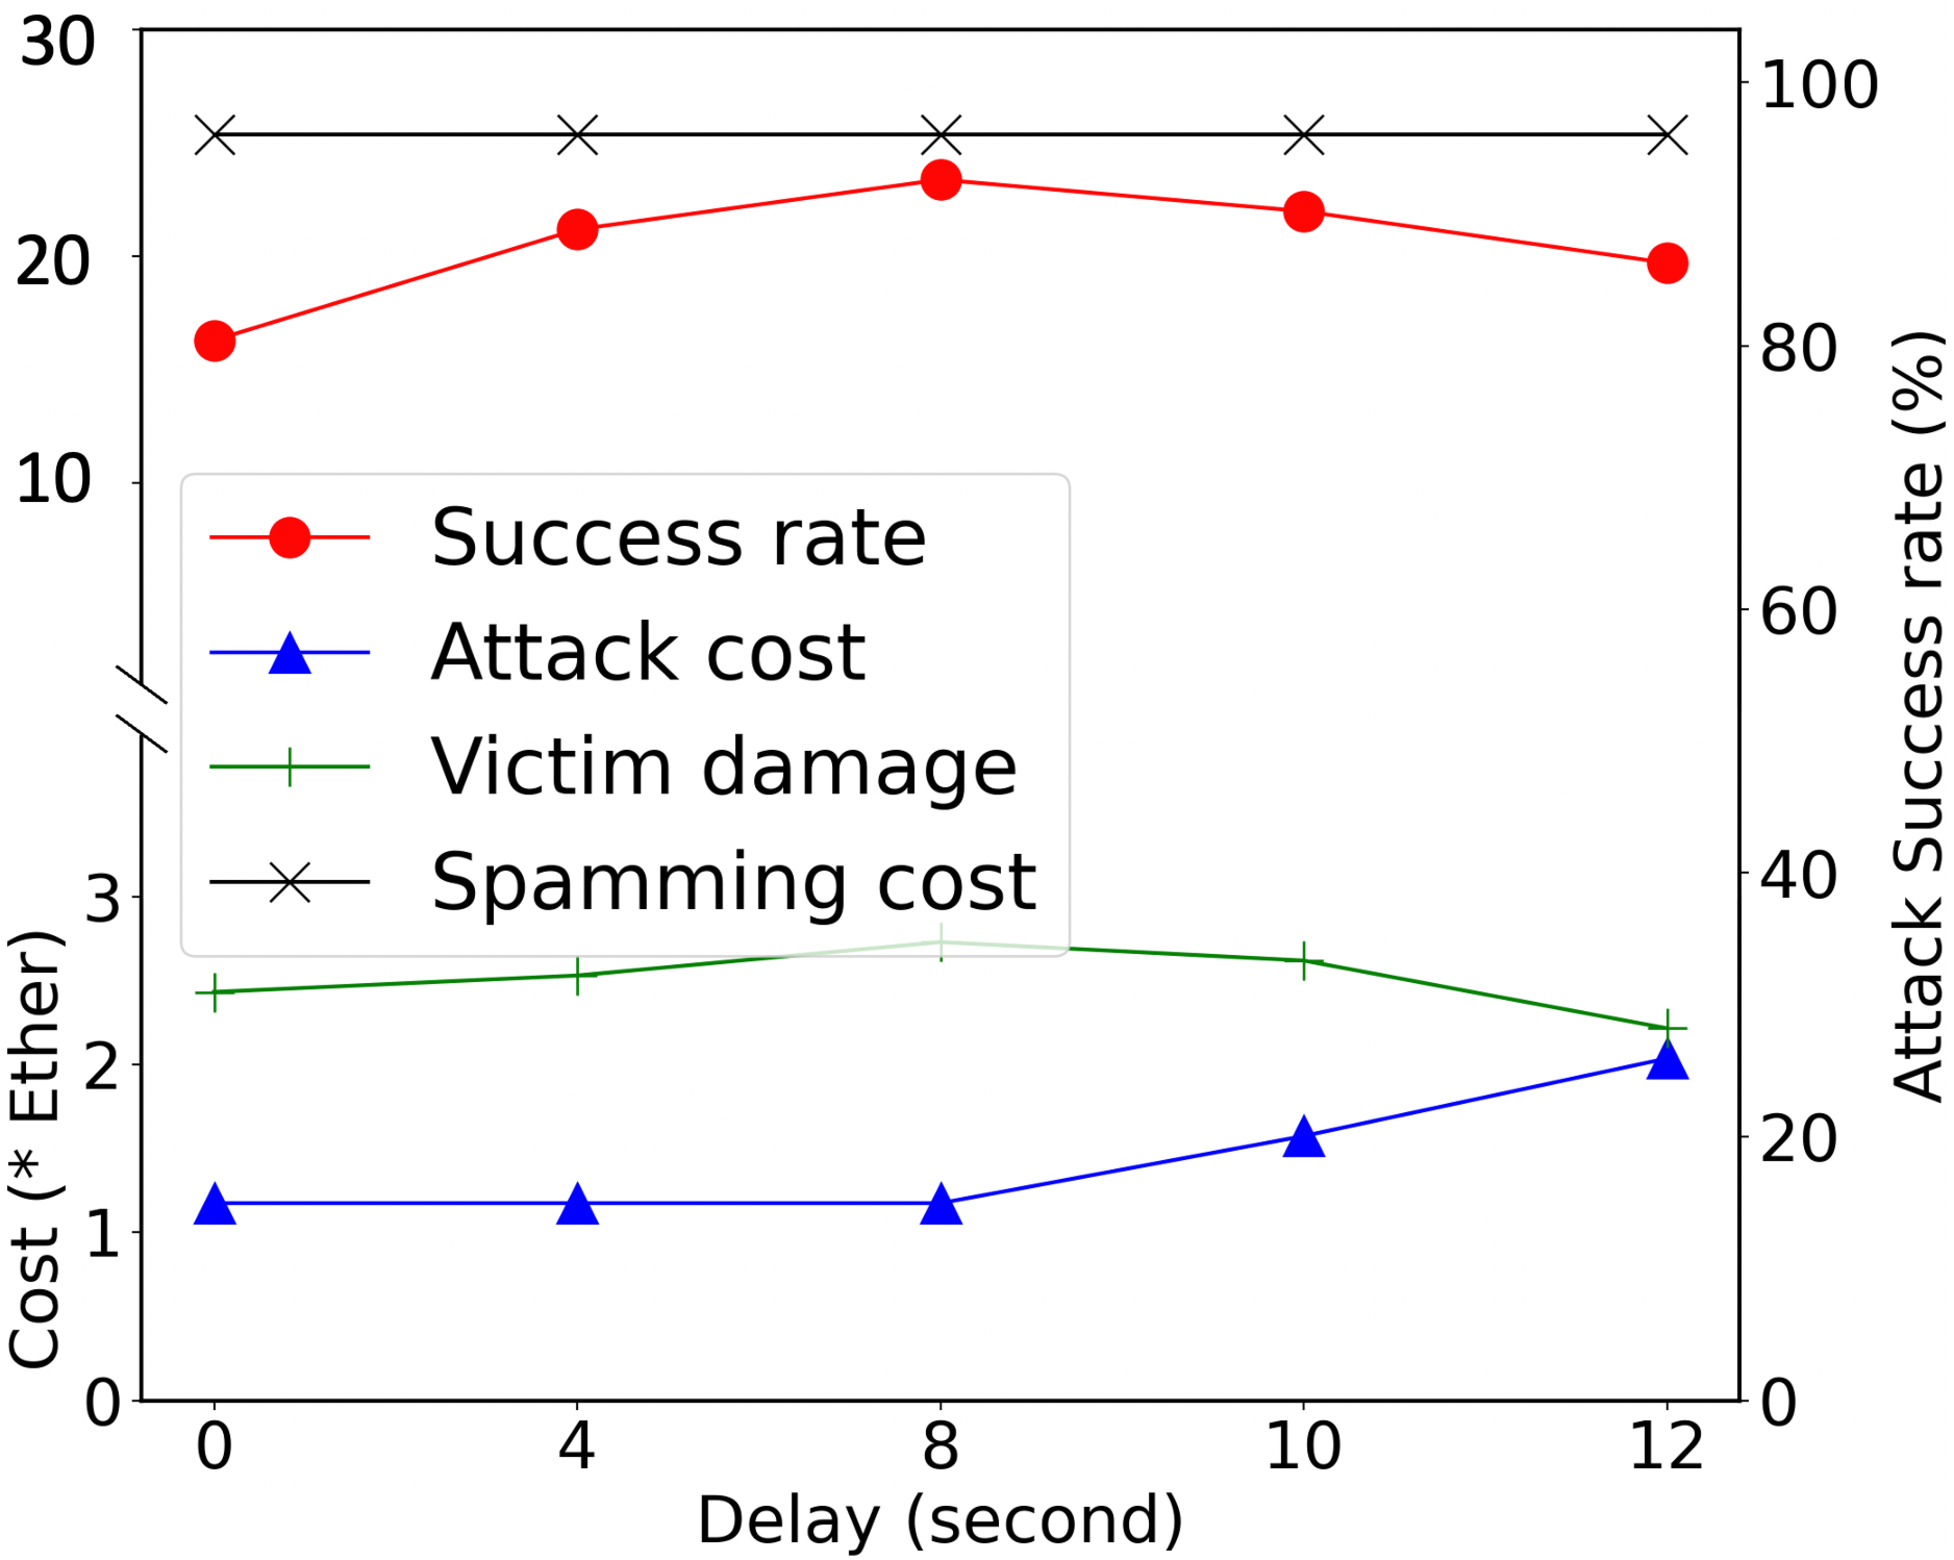}
  \label{fig:trade-off-xt4-erigon}}
  \subfloat[$XT_{8a}$ on Reth w. varying delay\\\hspace{\textwidth} (single node)] {%
   \includegraphics[width=0.24\textwidth]{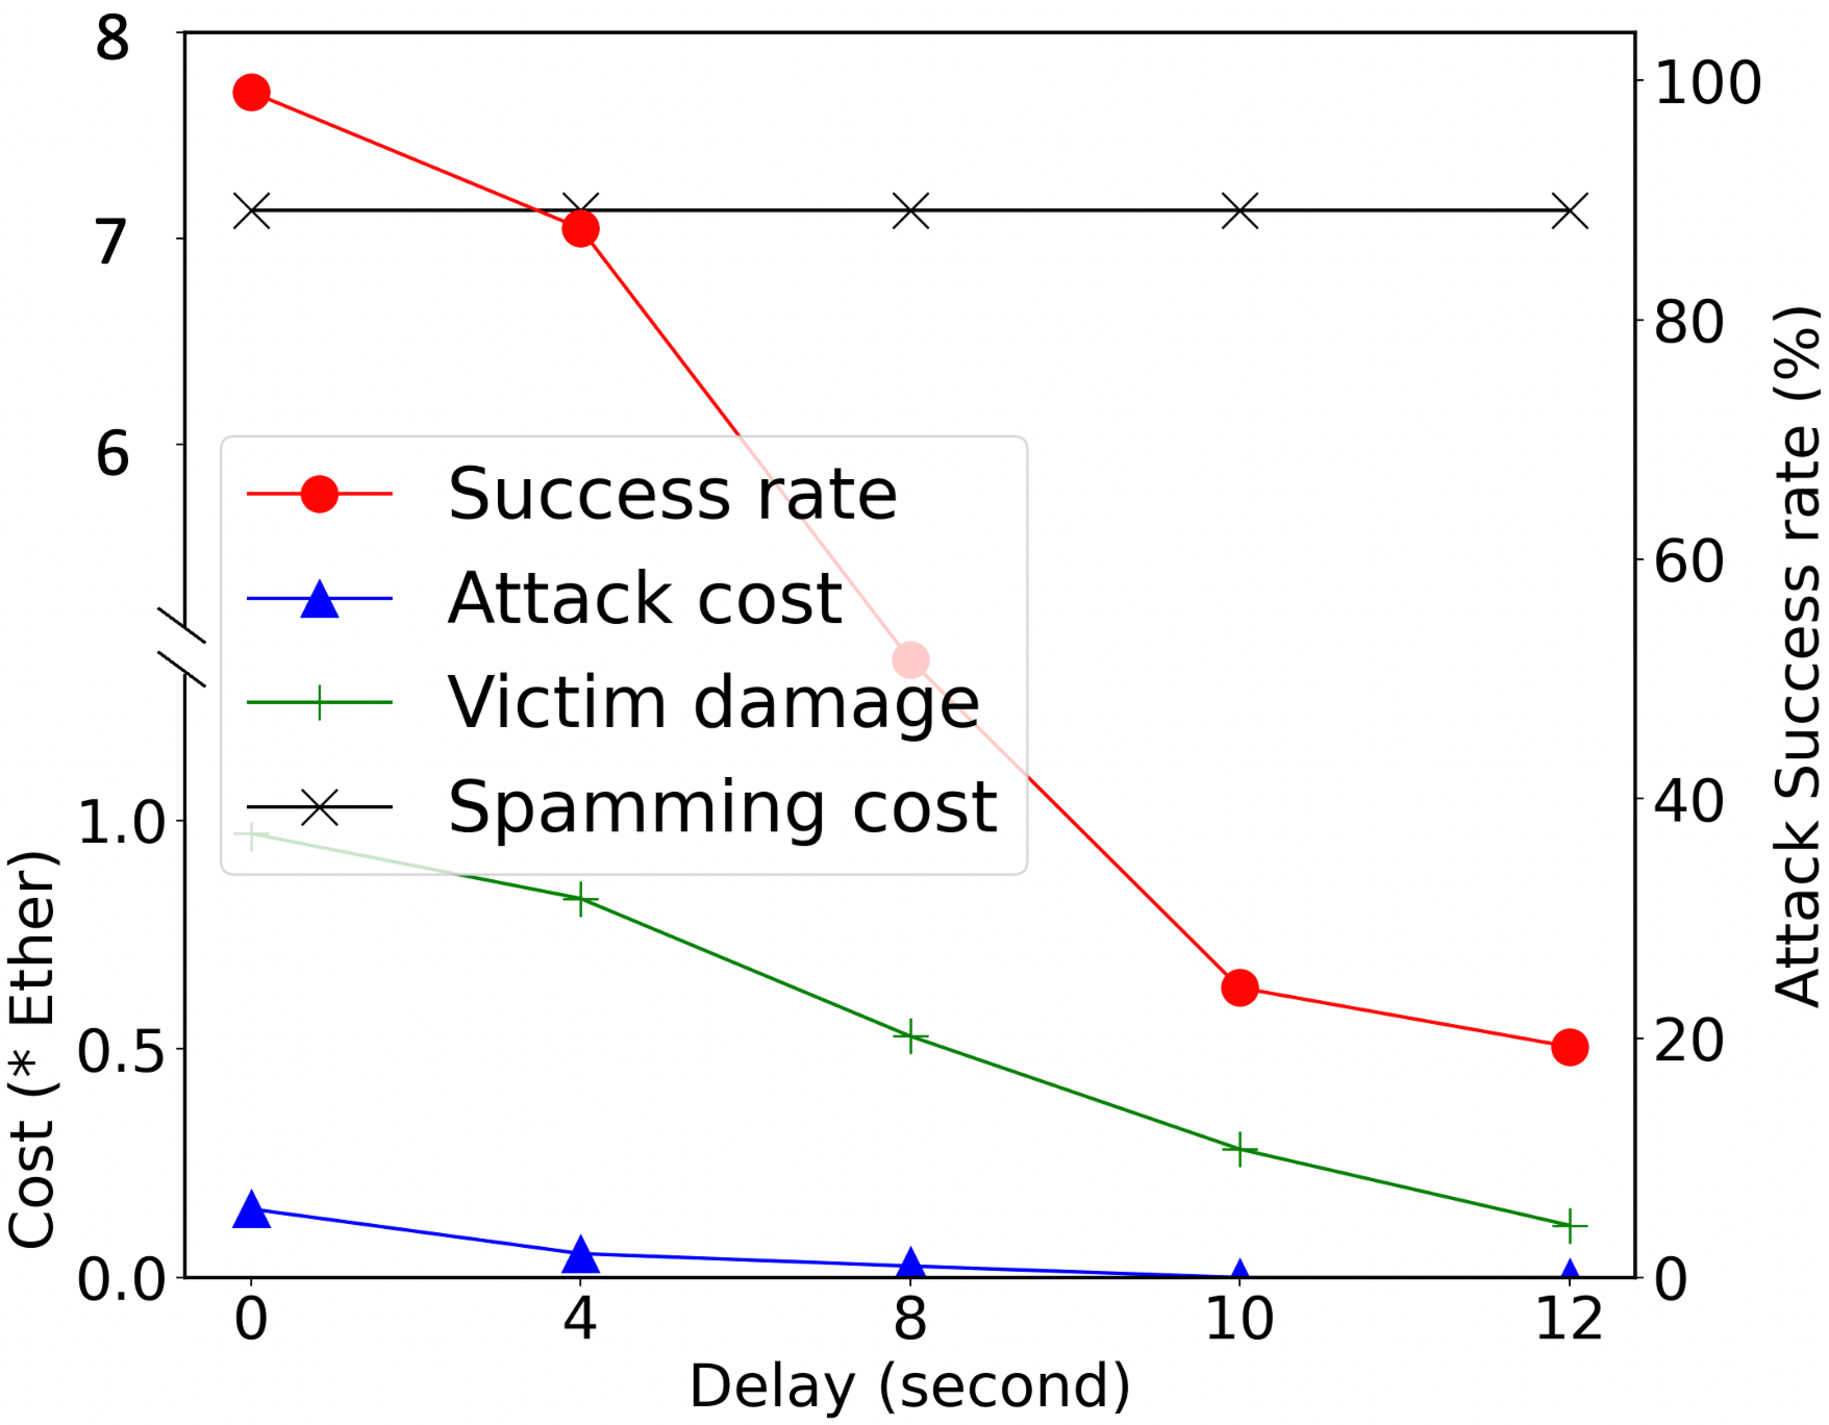}
  \label{fig:trade-off-xt8}}
  \subfloat[$XT_9$ on openEthereum w. varying \\\hspace{\textwidth}delay (single node)] {%
   \includegraphics[width=0.24\textwidth]{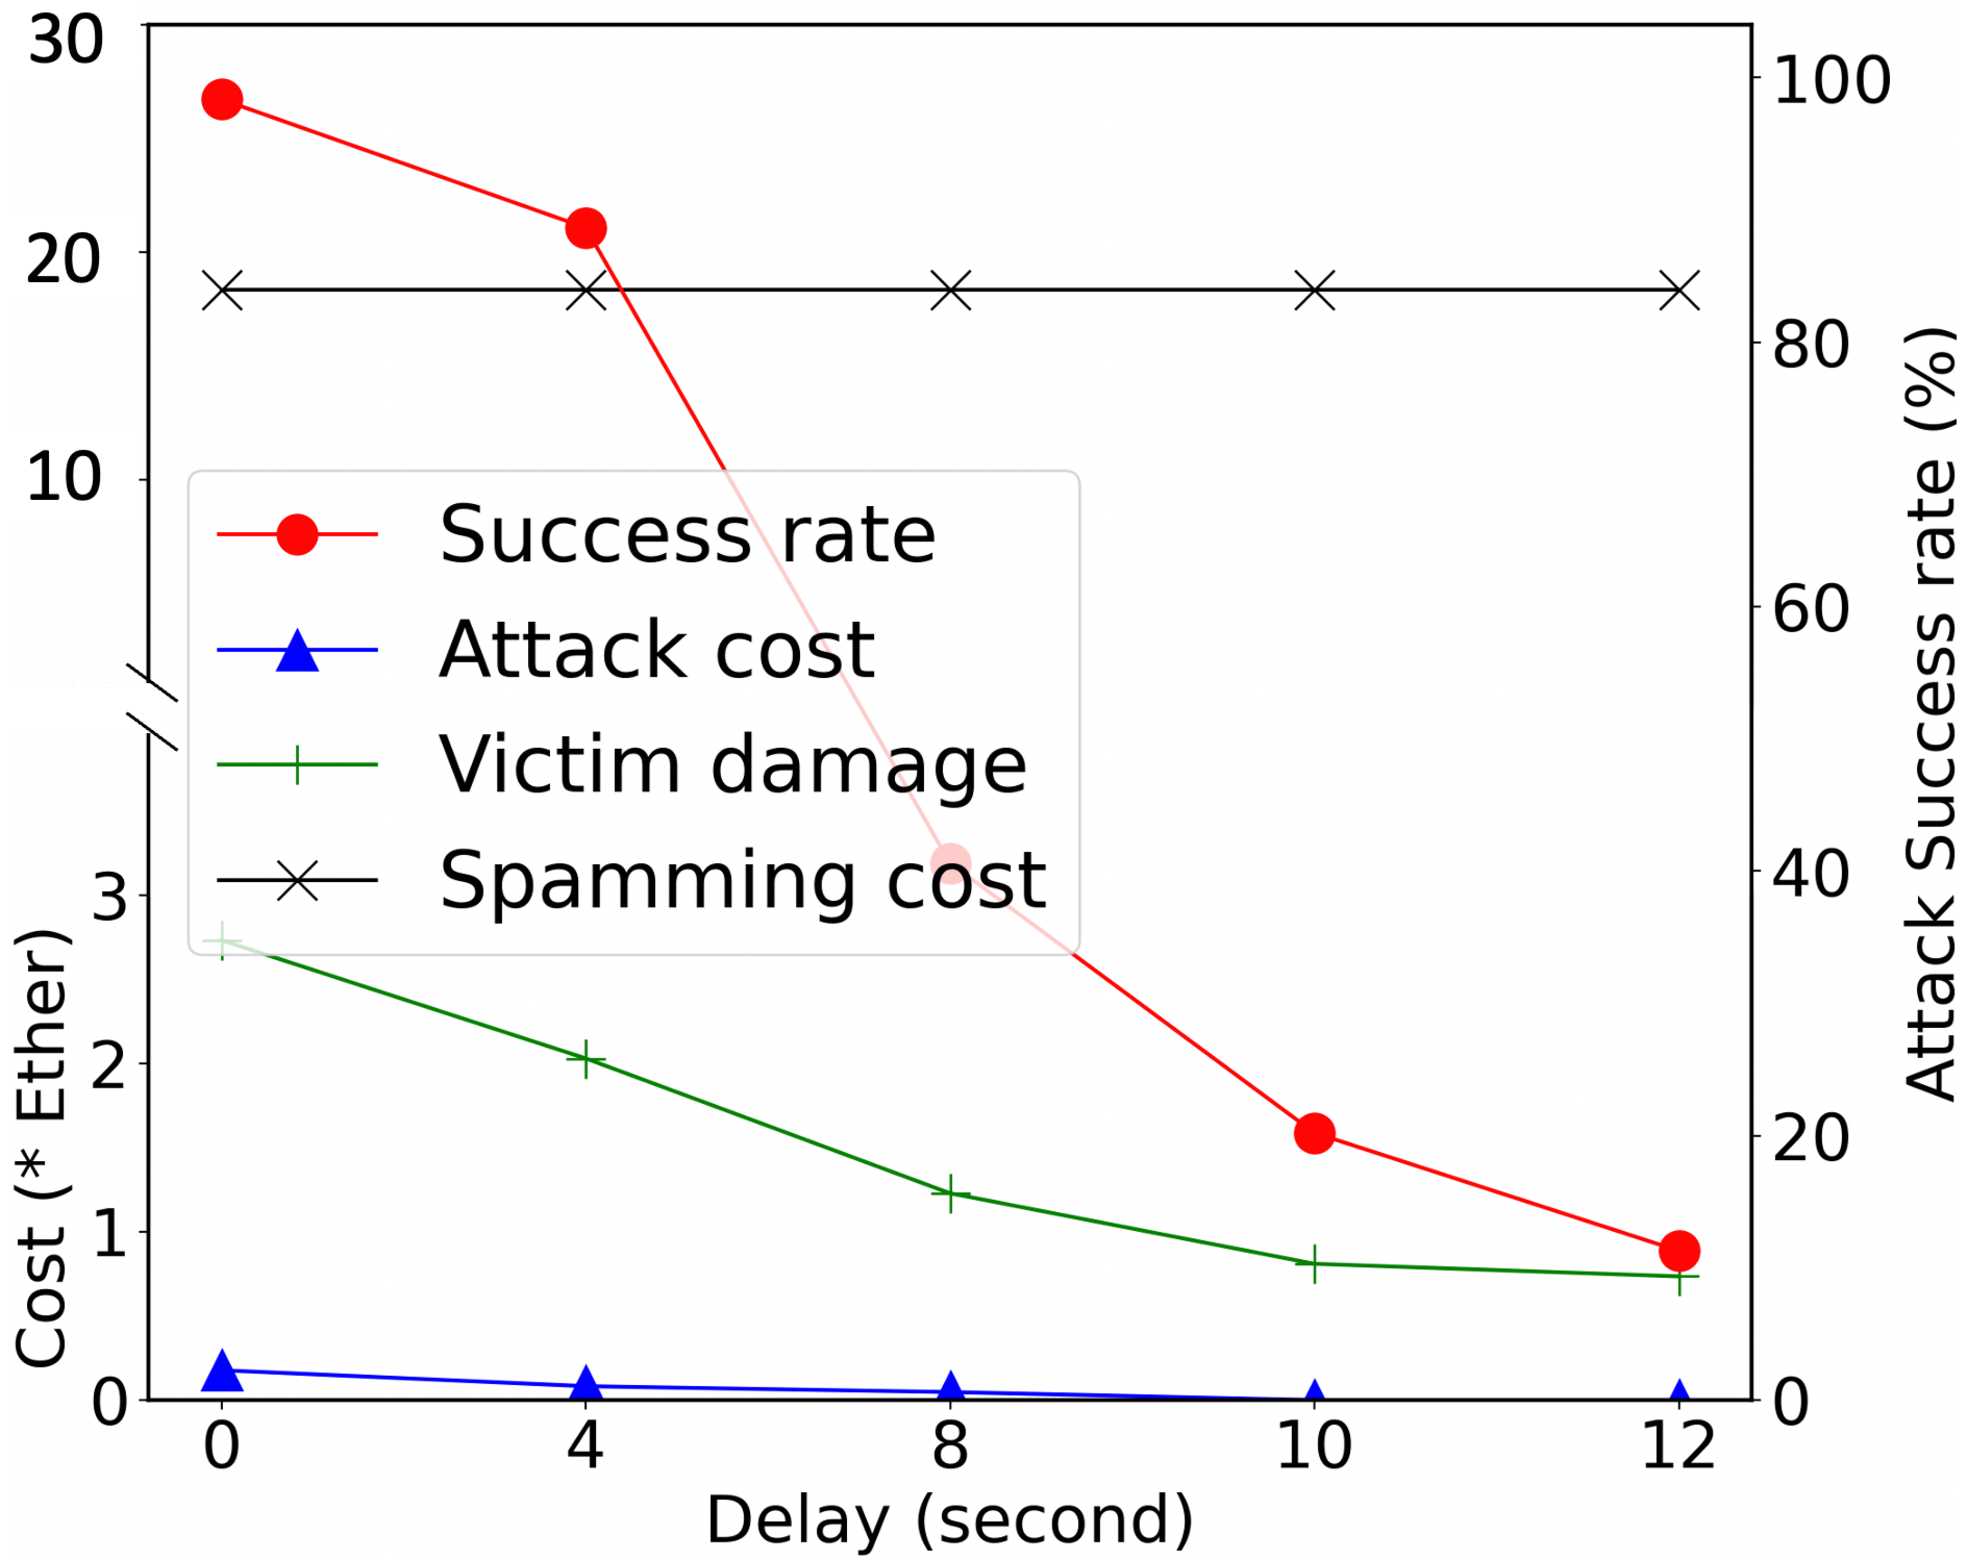}
  \label{fig:trade-off-xt9}
  
}
  \caption{Success rate and cost of turning-based eviction attack and locking attack.}%
\end{figure*}
\ignore{
Figure~\ref{fig:successrate-nethermind} reports the metrics for $XT_4$ on a victim node running Nethermind. Before the attack is launched (i.e., before the $30$-th block), the two experiment runs (attacked and no attack) produce the blocks of the same benign transaction fees, i.e., around $2-3$ Ether per block. As soon as the attack starts from the $30$-th block, the benign transaction fees quickly drop to zero Ether. The adversarial transaction fees show up and remain close to zero Ether per block. After the attack stops on $70$-th block, the benign transactions under attack gradually recover to the level of transactions under no attack. This process shows $XT_4$ with a 0-second delay has a high $100\%$ success rate, being able to evict all benign transactions in the mempool compared to the case of no attack. The $100\%$ success rate is due to that $XT_4$ is able to lock the mempool, and with $0$-second delay, the chance the transaction sequence of $XT_4$ is cut off by a block is minimal. It also shows the attack cost of $XT_4$ is extremely low, with almost zero Ether per block. The cost of spamming attack~\cite{DBLP:conf/fc/BaqerHMW16} is as high as $50$ Ether per block.

Figure~\ref{fig:successrate-geth} reports the same metrics for launching exploit $XT_6$ with $8$-second delay on a victim node running Geth-$V1.11.4$. The results are similar to those in Figure~\ref{fig:successrate-nethermind} except for the following: Instead of strictly zero-Ether fees, the adversarial-transaction fees of $XT_6$ are mostly zero Ether but also with sporadic spikes of non-zero fees under $1$ Ether. Because $XT_6$ does not lock the mempool, chances are the benign transactions sent $8$ seconds after a block is produced can be admitted into the mempool and included in the next block.
}

Figure~\ref{fig:successrate-geth} reports the metrics for $XT_6$ on a victim node running Geth $v1.11.4$. Before the attack is launched (i.e., before the $30$-th block), the two experiment runs (attacked and no attack) produce the blocks of the same benign transaction fees, i.e., around $2-3$ Ether per block. As soon as the attack starts from the $30$-th block, the benign transaction fees quickly drop to zero Ether except for some sporadic spikes (under $1$ Ether per block). The non-zero Ether cost is due to that $XT_6$ cannot lock the mempool. The adversarial transaction fees show up and remain close to zero Ether per block. After the attack stops on $70$-th block, the benign transactions under attack gradually recover to the level of transactions under no attack. 

\ignore{
Figure~\ref{fig:successrate-nethermind} reports the metrics for $XT_4$ on a victim node running Nethermind. Before the attack is launched (i.e., before the $30$-th block), the two experiment runs (attacked and no attack) produce the blocks of the same benign transaction fees, i.e., around $2-3$ Ether per block. As soon as the attack starts from the $30$-th block, the benign transaction fees quickly drop to zero Ether. The adversarial transaction fees show up and remain close to zero Ether per block. After the attack stops on $70$-th block, the benign transactions under attack gradually recover to the level of transactions under no attack. This process shows $XT_4$ with a 0-second delay has a high $100\%$ success rate, being able to evict all benign transactions in the mempool compared to the case of no attack. The $100\%$ success rate is due to that $XT_4$ is able to lock the mempool, and with $0$-second delay, the chance the transaction sequence of $XT_4$ is cut off by a block is minimal. It also shows the attack cost of $XT_4$ is extremely low, with almost zero Ether per block. The cost of a baseline spamming attack is very high, about $20$ Ether per block.
}

We also conduct experiments with varying attack delays between $0$ seconds and $12$ seconds (note that the average time to produce a block in our collected trace is $14$ seconds). Figure~\ref{fig:delay-nethermind} shows the results of Attack $XT_4$ on Nethermind. On shorter delay than $8$ seconds, the success rates are strictly $100\%$, and the attack cost remains at $0.025$ Ether per block. When the delay grows over $8$ seconds, success rates begin to drop, and attack costs increase. At the longest delay of $12$ seconds, the success rate is $80\%$, and the attack cost is $1.5$ Ether per block. 
The reason is that as the delay becomes large, the transaction sequence sent in an attack can be interrupted by block production, leading to adversarial transactions included in the blockchain and normal transactions un-evicted from the mempool.

\definecolor{blue-yibo}{rgb}{0.0, 0.0, 1.0}
{ The results of Attack $XT_4$ on Geth as shown in Figure~\ref{fig:trade-off-xt4-geth} are similar to those on Nethermind. The difference is the cost of $XT_4$ on Geth is higher than that of Nethermind. In the attack sequence of $XT_4$ on Geth, it needs $384$ attack senders which means $384$ attack transactions are included in blocks on shorter delay than $8$ seconds while only $1$ attack transaction is included in $XT_4$ on Nethermind.  
}

Figure~\ref{fig:delay-geth} shows the success rates and costs of Exploit $XT_6$ on Geth $v1.11.4$. The results are similar to those in Figure~\ref{fig:delay-nethermind} except that when the delay is short, the success rates of $XT_6$ are not $100\%$ because $XT_6$ cannot lock the attacked mempool and an attack sent too early risks admitting normal transactions sent after the attack. 

{ The results of Attack $XT_4$ on Erigon are shown in Figure~\ref{fig:trade-off-xt4-erigon}. The results are similar to those in Figure~\ref{fig:delay-geth} as the $XT_4$ on Erigon also cannot lock the attacked mempool when the delay is short. 
%However, the attack cost is $1.17$ ETH which is higher than that of Geth and Nethermind on a shorter delay than $8$ seconds. The reason is more attack senders (i.e., $625$ senders) are required in the attack sequence of $XT_4$ on Erigon and more attack transactions are included in blocks.

Figure~\ref{fig:trade-off-xt8} shows the success rates and cost of $XT_8$ on Reth. When the delay is $0$ second, the success rate is $99.04\%$, and the cost is $0.151$ Ether per block. The low-priced attack transactions sent with a $0$ delay occupy all the empty slots and decline all the incoming normal transactions. When the delay grows, the success rate and attack cost begin to drop. The reason is as the delay increases, more empty slots in the mempool are occupied by normal transactions. As a result, more normal transactions and less attack transactions are included in blocks.

The results of Attack $XT_9$ on OpenEthereum are shown in Figure~\ref{fig:trade-off-xt9}. The results are similar to those of $XT_8$ on Reth except when the delay is short, the cost of $XT_9$ on OpenEthereum is $0.177$ per block which is higher than that of Reth. The reason is that each attack sender in the $XT_9$ attack sequence sends a high-priced child transaction for declining the incoming normal transactions and the high-priced transactions are included in blocks.   
}

{  
The evaluation results of all attacks on all clients are in Table~\ref{tab:attack-success-rate-cost}. On the six Ethereum clients in the public transaction path, the attack success rates are all higher than $84.63\%$, and the attack costs are all lower than $1.172$ Ether per block, which is significantly lower than the baseline.
}

{  
On PBS clients and Ethereum-like clients, we also evaluate the attacks found by \textsc{mpfuzz}. Under the same experimental settings as \S~\ref{sec:setup:singlenode}, the results show similar success rates and costs with the attacks on Geth (recall these clients are Geth forks). More specifically, Table~\ref{tab:attack-success-rate-cost} shows that the success rates are higher than $92.60\%$, and attack costs are lower than $0.806$ Ether per block.
}

\begin{table}[!htbp]
\caption{Attack success rate and cost}
\label{tab:attack-success-rate-cost}
\centering{\footnotesize
\begin{tabularx}{0.495\textwidth}{ |X|l|X|X|X| }
\hline
%Exploit-rate (\#/sec.)
Clients & Exploit& Success rate & Cost (Ether/block) & Baseline (Ether/block) \\ \hline
Geth & $XT_1$ & $99.80\%$& $0$ & $11.39$ \\  \cline{2-5}
$v1.10.25$& $XT_2$ & $99.42\%$& $0.725$ & $11.39$ \\  \cline{2-5}
& $XT_3$ & $93.02\%$& $0.0021$ & $11.39$\\  \hline
Geth & $XT_4$ & $99.42\%$& $0.806$ & $11.39$ \\  \cline{2-5}
$v1.11.4$& $XT_5$ & $92.65\%$ &$0.806$ & $11.39$ \\  \cline{2-5}
& $XT_6$ & $94.74\%$& $0.0022$ & $11.39$ \\  \hline
Erigon $v2.42.0$ & $XT_4$ & $92.53\%$& $1.172$ & $17.7$ \\  \hline
Nethermind & $XT_4$ & $99.60\%$& $0.0021$ & $10.75$ \\ \cline{2-5}
$v1.18.0$ & $XT_7$ & $84.63\%$& $0.20$ & $10.75$ \\  \hline
Besu  & $XT_2$ & $99.63\%$& $1.04$ & $17.7$\\  \cline{2-5}
$v22.7.4$ & $XT_4$ & $99.60\%$& $1.06$ & $17.7$\\  \hline
Reth $v0.1.0\-alpha.6$& $XT_4$ &$92.53\%$ &$0.672$ & $17.6$ \\  \hline
Flashbot builder $v1.11.5$& $XT_6$ & $94.74\%$& $0.0022$ & $11.39$ \\  \hline
EigenPhi & $XT_1$ & $99.80\%$& $0$ & $11.39$ \\  \cline{2-5}
builder& $XT_2$ & $99.42\%$& $0.725$ & $11.39$ \\  \cline{2-5}
 & $XT_3$ & $93.02\%$& $0.0021$ & $11.39$ \\  \cline{2-5}
& $XT_4$ & $99.42\%$& $0.806$ & $11.39$ \\  \cline{2-5}
& $XT_6$ & $94.74\%$& $0.0022$ & $11.39$ \\   \hline
bloXroute builder-ws& $XT_6$ & $94.74\%$& $0.0022$ & $11.39$ \\  \hline
go-opera & $XT_2$ & $99.12\%$& $0.201$ & $11.39$ \\  \cline{2-5}
$v1.1.3$& $XT_3$ & $92.60\%$& $0.0021$ & $11.39$ \\  \cline{2-5}
& $XT_4$ & $99.13\%$& $0.221$ & $11.39$ \\  \cline{2-5}
& $XT_6$ & $93.76\%$& $0.0022$ & $11.39$ \\  \hline
BSC $v1.3.8$& $XT_6$ & $94.74\%$& $0.0022$ & $11.39$ \\  \hline
core-geth $v1.12.18$ & $XT_6$ & $94.74\%$& $0.0022$ & $11.39$ \\  \hline
Reth $v0.1.0\-alpha.4$& $XT_8$ & $99.04\%$ &$0.151$ & $7.14$ \\  \hline
OpenEthereum & $XT_4$ &$99.56\%$ &$0.233$ & $11.39$\\  \cline{2-5}
$v3.3.5$ & $XT_9$ & $98.36\%$& $0.177$ & $18.35$\\ \hline
\end{tabularx}
}
\end{table}

\subsection{Experiments on Multi Nodes}

\label{appdx:sec:eval:local:2}
\noindent{\bf Evaluation settings}:
We extend our experiment platform to support a network of victim nodes, instead of a single victim node. Specifically, the attack node is connected to the first victim non-validator node $V_1$. Node $V_1$ is connected to the second victim non-validator node $V_2$, which is further connected to node $V_3$. The chain of victims continues until it reaches the $6$-th non-validator victim $V_6$, which is connected to the validator victim node $V_0$. The workload node is connected to the validator node $V_0$. We run the victim network among a set of geo-distributed cloud instances on the Internet. We place victim nodes $V_1, V_3, V_5$ in one geographic area in Amazon AWS cloud (a.k.a., one Availability Zone or AZ). We place the other victim nodes $V_2, V_4, V_6, V_0$ in a different geographic area, so that each message sent between $V_i$ and $V_{i+1}$ has to travel across continents on the Internet. The experiment architecture is illustrated in Figure~\ref{fig:exp:setup}.

\noindent{\bf Experiment results}:
On the multi-victim platform, we conduct similar experiments as in \S~\ref{sec:setup:singlenode}. The results are presented in Figure~\ref{fig:turning:multi}. Compared with the results on the single node, the attack cost increases faster and is much higher. For instance, when the delay is $10$/$12$ seconds, the attack cost is $8$/$8.5$ Ether per block, which is higher than the attack damage (i.e., the victim transaction fees). Under the delay, the attacks incur higher attack cost than damage and are no longer ADAMS. By contrast, from Figure~\ref{fig:delay-geth}, the attack costs on the single node with $10$/$12$-second delays are $1$/$1.4$ Ether per block, both of which are below the attack damage. The cause of the higher attack cost is the longer time to propagate the transaction sequence of an ADAMS attack in the multi-node setting than in the single node; the longer time implies the higher chance the transaction sequence is interrupted by the production of the next block and that the transactions are included to the block without being turned invalid.

\subsection{Additional Evaluation Results on Single Node}
\label{appdx:singlenode}

We present more evaluation results of different found exploits across Erigon and Nethermind as shown in Figure~\ref{fig:erigon-local}, Figure~\ref{fig:nethermind-td} and Figure~\ref{fig:nethermind-ed}. The evaluations are conducted on a single node.

\begin{figure}[!ht]
  \centering
  \subfloat[Attack damage]{%
  \includegraphics[width=0.25\textwidth]{figures/rate-erigon-local.eps}
  \label{fig:rate-erigon-local}
    }%
    \subfloat[Attack cost]{%
  \includegraphics[width=0.25\textwidth]{figures/cost-erigon-local.eps}
  \label{fig:cost-erigon-local}}
  \caption{Exploit $XT_4$ (Erigon)}%
  \label{fig:erigon-local}
\end{figure}

\begin{figure}[!ht]
  \centering
  \subfloat[Attack damage]{%
  \includegraphics[width=0.25\textwidth]{figures/rate-nethermind-local1.eps}
  \label{fig:rate-nethermind-local1}
    }%
    \subfloat[Attack cost]{%
  \includegraphics[width=0.25\textwidth]{figures/cost-nethermind-local1.eps}
  \label{fig:cost-nethermind-local1}}
  \caption{Exploit $XT_4$ (Nethermind)}%
  \label{fig:nethermind-td}
\end{figure}

\begin{figure}[!ht]
  \centering
  \subfloat[Attack damage]{%
  \includegraphics[width=0.25\textwidth]{figures/rate-nethermind-EDlocal.eps}
  \label{fig:rate-nethermind-ed}
    }%
    \subfloat[Attack cost]{%
  \includegraphics[width=0.25\textwidth]{figures/cost-nethermind-ED.eps}
  \label{fig:cost-nethermind-ed}}
  \caption{Exploit $XT_7$ (Nethermind)}%
  \label{fig:nethermind-ed}
\end{figure}

\subsection{Additional Evaluation of Locking on Reth}
\label{appdx:sec:eval:locking2}

\begin{figure}
  \centering
  \includegraphics[width=0.375\textwidth]{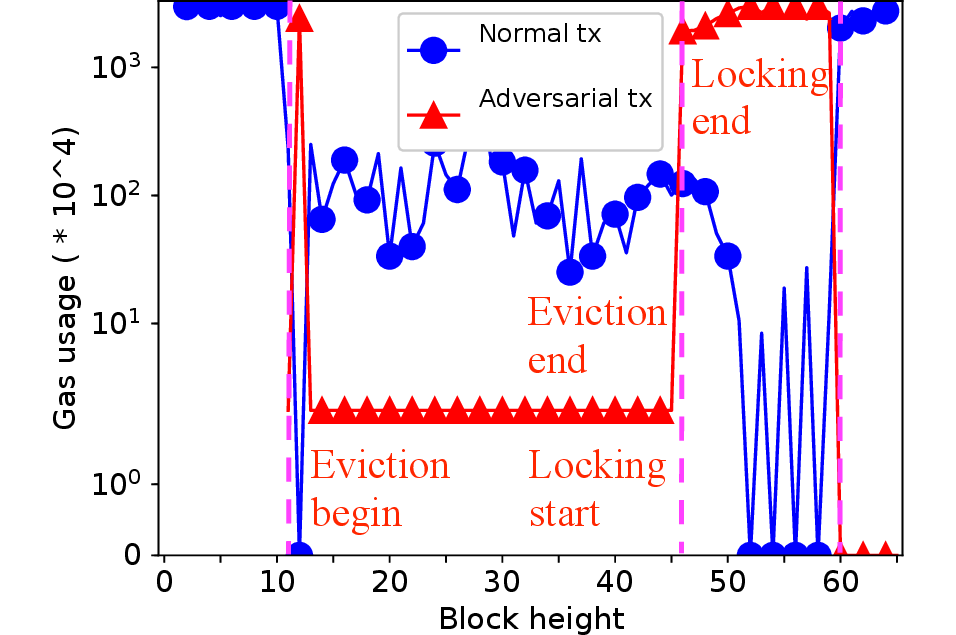}
  \caption{Gas usage of attacks $XT_{8a}$}
  \label{fig:reth-gas}
\end{figure}
Figure~\ref{fig:reth-gas} shows the Gas usage of attack transactions and normal transactions in $XT_{8a}$. During the locking attack from block height $45$-th to $60$-th, the attacker sends locking transactions to occupy all the empty slots. It makes the Gas usage of the attacker almost 100\% block limit while the Gas usage of the normal transactions drops to around $0$. When empty slots are created by arriving blocks, normal transactions compete with the attack transactions to admit into the empty slots. Thus, some normal transactions are included in blocks during the locking attack.

\subsection{Additional Evaluation of Locking Attacks}
\label{appdx:sec:eval:locking}

\subsubsection{Locking Attacks $XT_{8b}$ on Reth}

\noindent{\bf 
Exploit $XT_{8b}$}: We also manually designed another locking variant for Reth. Suppose the Reth node does not run block validation, and its mempool is initially synchronized with the mempool of a block validator. The attacker first evicts $10,000$ normal transactions from the validator's mempool. Then, the Reth node's mempool is permanently locked by the $10,000$ normal transactions evicted from the validator mempool. Because these 10,000 transactions will never be included in blocks, they would exist in the Reth node's mempool forever, permanently locking it in its current state.

\begin{figure}[!htb]
  \centering
  \includegraphics[clip,width=0.72\columnwidth]{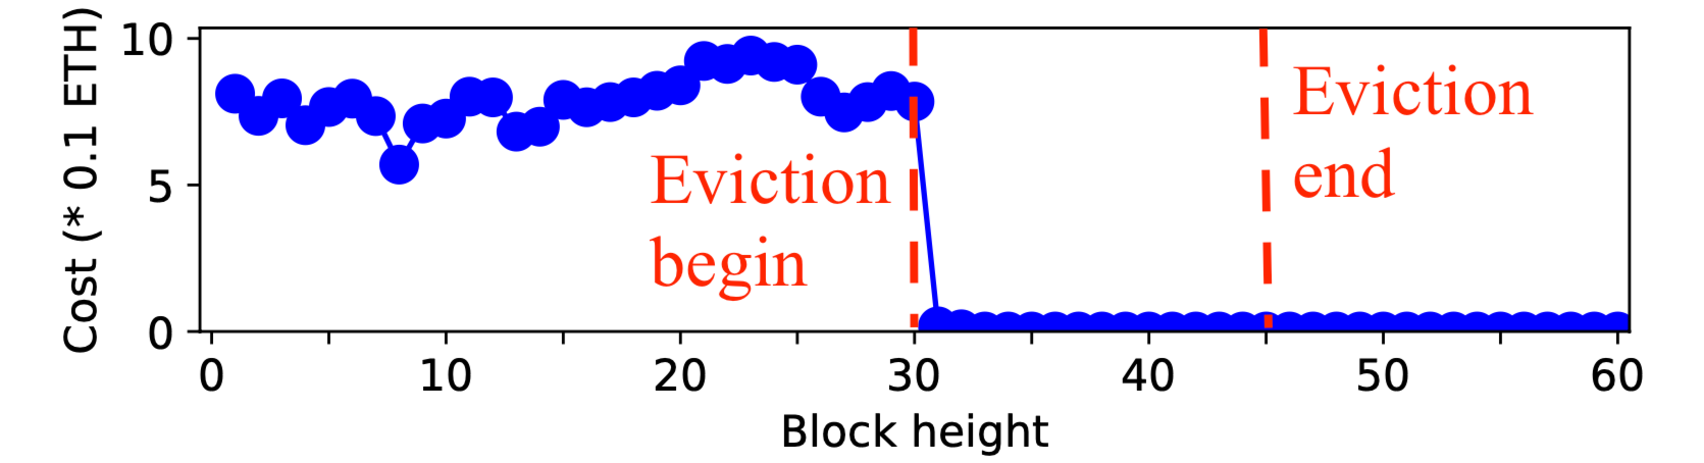}%
\caption{Evaluation of locking attack $XT_{8b}$ on Reth}%
\label{fig:side-effect-locking}
\end{figure}

\noindent{\bf 
Evaluation of $XT_{8b}$}: To evaluate $XT_{8b}$, we initially set up the attacker node connected to the validator node running Geth, the workload generator node connected to the victim non-validator Reth node, and the Reth node connected to the validator. The system is run long enough to produce a certain number of blocks and the normal transactions are propagated to both validator and on-validator nodes' mempools. We then mount the eviction attack ($XT_6$) directly to the validator Geth node that evicts the mempool transactions on the validator node and prevents them from being included in the blocks. 

By mounting eviction attacks between the $30$-th to $45$-th blocks in Figure~\ref{fig:side-effect-locking}, the Reth mempool is successfully locked afterward: From the figure, after the $45$-th block, the total fees of normal transactions included in blocks remain at zero Ether per block until the experiment ends on the $60$-th block.

\subsubsection{Additional Evaluation of Locking on Geth}

\begin{figure}[!bthp]
\centering
\includegraphics[width=0.375\textwidth]{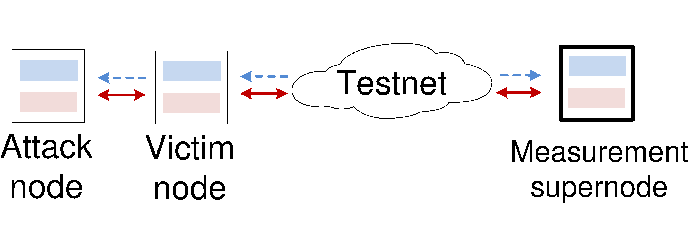}
\caption{Experimental setup for locking attacks on Geth/OpenEthereum}
\label{fig:exp:setup4}
\end{figure}

\ignore{
\begin{center}
\fbox{\parbox{0.90\linewidth}{RQ2. What's the success rate and attack cost in locking a remote mempool secured under turning attacks?
}}\end{center}
}

\begin{figure}[!ht]
 \centering
  \subfloat[Attack damage]{%
  \includegraphics[width=0.245\textwidth]{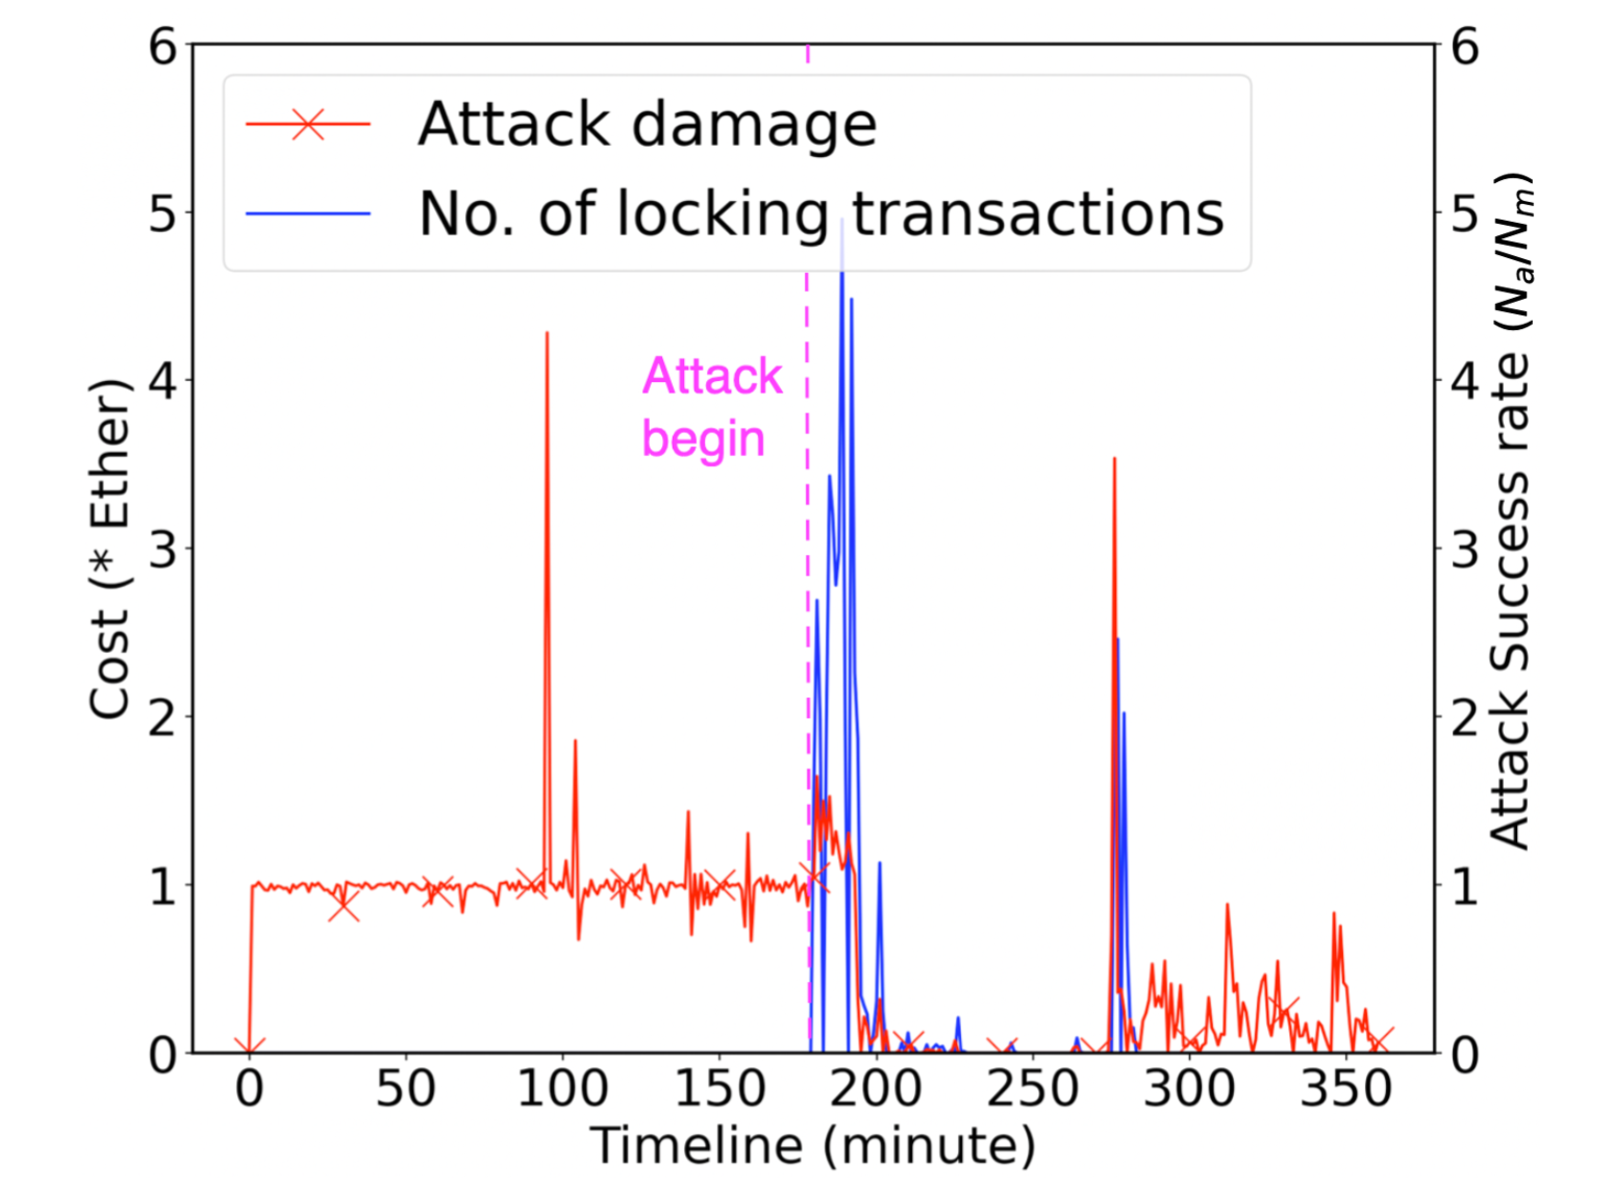}
 \label{fig:ld5:x}}
%  \subfloat[No. of locking transactions]{%2
% \includegraphics[width=0.295\textwidth]{figures/Kai-LD-figure2.eps}
% \label{fig:ld5:2}}
  \subfloat[Attack cost]{%
 \includegraphics[width=0.245\textwidth]{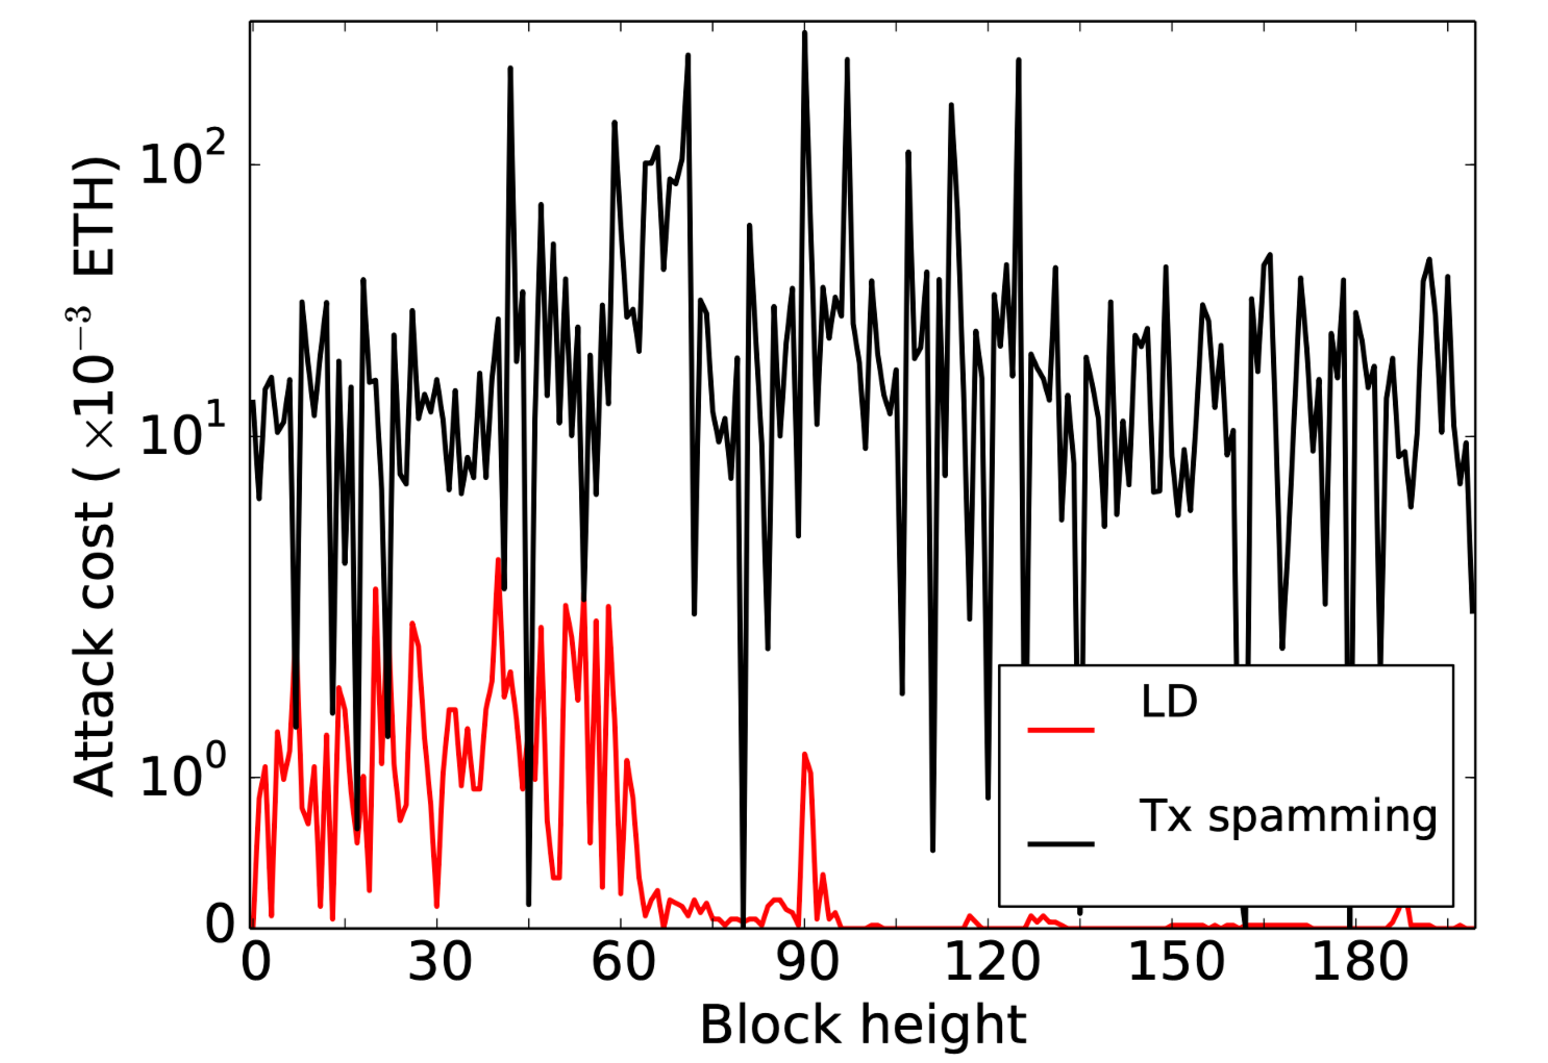}
 \label{fig:ld5:3}
  }%
 \caption{Mounting locking attacks on a Geth node in testnet.}
\end{figure}
\ignore{}

\noindent{\bf 
Design rational}: Recall that OpenEthereum adopts an overly strict policy that determines eviction by only considering the fees of childless transactions. While this policy is intended to prevent turning attacks ($XT_5$), it is vulnerable to locking attacks. Because OpenEthereum has been deprecated from the operational Ethereum 2.0 networks, we re-implement its admission policy on Geth $v1.11.4$ and run the turning-hardened Geth on a victim under locking attacks.

\noindent{\bf Settings}: 
We set up an experimental platform for evaluating locking attacks. The victim node runs the turning-hardened Geth client (based on $v1.11.4$) described above. The attacker node runs an instrumented Geth client (based on $v1.11.4$) at the execution layer such that it can mount locking attacks. Specifically, the Geth instrumentation enables the attacker node to monitor the local mempool and send a crafted transaction to the victim node upon each new empty slot created (by block arrival). The network topology is depicted in Figure~\ref{fig:exp:setup4}.

In the experiment, we first run our three nodes for $350$ minutes and then turn on the locking attack on the attacker node. We collect the benign transactions received by the attacker node (the number of which is denoted by $N_a$), the crafted transactions the attacker sends (the number denoted by $N_c$), and the benign transactions received by the measurement node (the number denoted by $N_m$). We use Metric $\frac{N_a}{N_m}$ to report the (inverse) of the attack success rate -- Under the same transactions received by the measurement node, the fewer transactions the attacker node receives from the victim node, the more successful the victim mempool is locked. 

\noindent{\bf 
Evaluation of locking attacks}: 
We report in Figure~\ref{fig:ld5:x} the locking attack's success rate over the period of $350$ minutes. Each tick on the $X$ axis represents $1$ minute; that is, $N_a$/$N_m$ is the number of benign transactions received by the attacker/measurement node every $1$ minute. It is clear that the locking attack is highly successful -- Right after the attack is launched at the $180$-th minute, the rate of normalized transactions received from the victim node drops essentially to zero. And it persists over the period where the attack lasts.

We also calculate the attack cost by the total fees of the attacker's transactions included in the blockchain. In the experiment, we wait three hours after the attack stops and consider all the blocks produced until then. Not a single attacker's transaction sent in our experiment is included in the blockchain. This may be due to the low fee with which crafted transactions are sent.  

Understanding crafted transaction inclusion is nondeterministic and dependent on benign transactions, we estimate the worst-case attack cost, which is the total fees of crafted transactions sent by the attacker (i.e., when all the crafted transactions are included in the blockchain). Figure~\ref{fig:ld5:3} reports the worst-case locking attack cost over time; on average, the attack, as successful as reported in Figure~\ref{fig:ld5:x}, consumes $0.0004$ Ether per block. By comparison, it is $0.028$ Ether of transactions included per block, which is the minimal cost of the baseline transaction-spamming attack~\cite{DBLP:conf/fc/BaqerHMW16}.

\ignore{
\section{Discussion: The Case of MemPurge Attack}
A mempool-DoS attack, named MemPurge, has been described in a preprint~\cite{cryptoeprint:2023/956}. We describe the mechanism how MemPurge works on Geth, evaluate the attacks on Geth with varying conditions, and present an assessment and mitigation of the attack.

\noindent{\bf 
Attack mechanism}: 
On a Geth node, the MemPurge paper~\cite{cryptoeprint:2023/956} assumes the initial state of the target mempool that stores $5120$ normal transactions sent from victim account, say Alice, and of nonces $1, 2, 3, \dots, 5120$. 

\ballnumber{1} The attacker sends $64$ transactions from attacker account B1 and, respectively, of nonces $2, 3, \dots, 65$. These $64$ transactions are admitted to the Geth mempool as future transactions. \ballnumber{2} The attacker then sends a ``reconnecting''  transaction, say $tx$, from account B1 and of nonce 1 to the mempool. $tx$'s value, i.e., the amount of Ether transferred, is set so that $tx.value$ is lower than account $B1$'s balance but $tx.value+tx'.value$ is higher than $B1$'s balance, where $tx'$ is $B1$'s transaction of nonce 2. The mempool of Geth $v1.20.2$ admits $tx$, which turns all the $64$ transactions into pending-and-latent-overdraft transactions. The newly turned pending transactions trigger Geth's limit of $64$ pending transactions per sender, and would evict $65$ pending transactions from Alice. Thus, after \ballnumber{1} and \ballnumber{2}, the mempool stores $5120-65$ normal transactions from Alice and $65$ pending transactions from $B1$. Note that of the $65$ transactions from $B1$, $64$ are latent overdraft and the other one (of nonce $1$) is a valid transaction (of low fees).

The attacker repeats Steps \ballnumber{1} and \ballnumber{2} for 78 times, each time using a distinct sender account (i.e., $B2, B3, \dots, B78$). Eventually, $78*65=5070$ Alice's transactions are evicted from the mempool at an attack cost of $78$ pending transactions at minimal fees.

\noindent{\bf 
Attack evaluation}: We have run the MemPurge attack, exactly as described above (and in the preprint~\cite{cryptoeprint:2023/956}), on a local Geth $v1.11.4$ node. The attack works as presented in the paper.

We notice the assumption made about the initial state (of $5120$ normal transactions sent from one victim account) is very strong. In practice, it is very unlikely that a real mempool content would be set up this way. We thus modify the initial state to be more realistic: Initial state $IS2$: $5120$ normal transactions sent from $5120$ different victim accounts (i.e., one transaction per victim account), and Initial state $IS3$: $5120$ normal transactions sent from 5120/2=2560 distinct victim accounts (i.e., two transactions per victim account). We rerun the same attack transactions against more realistic initial states $IS2$ and $IS3$, and the MemPurge attack did not succeed. To be more specific, in both initial settings, the attack cannot evict a single victim transaction from the mempool.

Due to this reason, we believe MemPurge attacks, at least in its current design, are not practical and do not pose real threats. 

Besides, the MemPurge attack exploits Geth-specific features (e.g., limiting 64 transactions of the same sender only when there are more than $5120$ pending transactions in the mempool) and is inapplicable to other Ethereum clients that don't have such limits.

\noindent{\bf 
Attack assessment and mitigation}: The cause of the MemPurge attacks is that the detection of latent overdraft transactions, as merged into Geth $v1.11.4$ codebase, is not triggered if the arriving transactions are first future transactions and then turned to pending-and-latent-overdraft transactions. In other words, this is an implementation bug that can be easily fixed. 

On the Internet, code patch against MemPurge is developed for Geth~\cite{me:mempurge:fix}. We run MemPurge attack with its original one-sender initial state against the patched Geth code. It shows the MemPurge attack did not succeed, that is, the attack transactions are not admitted to the $5120$ mempool slots supposed to store pending transactions in Geth. 

In hindsight, given a mempool section supposed to store only valid (or pending) transactions, the MemPurge attack follows the same transaction pattern as DETER, that is, evict-by-invalid transactions. The sophistication here in MemPurge is that the invalid transactions are first buffered in the future-transaction mempool as future transactions and are then reconnected to become pending transactions that are invalid (or latent overdraft). The arriving transactions seen by the pending transaction mempool in MemPurge are invalid transactions.
}

{
\section{Root-Cause Analysis and Mitigation}
\label{appdx:sec:mitigate}

This section analyzes the root causes of found exploits (i.e., $XT_1$ - $XT_9$ described in \S~\ref{sec:exploits}) and presents rule-based mitigation strategies.

\noindent{\bf Analytical methods}: Recall that each exploit is a sequence of transaction-admission events following certain patterns. While some admission events can be easily justified by the need to increase block revenues (e.g., let an existing transaction of low price to be evicted by a transaction of high price), we observe in each exploit there are other admission events where optimizing block revenue in one case can conflict with that in some other cases. We attribute the root cause of an exploit to those ``conflicting'' admission events.

\newcommand{\tikzmarkvertical}[1]{\tikz[overlay,remember picture] \node (#1) {};}
\newcommand{\DrawBox}[1][]{%
        \tikz[overlay,remember picture]{      
        \draw[red,#1]
          ($(left1)+(-0.5em,1.6ex)$) rectangle
          ($(right1)+(0.5em,-0.6ex)$);
        \draw[red,#1]
          ($(left2)+(-0.5em,1.6ex)$) rectangle
          ($(right2)+(0.5em,-0.6ex)$);
        \draw[red,#1]
          ($(left16)+(-0.5em,1.6ex)$) rectangle
          ($(right16)+(0.5em,-5.95ex)$);
        \draw[red,#1]
          ($(left17)+(-0.5em,1.6ex)$) rectangle
          ($(right17)+(0.5em,-5.90ex)$);
        \draw[red,#1]
          ($(left3)+(-0.5em,1.6ex)$) rectangle
          ($(right3)+(0.5em,-0.6ex)$);
        \draw[red,#1]
          ($(left4)+(-0.5em,1.6ex)$) rectangle
          ($(right4)+(0.5em,-19.0ex)$);
        %\draw[red,#1]
        %  ($(left5)+(-0.5em,1.4ex)$) rectangle
        %  ($(right5)+(0.5em,-0.5ex)$);
        \draw[red,#1]
          ($(left6)+(-0.5em,1.6ex)$) rectangle
          ($(right6)+(0.5em,-3.2ex)$);
        %\draw[red,#1]
        %  ($(left7)+(-0.5em,1.4ex)$) rectangle
        %  ($(right7)+(0.5em,-0.5ex)$);
        \draw[red,#1]
          ($(left8)+(-0.5em,1.6ex)$) rectangle
          ($(right8)+(0.5em,-0.6ex)$);
        \draw[green,#1]
          ($(left9)+(-0.5em,1.6ex)$) rectangle
          ($(right9)+(0.5em,-0.6ex)$);
        \draw[green,#1]
          ($(left10)+(-0.5em,1.6ex)$) rectangle
          ($(right10)+(0.5em,-0.6ex)$);
        \draw[green,#1]
          ($(left18)+(-0.5em,1.6ex)$) rectangle
          ($(right18)+(0.5em,-0.6ex)$);
        \draw[green,#1]
          ($(left11)+(-0.5em,1.6ex)$) rectangle
          ($(right11)+(0.5em,-0.6ex)$);
        \draw[green,#1]
          ($(left12)+(-0.5em,1.6ex)$) rectangle
          ($(right12)+(0.5em,-3.2ex)$);
        \draw[green,#1]
          ($(left14)+(-0.5em,1.6ex)$) rectangle
          ($(right14)+(0.5em,-0.6ex)$);
        \draw[green,#1]
          ($(left15)+(-0.38em,1.6ex)$) rectangle
          ($(right15)+(0.38em,-0.6ex)$);
        %\draw[red,#1]
        %  ($(left10)+(-0.5em,1.4ex)$) rectangle
        %  ($(right10)+(0.5em,-0.5ex)$);
        %\draw[red,#1]
        %  ($(left11)+(-0.5em,1.4ex)$) rectangle
        %  ($(right11)+(0.5em,-0.5ex)$);
        %\draw[red,#1]
        %  ($(left12)+(-0.5em,1.4ex)$) rectangle
        %  ($(right12)+(0.5em,-0.5ex)$);
        \draw[red,#1]
          ($(left13)+(-0.5em,1.6ex)$) rectangle
          ($(right13)+(0.5em,-0.6ex)$);

        }
        }

\begin{table*}[!htbp]
  \caption{Root causes of found exploits expressed by symbolized admission patterns (SAP).}
  \label{tab:causes}
  \centering{\footnotesize
  \begin{tabularx}{0.825\textwidth}{|l|X|*{10}{c}|}
  \hline
Name&Pattern & $XT_1$ & $XT_2$ & $XT_3$ &$XT_4$ & $XT_5$ & $XT_6$ & $XT_7$ & $MN_*$  & $XT_9$ & $XT_8$\\ \hline
   $SAP_1$& $[\mathcal{C}|\mathcal{P}] \rightarrow \mathcal{F}$ & \tikzmarkvertical{left1} \cmark \tikzmarkvertical{right1} & & \tikzmarkvertical{left16} \cmark \tikzmarkvertical{right16} && & & & \tikzmarkvertical{left9}\xmark\xmark \tikzmarkvertical{right9}& &\tikzmarkvertical{left4} \xmark\xmark \tikzmarkvertical{right4}\\ \hline 
$SAP_2$& $[\mathcal{C}|\mathcal{P}]\cdot{} [\mathcal{C}|\mathcal{P}] \rightarrow \mathcal{P}\cdot{}\mathcal{L}$ & &\tikzmarkvertical{left2} \cmark \tikzmarkvertical{right2}  & \cmark& && & &\tikzmarkvertical{left10}\xmark\xmark\tikzmarkvertical{right10} &&\xmark\xmark \\ \hline 
$CRP_1$ & (Conditional limit of txs per sender)  & &  & \cmark & &  &\tikzmarkvertical{left17} \cmark \tikzmarkvertical{right17}&&\tikzmarkvertical{left18}\xmark\xmark\tikzmarkvertical{right18} &&\xmark\xmark \\ \hline 
$SAP_4$& $\mathcal{P}\cdot\mathcal{C}\xrightarrow[]{\text{r}}\mathcal{P}\mathcal{L}$ & & &   & \tikzmarkvertical{left13} \cmark \tikzmarkvertical{right13}& & &&\tikzmarkvertical{left11}\xmark\xmark \tikzmarkvertical{right11}&&\xmark\xmark\\ \hline 
$SAP_5$& $\mathcal{P}\cdot{}\mathcal{C}\rightarrow\mathcal{F}\cdot{}[\mathcal{P}|\mathcal{C}]$ & &  & & & \tikzmarkvertical{left3} \cmark \tikzmarkvertical{right3}&\cmark& &\tikzmarkvertical{left12}\xmark\xmark \tikzmarkvertical{right12} & 
\tikzmarkvertical{left6} \xmark\xmark \tikzmarkvertical{right6}&\xmark\xmark\\ \hline 

$SAP_9$ & $\mathcal{P}_l \mathcal{C}_h \rightarrow{} \mathcal{P}_l \mathcal{P}_m$ & &  &  & &  && & \cmark & \xmark\xmark &\xmark\xmark\\ \hline 
$SAP_{11}$ & $C_l\rightarrow{}C_h$ &&&&&&&&\tikzmarkvertical{left15}\cmark\cmark\tikzmarkvertical{right15}&&\xmark\xmark\\ \hline 
$CRP_2$ & $\forall{SAP}, SAP\land{}\textsc{reversed}(SAP)$
 %(e.g.,  $\mathcal{P}_l\cdot\mathcal{C}_h \rightarrow{} \mathcal{P}_l \cdot \mathcal{P}_m \land{} \mathcal{P}_l \cdot \mathcal{P}_m \rightarrow{} \mathcal{P}_l \cdot\mathcal{C}_h$)
 & & && &  & &\tikzmarkvertical{left8} \cmark \tikzmarkvertical{right8} & \tikzmarkvertical{left14}\xmark\xmark \tikzmarkvertical{right14}  &&\xmark\xmark\\ \hline 
  \end{tabularx}
  }
\DrawBox[ultra thick]
\end{table*}

\begin{table}[!htbp] %force in current page, disable float.
\caption{Mitigation schemes}
\label{tab:mitigate}\centering{\small
\begin{tabularx}{0.375\textwidth}{ l|X }
Scheme & Expression \\ \hline
$MN_1$ & $SAP_1=$\xmark\xmark{} $\land{} SAP_2=$\xmark\xmark{} $\land{} SAP_4=$\xmark\xmark
\\ 
$MN_2$ & $SAP_{11}=$\cmark\cmark
\\
$MN_3$ & $SAP_9=$\cmark{} $ \land{}$ $SAP_5=$\xmark\xmark{} 
\\
$MN_4$ & $\forall{}SAP, SAP \land{}$ $\textsc{reversed}(SAP)=$\xmark\xmark{} 
\\
  \end{tabularx}
}
\end{table}

Specifically, consider an admission event $\textsc{txAd}(tx_1\cup{}st', tx_2) \rightarrow{} tx_2\cup{}st'$ where $tx_1$ in the mempool is evicted by the arriving $tx_2$. Note that $st'$ remains unchanged before and after the admission. 
We establish the Symbolized Admission Pattern (or SAP) by $Symbol(tx_1)\rightarrow{}Symbol(tx_2)$. If $\exists{}st'$, such that $\textsc{txAd}(tx_1\cup{}st', tx_2) \rightarrow{} tx_2\cup{}st'$, we define SAP $Symbol(tx_1)\rightarrow{}Symbol(tx_2)$ is ``sometimes turned on'' (\cmark). If $\forall{}st', tx_1'\in{}Symbol(tx_1), tx_2'\in{}Symbol(tx_2)$, $\textsc{txAd}(tx_1'\cup{}st', tx_2')$ does not end with $tx_2'\cup{}st'$, we define SAP $Symbol(tx_1)\rightarrow{}Symbol(tx_2)$ is ``always turned off'' (\xmark\xmark). 

We summarize six SAP from the nine found exploits and list them in the second columns in Table~\ref{tab:causes}. Here, if an SAP involves with two transactions, we follow our conventions in ordering symbols based on sender and then nonces.
For instance, $SAP_1$, that is, $[\mathcal{C}|\mathcal{P}]\rightarrow\mathcal{F}$, describes the eviction of one valid transaction, be it a parent or child transaction by an arriving future transaction. Here, we use the regular expression $[|]$ to denote one transaction that is either $\mathcal{C}$ or $\mathcal{P}$. 
For the second example, $SAP_5$, that is, $\mathcal{P}\cdot{}\mathcal{C}\rightarrow\mathcal{F} [\mathcal{P}|\mathcal{C}]$ describes the eviction of a parent transaction by another valid transaction, turning the child transaction into future. 
For the third example, $SAP_4$, $\mathcal{P}\cdot\mathcal{C}\xrightarrow[]{\text{r}}\mathcal{P}\mathcal{L}$ describes the replacement ($\xrightarrow[]{\text{r}}$) of a parent transaction with a higher value that turns its children into latent overdraft. 

We attribute the exploits to four causes, each related to a certain combination of one or several SAP'es. The mapping between exploits and their cause SAP'es is in Table~\ref{tab:causes}. 

\noindent{\bf
Cause 1: Presence of individual SAP}: Eviction-based exploits, including $XT_1$, $XT_2$, $XT_4$, and $XT_7$, can be attributed to the fact that a certain SAP is sometimes turned on in the victim mempool. For example, $SAP_4$ is sometimes on in Geth $<v1.11.4$, and Exploit $XT_4$ exploits this fact to first evict the mempool using adversarial transactions and then reduce attack costs by turning all adversarial child transactions into latent overdraft. 

\noindent{\bf
Mitigation design $MN_1$}: We propose a rule-based mitigation scheme $MN_1$ against exploits of cause 1. In $MN_1$, the mempool detects and prohibits all admission events that satisfy the SAP that causes the target exploits. For instance, against $XT_4$, $MN_1$ would decline any admission event matching $SAP_4$. We implement this mitigation on Geth, and it is now merged into Geth $v1.11.4$~\cite{me:gethfix11}.
The $MN_1$ schemes against other exploits of the same cause, like $XT_1$ and $XT_2$, can be found in Table~\ref{tab:mitigate}.

\noindent{\bf
Cause 2: Absence of individual SAP}: Locking-based exploits, including $XT_8$ and $XT_9$, are attributable to the fact that some SAP'es are always absent on the victim mempool. For instance, the mempool in Reth $<v0.1.0-alpha.6$ was an FIFO queue and prohibits evictions of any kind (i.e., all of $SAP_1, SAP_2, \dots, SAP_{11}$ are always off). 

\noindent{\bf
Mitigation design $MN_2$}: We propose to mitigate exploits of cause 2 by reenacting some SAP, such as price-based eviction, that is, $SAP_{11}: C_l\rightarrow{}C_h$, and making it always turned on (i.e., \cmark\cmark{} ). Scheme $MN_2$ is described in Table~\ref{tab:mitigate}.

\noindent{\bf
Cause 3: Combination of multiple SAPes}: Some exploits can be attributed to a certain combination of multiple $SAP$'es. For instance, $XT_9$ can be attributed to that $SAP_5$ and $SAP_9$ are always turned off. 

\noindent{\bf
Mitigation design $MN_3$}: Because the $SAP_5$ that $XT_9$ relies on is also related to Exploit $XT_5$. One has to consider both exploits when designing mitigation schemes. We propose bypassing both $SAP$ patterns causing the exploit with $SAP_5=$\xmark\xmark{} $\land{} SAP_9=$\cmark . Specifically, the admission decision regarding $SAP_9$ is randomized so it can be sometimes turned on ($SAP_9=$\cmark). Making $SAP_9$ always turned on may decrease block revenue, and we leave it to the future work for fully exploring the design space of $MN_3$.

\ignore{
Exploit $XT_5$ can be attributed to the presence of $SAP_5$ being sometimes on. One mitigation is to make $SAP_5$ always off, that is, prohibit the eviction of a parent transaction in any case. In other words, only childless transactions (i.e., transactions without children) can be evicted. 

Under this circumstance, while it seems intuitive to prohibit evicting a high-priced transaction by a low-priced transaction (i.e., making $SAP_9$ always off), the combination of $SAP_9=$\xmark\xmark{} and $SAP_5=$\xmark\xmark{} would introduce the vulnerability of $XT_9$. Specifically, Policy $SAP_9=$\xmark\xmark{} and $SAP_5=$\xmark\xmark{} leaves the mempool no choice but always declines an arriving transaction of high price, introducing $XT_9$. For instance, in practice, OpenEthereum adopts the combination of $SAP_9=$\xmark\xmark{} and $SAP_5=$\xmark\xmark{}  is found vulnerable to $XT_9$.

We propose to mitigate both $XT_5$ and $XT_9$, by the rule above. Here, we propose one specific policy in compliance with $MN_3$, in which the admission decision regarding $SAP_9$ is randomized, so that the counter-intuitive admission can be turned on, $SAP_9=$\cmark. Making $SAP_9$ always on would decrease block revenue. Fully exploring the design space of $MN_3$ would be the future work.
}

\noindent{\bf
Policy-specific cause 4}: Some exploits are adaptive and specific to the admission policies of the victim mempool. The examples include $XT_3$, $XT_6$ and $XT_7$. 
For instance, $XT_3$/$XT_6$ are caused by the condition that triggers the protective admission policies; such condition is evadable. For instance, on Geth, when the mempool stores more than $py_3'=5120$ pending transactions (named as $CRP_1$), it triggers the policy to limit the number of transactions per sender under $py_2'=16$. The condition regarding $py_3'$ is evaded in $XT_3$ and $XT_6$. Here, $CRP$ refers to context-relevant properties, as the admission of a transaction $tx$ depends on the context of the mempool states.

Exploit $XT_7$ is caused by the inconsistency between an admission event and its reversed event. The conjunctive form, $CRP_2: SAP_9 \land{} \textsc{reverse}(SAP_9)$, is sometimes turned on. 

\noindent{\bf
Policy-specific mitigation design $MN_4$}: To mitigate policy-specific exploits, our proposed mitigation scheme is also policy-specific. For instance, to mitigate $XT_7$, we propose enforcing that the conjunction of any SAP and its reversed one does not hold (see Table~\ref{tab:mitigate}). To mitigate $XT_3$ and $XT_6$, we propose making the protective policy conditionless, that is, $py_3'=0$ .

%More specifically, this conjunctive form means $\exists{}st'$, such that $\textsc{txAd}(tx_1\cup{}st', tx_2)=tx_2\cup{}st' \land \textsc{txAd}(tx_2\cup{}st', tx_1)=tx_1\cup{}st'$. 
}

{
\section{Transaction Symbols and Code Coverage}
\label{appdx:transaction-code-coverage}

\noindent{\bf
Methodology}: This section measures the code coverage of mempool admitting transactions under the same and different symbols. To do so, given a symbol, we randomly generate $20$ different transactions in the transaction space covered by the symbol and then initialize an Ethereum client to admit each transaction in its mempool. The initial mempool is full of $6144$ pending transactions from $6144$ distinct senders. After the transaction admission, we collect the code coverage; for instance, when we run Geth (with versions before and after $v1.11.4$), we use the built-in code-coverage tool~\cite{me:gocover}. The collected code coverage is a linearized list of code blocks, each tagged with the number of times the block is executed. We denote the code-coverage metric under transaction $tx$ by $cc(tx)$. Then, for each symbol $\mathcal{S}$, we aggregate the code coverage metrics of all $20$ transactions generated under $\mathcal{S}$ and name the symbol-wise code coverage by $cc(\mathcal{S})$.

We report the pairwise symbol distance by the dissimilarity between the symbol code coverage metrics. That is, given two symbols, say $\mathcal{S}_1$ and $\mathcal{S}_2$, their distance is defined as follows:

$$
Dist(\mathcal{S}_1, \mathcal{S}_2) = 
\frac{\sum_{\forall{}p_i\in{}cc(\mathcal{S}_1), p_j\in{}cc(\mathcal{S}_2)} Dist(p_i, p_j)}{ 
\sum_{\forall{}p_i\in{}cc(\mathcal{S}_1), p_j\in{}cc(\mathcal{S}_2)} 1}
$$

$$
Dist(p_i, p_j) = 1 - \frac{p_i \cap p_j}{p_i \cup p_j}
$$

\begin{table}[!htbp]
  \caption{Difference of symbol code coverage ($Geth < V1.11.4$)}
  \label{tab:ccdist:geth1}
  \centering{\scriptsize
  \begin{tabularx}{0.495\textwidth}{ |l|X|X|X|X|X|X| }
  \hline
  Symbol  & $\mathcal{F}$ & $\mathcal{P}$ & $\mathcal{C}$ & $\mathcal{L}$ & $\mathcal{R}$ &$\mathcal{RL}$  \\ \hline 
  $\mathcal{F}$ & ${\bf 0.23\%}$ &$6.80\%$ &$6.80\%$&$6.80\%$&$14.99\%$&$14.99\%$\\ \hline 
  $\mathcal{P}$ & \cellcolor{black!25} & ${\bf 0.23\%}$ &$2.01\%$& $2.01\%$& $17.31\%$& $17.31\%$\\ \hline 
  $\mathcal{C}$ & \cellcolor{black!25} & \cellcolor{black!25} & ${\bf 0.30\%}$ & ${\bf 0.30\%}$& $17.00\%$& $17.00\%$ \\ \hline
  $\mathcal{L}$ &\cellcolor{black!25} &\cellcolor{black!25}&\cellcolor{black!25} & ${\bf 0.30\%}$& $17.00\%$ & $17.00\%$ \\ \hline
  $\mathcal{R}$ &\cellcolor{black!25} &\cellcolor{black!25}&\cellcolor{black!25} &\cellcolor{black!25}& ${\bf 0.92\%}$& ${\bf 0.92\%}$\\ \hline
  $\mathcal{RL}$ &\cellcolor{black!25} &\cellcolor{black!25}&\cellcolor{black!25}&\cellcolor{black!25}&\cellcolor{black!25} &${\bf 0.92\%}$ \\ \hline
\end{tabularx}
}
\end{table}

\begin{table}[!htbp]
  \caption{Difference of symbol code coverage ($Geth \geq{} V1.11.4$)}
  \label{tab:ccdist:geth2}
  \centering{\scriptsize
  \begin{tabularx}{0.495\textwidth}{ |l|X|X|X|X|X|X| }
  \hline
  Symbol  & $\mathcal{F}$ & $\mathcal{P}$ & $\mathcal{C}$ & $\mathcal{L}$ &$\mathcal{R}$ &$\mathcal{RL}$ \\ \hline 
  $\mathcal{F}$ & ${\bf 0.23\%}$ &$6.71\%$ &$7.01\%$&$13.73\%$ & $15.37\%$& $14.03\%$\\ \hline 
  $\mathcal{P}$ & \cellcolor{black!25} & ${\bf 0.23\%}$ &$2.23\%$& $17.76\%$& $17.62\%$ & $17.91\%$\\ \hline 
  $\mathcal{C}$ & \cellcolor{black!25} & \cellcolor{black!25} & ${\bf 0.45\%}$& $17.46\%$& $16.86\%$& $13.73\%$\\ \hline
  $\mathcal{L}$ &\cellcolor{black!25} &\cellcolor{black!25}&\cellcolor{black!25} & ${\bf 0}$& $11.34\%$& ${\bf 0.15\%}$\\ \hline
  $\mathcal{R}$ &\cellcolor{black!25} &\cellcolor{black!25}&\cellcolor{black!25} &\cellcolor{black!25}& ${\bf 0.89\%}$& $11.12\%$\\ \hline
  $\mathcal{RL}$ &\cellcolor{black!25} &\cellcolor{black!25}&\cellcolor{black!25}&\cellcolor{black!25}&\cellcolor{black!25} & ${\bf 0}$\\ \hline
\end{tabularx}
}
\end{table}

\noindent{\bf
Results}: In the experiment, we measure the code coverage on two Geth clients ($V1.11.3$ and $v1.11.4$) under the following symbols $\mathcal{F}$, $\mathcal{P}$, $\mathcal{C}$, $\mathcal{R}$, $\mathcal{L}$, and $\mathcal{RL}$. We report the pairwise symbol distance in Tables~\ref{tab:ccdist:geth1} and ~\ref{tab:ccdist:geth2}.

In Table~\ref{tab:ccdist:geth1}, the same-symbol distance (i.e., $\mathcal{S}_1=\mathcal{S}_2$) is consistently below 1\%, and the different-symbol distance (i.e., $\mathcal{S}_1\neq{}\mathcal{S}_2$) is consistently above 5\%, except for the exception cases as will be described. In Table~\ref{tab:ccdist:geth2}, the same-symbol distance (i.e., $\mathcal{S}_1=\mathcal{S}_2$) is consistently below 0.9\%, and the different-symbol distance (i.e., $\mathcal{S}_1\neq{}\mathcal{S}_2$) is consistently above 6\% except the following cases: In both tables, the code-coverage distances between Symbols $\mathcal{C}$ and $\mathcal{P}$ are low (e.g., $2.23\%$ in Table~\ref{tab:ccdist:geth2}). The distances between Symbols $\mathcal{L}$ and $\mathcal{RL}$ in both tables are also low, such as $0.15\%$ in Table~\ref{tab:ccdist:geth2}. The low distance shows that the two symbols are handled by similar code paths and can result in the similar mempool behavior. 

The current results show the match between symbols and mempool code coverage, with some disparity. We leave it to the future work to explore the automatic generation of symbols from mempool implementation. 
}

\ignore{
{
{\color{green}{\section{Evaluation of Locking OpenEthereum in Local Networks}}} \yw{We do not describe LD1,2,4,5 in previous section. I suggest removing this section. If we keep this section, please note Fig 18 is not referenced}
To evaluate the effectiveness of Lock attacks on OpenEthereum, we set up a private network of three nodes: A victim OpenEthereum miner node, an attacker node and a normal node. The victim OpenEthereum node connects to both attacker node and normal node. There is no connection between the miner and attacker nodes. In each experiment to be described below, we first populate the miner node with $5120$ normal transactions with a medium Gas price (e.g., 1 Gwei). Then we generate normal transactions of the same medium Gas price at the rate of $50$ transactions per second. Meanwhile, we turn on the mining on the miner node. The attacker node then launches the attack by sending a message of $5120$ attack transactions of patterns ED2/4/LD2/4 to the miner node. From the normal node, we send normal transactions to the miner node for $1000$ seconds. After that, we turn off mining and report the accumulative number of included transactions at different block height. For comparison, we also run experiments without the attack.
We repeat the experiment three times and report the mean and standard deviation of the accumulative number of included normal transactions.

\begin{figure}[!ht]
  \centering
    \subfloat[Success rate]{%
  \includegraphics[width=0.25\textwidth]{figures/exp-Numberofincludedtransactions-Blockheight-Open-LD24-ED24.eps}
  \label{fig:local:lock_open_LD24_ED24}
    }%
    \subfloat[Attack costs]{%
  \includegraphics[width=0.25\textwidth]{figures/exp-Attackcost-Open-ED24-LD24.eps}
  \label{fig:local:lock_open_LD24_ED24_cost}}
  \caption{ADAMS attacks exploiting latent overdraft transactions on OpenEthereum}%
  \label{fig:local:lock_open1}
\end{figure}

\begin{figure}[!ht]
  \centering
    \subfloat[Success rate]{%
  \includegraphics[width=0.25\textwidth]{figures/exp-Numberofincludedtransactions-Blockheight-Open-LD5.eps}
  \label{fig:local:lock_open_LD5}
    }%
    \subfloat[Attack costs]{%
  \includegraphics[width=0.25\textwidth]{figures/exp-Attackcost-LD5.eps}
  \label{fig:local:lock_open_LD5_cost}}
  \caption{ADAMS attacks exploiting LD5 on OpenEthereum}%
\end{figure}

Figure~\ref{fig:local:lock_open1} presents the result of ED2/4/LD2/4 attacks. From the result, it can be seen that when no attack is mounted (black line), as the block height grows, the number of normal transactions included in the block steadily increases, and at block height $100$, more than $27534$ normal transactions are included; However, when the attack with seed ED2 is mounted (pink line), the number of normal transactions included at block height $100$ is reduced to $6002$. The result shows this attack can achieve a success rate of $78.2\%$. Besides, when the attack with seed LD2 is launched (blue line), the number of included normal transactions at block $100$ is $7296$, which achieves a success rate of $73.5\%$. In addition, when the attack with seed ED4 is launched (red line), the number of included normal transactions is $380$. For seed LD4, the number of included normal transactions is $7928$. Comparing all four attack seeds, D6 is the most effective seed which can achieve the highest success rate of $98.6\%$. 
}
}
\section{More Related Works}
\label{appdx:more-related-work}

\noindent{\bf 
Exhaustion by contract execution}: Normally, a blockchain node executes a smart contract after deciding to include the transaction in the blockchain. Gas mechanism is deployed to mitigate the risk of computation exhaustion, that is, to charge the attacker with high fees who deploy a computationally expensive smart contract to exhaust the victim node's resources. Existing works explore the smart contract space and find the one that consumes computing resources at low prices to construct attacks~\cite{DBLP:conf/ndss/0002L20}. Such low-price instructions exist for reasons such as heterogeneous hardware, variant execution environment, etc.

A blockchain node may speculatively execute a smart contract, that is, execute smart contract {\it before}, including the invoking transaction. One can misuse speculative execution to send invalid transactions speculatively executing smart contracts. This can cause two types of DoS, yet at low costs: 1) Exhaust the victim node's computing resources by deploying and invoking computationally expensive smart contracts.
DoERS attack~\cite{DBLP:conf/ndss/LiCLT0L21} is an exhaustion attack by misusing the speculative execution on Ethereum RPC nodes (i.e., eth\_call) to exhaust computations. ConditionalExhaust~\cite{cryptoeprint:2023/956} misuses the speculative execution by block validators in post-merge Ethereum, which is designed for censoring addresses. 2) Occupy the mempool by sending invalid transactions; for instance, in ConditionalExhaust with MemPurge~\cite{cryptoeprint:2023/956}, an attacker sends invalid transactions triggering failed speculative executions to occupy a victim mempool at low cost.

In particular, in MemPurge~\cite{cryptoeprint:2023/956}, an attacker sends future transactions and then sends a transaction with a nonce reconnecting the nonces of the future transactions and turning them back to latent-overdraft transactions. The future-turned-latent-overdraft transactions are admitted to the mempool and evict normal transactions at low costs.

{
\section{Relaxed Bug Oracle Design}
\label{sec:oracle:relaxed}

We define a strict bug oracle (i.e., erasing all benign TXs) to counter the effect that our fuzzer needs to run in a smaller-than-usual mempool so that the exploits found in the small mempool are true positives in the actual mempool.

For instance, in Geth, the mempool can store up to $5120$ pending transactions, and a typical block stores < 200 transactions in the mainnet. To ensure the impact of a mempool under attack on the next block (e.g., preventing at least one benign transaction from the block), more than $4920$ ($=5120-200$) benign transactions in the mempool need to be evicted. When fuzzing, we use a small mempool (e.g., length $m=3, 6, 16$). Even with $m=16$ and when \textsc{mpfuzz} evicts 15 normal transactions, the exploit found will cause the eviction of $15/16*5120 = 4800 < 4920$ benign transactions in an actual Geth mempool, unable to prevent any benign transactions in the next block. In other words, this exploit found would be a false positive in an actual mempool. We will clarify and evaluate this observation in the paper.

All known ADAMS attacks today (i.e., DETER attacks) can be rediscovered by \textsc{mpfuzz}, making no undiscovered attacks by \textsc{mpfuzz} or zero false negatives. In theory, our bug oracle does not ensure completeness and can cause false negatives.

{
\subsection{Evaluation}

We evaluate the true positive rate when relaxing the bug oracle during fuzzing. 
\begin{definition}[Relaxed eviction bug oracle] Given a $m$-length mempool  (e.g., m = 6), a transaction admission timeline, $\langle{}st_0, dc_0=\emptyset\rangle{}, ops \Rightarrow{}\langle{}st_n, dc_n\rangle{}$, is a successful eviction attack, if.f.  1) at least $t$ normal transactions ($t < m$) in initial state $st_{0}$ is evicted and 2) the total adversarial transaction fees in the end state $st_n$ to be charged are smaller, by a multiplicative factor $\epsilon$, than the attack damage measured by the fees of evicted transactions in the initial state $st_0$. While not all the normal transactions in $st_0$ are evicted, the normal transactions left in the end state $st_n$ are denoted as $st_{nN}$ and the attack transactions are denoted as $st_{nA}$. Thus, the attack damage is denoted as $st_0-st_{nN}$. Formally, 
\begin{figure}[!tb]
  \centering
  \includegraphics[width=0.275\textwidth]{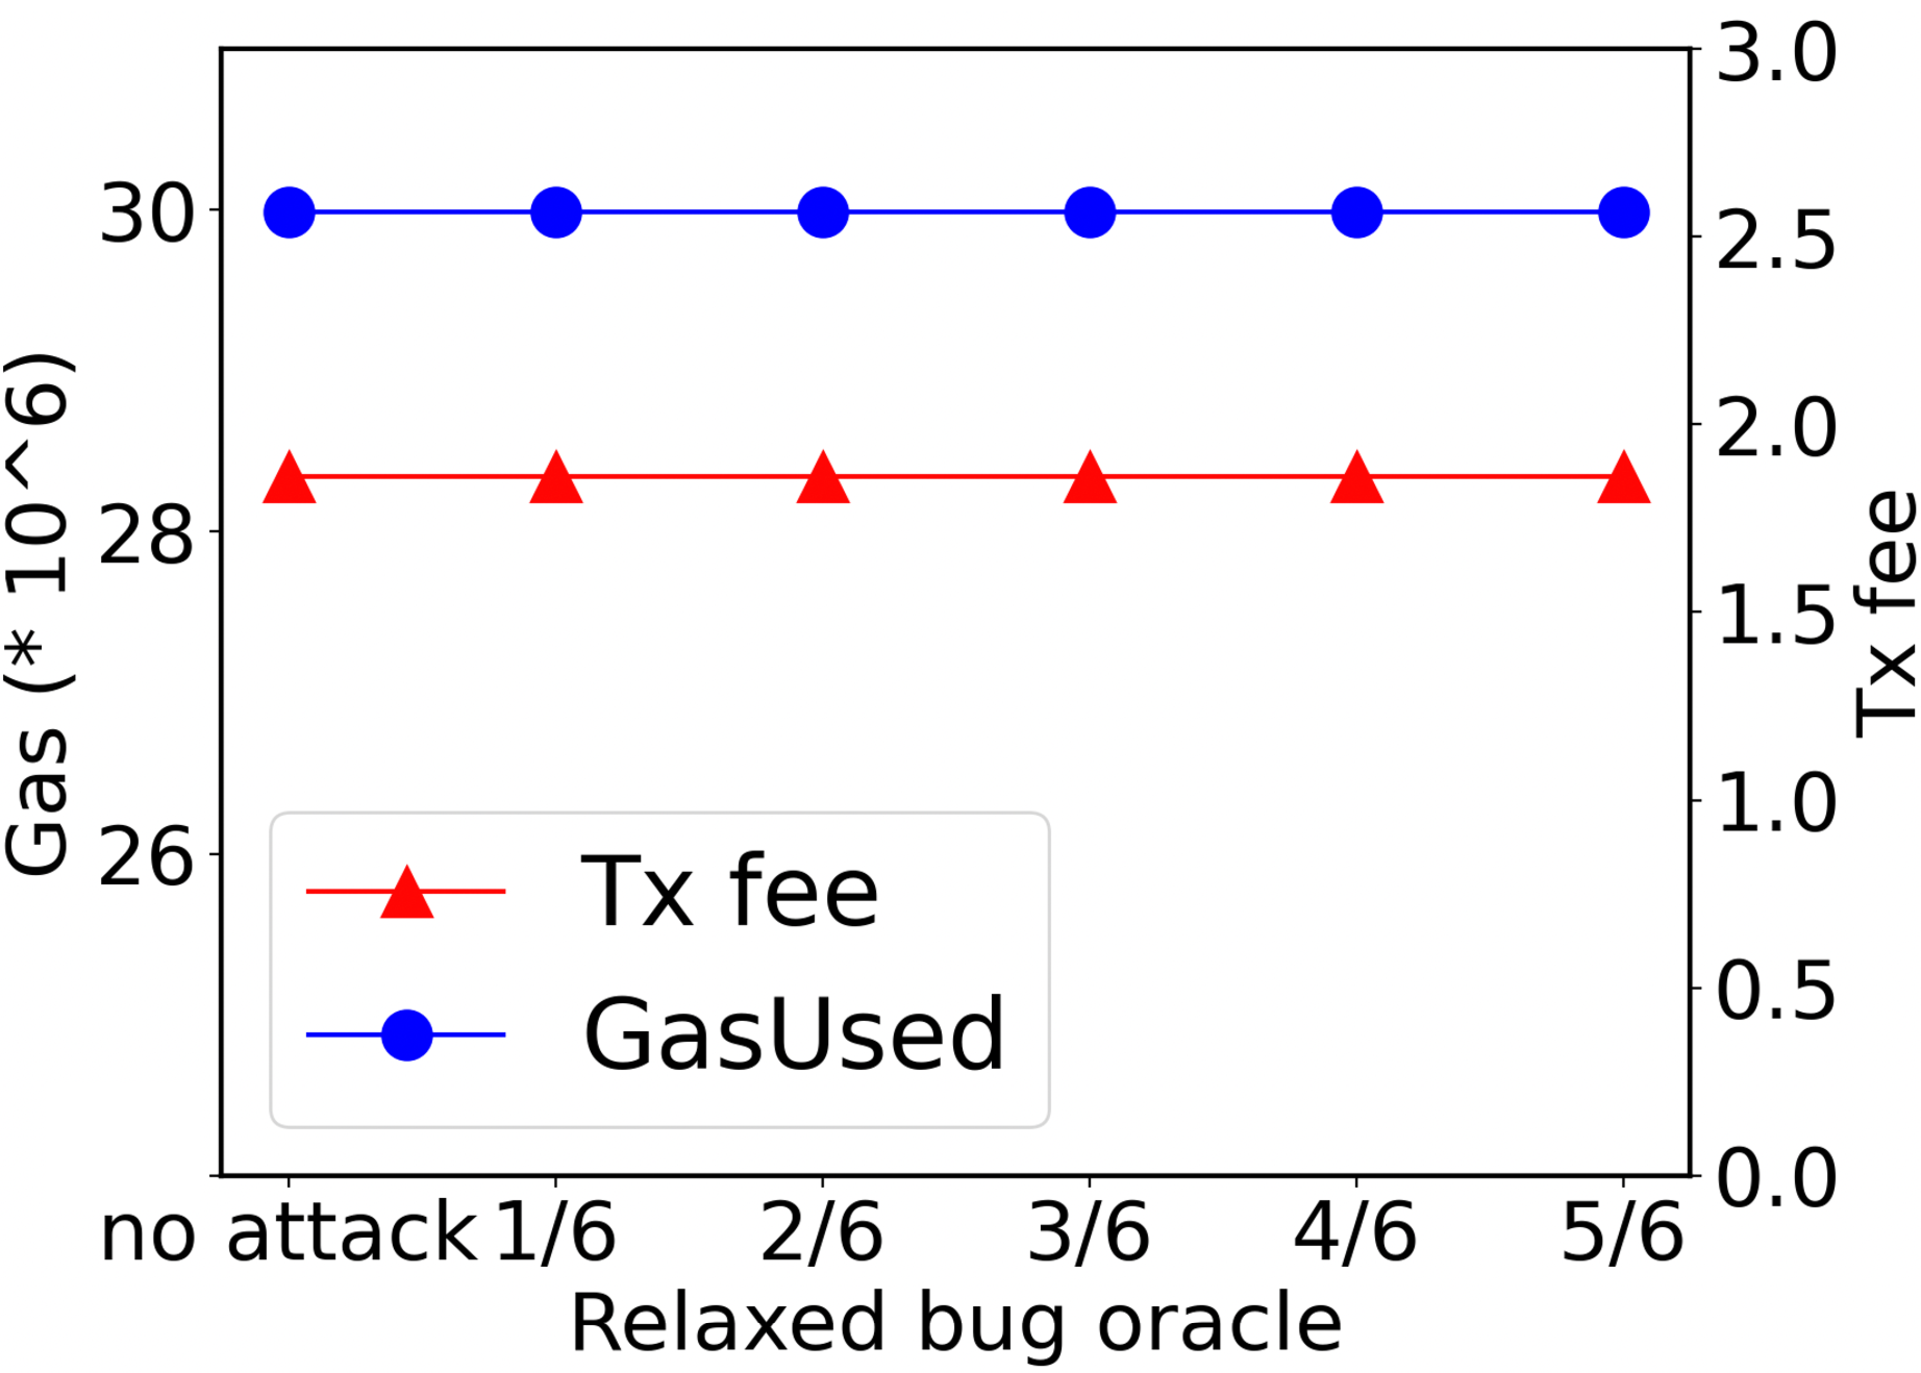}
  \caption{Attack evaluation with relaxed bug oracle}
  \label{fig:relax-bug-oracle}
  \end{figure}

\begin{eqnarray}
\label{eqn:relaxed:evict:1}
m - ||st_{nN}||& >& t
\\
asym_E(st_0, ops) &\stackrel[]{def}{=}& \frac{\sum_{tx\in{}st_{nA}}tx.fee}{\sum_{tx\in{}st_0/st_{nN}}tx.fee} 
\\
\label{eqn:relaxed:evict:2}
asym_E(st_0, ops) &<& \epsilon
\end{eqnarray}
\end{definition}

When evaluating the true positive rate of exploits discovered by the relaxed bug oracle, we accordingly modify the criteria for a successful eviction attack as not all normal transactions are evicted. Given a mempool full of normal transactions, it is a successful eviction attack if the synthesized attack meets the following conditions: 1) At least the same proportion of normal transactions is evicted, that is $t/m* mempool-length$. 2) The $asym_E$ of the synthesized attack is not larger than the $\epsilon$ in MUT that is set to find the exploit. 3) The total transaction fee (including that of attack transactions and normal transactions) of the next block is less than that of no attack. The third condition requires that the validator’s revenue is damaged by the attack compared to the scenario without the attack. The rationale for adding the third condition is the normal transactions left in $st_n$ can be included in the next block. If sufficient normal transactions are remaining to fill the next block, the validator's revenue will not decrease. In such cases, we do not consider this scenario as a successful eviction attack. 

%In the evaluation, we set various $t$ in the relaxed bug oracle when fuzzing MUT. Then, we synthesize the attack to evict at least the same proportion of normal transactions in the default configuration. At last, we launch the attack and report whether the attack meets the three conditions described above. 

We present the evaluation result of oracles with various $t$ on Geth $<v1.11.4$ with $m = 6$ as shown in Table~\ref{tab:false-positve}. We use $t/m$ to denote the oracles. When fuzzing with the \textsc{mpfuzz} bug oracle ($6/6$), \textsc{mpfuzz} finds $6$ unique exploits as reported in Table~\ref{sec:exploits}. All $6$ exploits are successful eviction attacks as evaluated in \S~\ref{sec:evaluate} and \S~\ref{appdx:sec:additional-attack-evaluation}. Thus, the true positive rate is $100\%$.

When fuzzing with a relaxed bug oracle on the same MUT with $t=5$, the fuzzer finds $9$ unique exploits. Among the $9$ exploits, $6$ of them are discovered in \textsc{mpfuzz} bug oracle; $3$ new exploits are discovered where the end state leaves $1$ normal transaction. However, the attack evaluation results show that all these $3$ new exploits are false positives because they do not satisfy the third condition of a successful eviction attack. In our attack evaluation, we drive the workload collected from Mainnet as normal transactions and report the total transaction fee and the block $GasUsed$ in the next block. As shown in Figure~\ref{fig:relax-bug-oracle}, we launch a $XT_4$ based attack with various $t$. In all the settings, $148$ high-priced normal transactions are included to fill the block. The attacks cannot damage the normal transactions included in the next block or the revenue of the validator. Thus, the $3$ new exploits are false positives. Similarly, when fuzzing with a relaxed bug oracle with $t=4$ and $t=3$, the fuzzer finds $12$ and $15$ unique exploits with $50\%$ and $40\%$ true positive rates respectively.

\begin{table}[!htbp]
  \caption{Evaluation on true positives}
  \label{tab:false-positve}
  \centering{\small
  \begin{tabularx}{0.47\textwidth}{ |l|X|l|l|l| }
  \hline
 Bug oracle & $6/6$ (\textsc{mpfuzz}) & $5/6$ & $4/6$& $3/6$\\\hline 
  \# exploits (MUT) &$6$&$9$ & $12$ & $15$ \\ \hline 
  TP rate & $\textbf{100\%}$ &$66.7\%$ & $50\%$ & $40\%$\\ \hline 
\end{tabularx}
}
\end{table}
}}

\section{Additional FP/TP Results}
\label{appdx:sec:fp}

\begin{figure}[!ht]
  \centering
  \subfloat[Eviction attack]{%
  \includegraphics[width=0.225\textwidth]{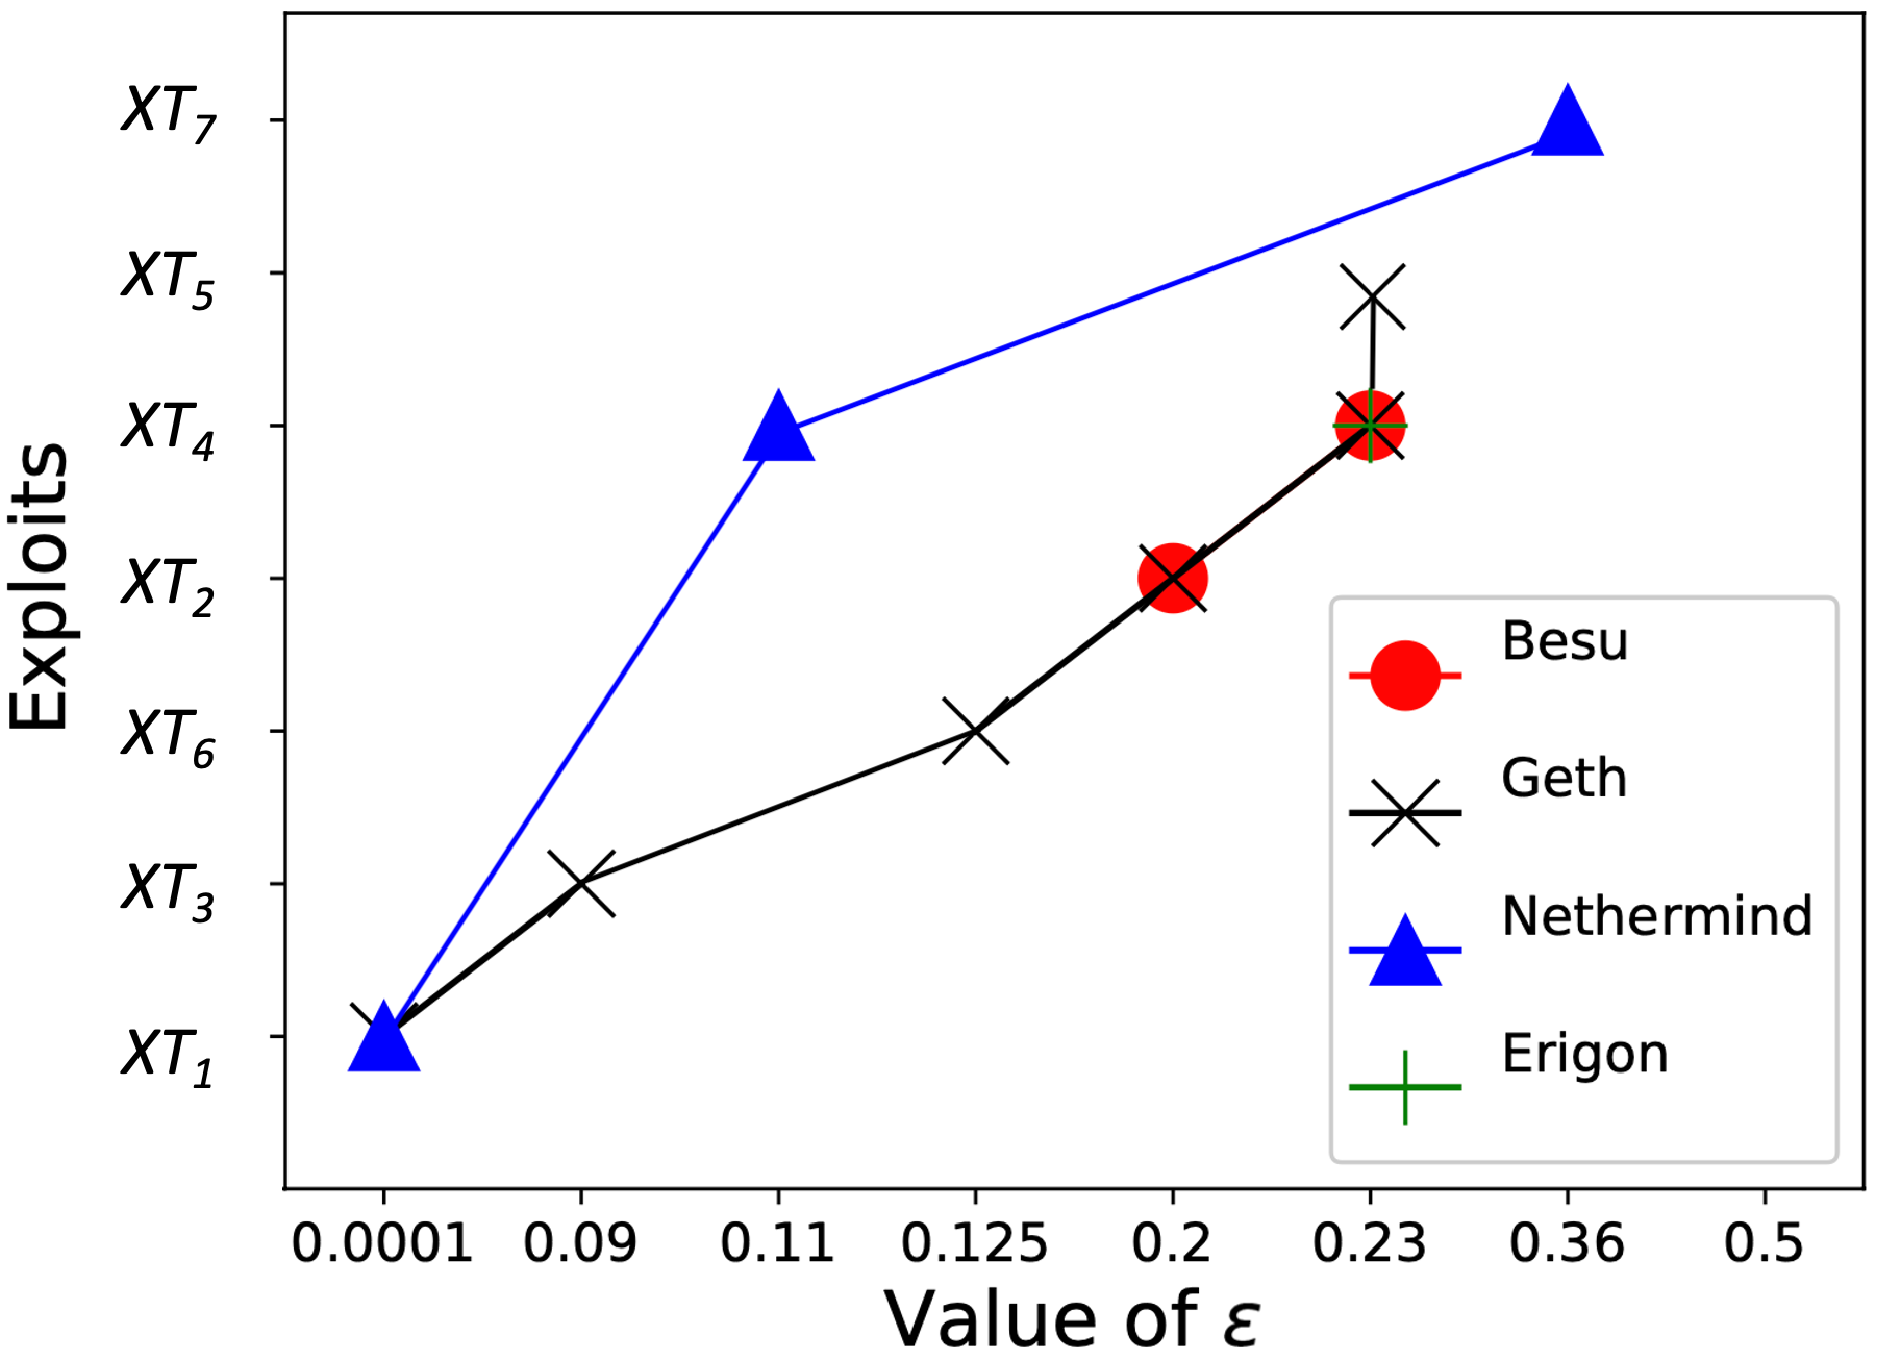}
  \label{fig:evaluation-epsilon}
    }%
    \subfloat[Locking attack]{%
  \includegraphics[width=0.225\textwidth]{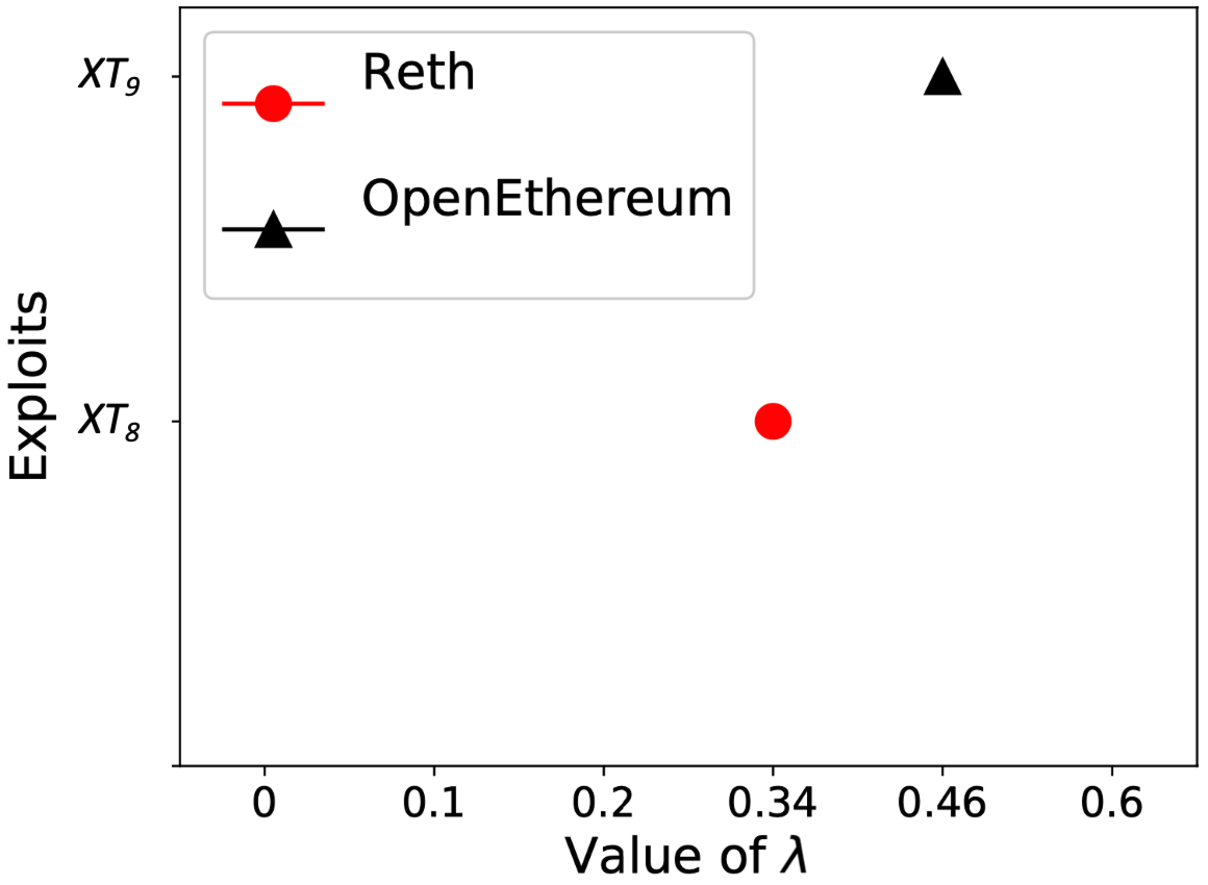}
  \label{fig:evaluation-lambda}}
  \caption{Evaluation of FP under varying $\epsilon$ and $\lambda$}%
  %\label{fig:erigon-local}
\end{figure}

Specifically, Figure~\ref{fig:evaluation-epsilon} shows that with increasing oracle parameter $\epsilon$, more short exploits are found on MUT, and each newly found unique exploit can be extended to a true positive actual exploit; this result leads to a $100\%$ true positive rate for eviction attacks with $\epsilon<0.5$ across Ethereum clients. 
Figure~\ref{fig:evaluation-lambda} shows similar results that each short exploit found by \textsc{mpfuzz} can be extended to a true positive actual exploit on the target Ethereum client. The true-positive rate remains at $100\%$ for $\lambda < 0.6$ across Ethereum clients.

{ 
\section{Additional Ablation Study}
Besides B1, B2, B3, and B4, We build two more baseline fuzzers, namely B5 and B6, for ablation study to demonstrate the performance efficacy of three techniques in \textsc{mpfuzz}, including mutation feedback and input mutation.

\noindent{\bf Baseline B5:} Compared to \textsc{mpfuzz}, the only difference is that the baseline B5  takes concrete state coverage as feedback, while \textsc{mpfuzz} takes symbolized state coverage as feedback. The concrete state coverage is implemented the same as Baseline B2 described in \S~\ref{sec:eval:fuzz}. Specifically, if an input transaction sequence increases the concrete-state coverage, the input-concrete-state pair as a seed is added to the corpus. However, the energy of a state is determined the same way as \textsc{mpfuzz}. Specifically, given the concrete state of a seed, the energy is determined by its symbolized state.  

\noindent{\bf Baseline B6:} We build the last baseline fuzzer, which is also similar to \textsc{mpfuzz} but without symbolized input mutation. In each iteration, the baseline fuzzer B6 appends to the current transaction sequence a new transaction. Given the m-slot mempool, the fuzzer tries $m$ values for senders, $m$ values for nonces, $m$ values for Gas price, and $m$ values for Ether amount. After sending to the mempool the current transaction sequence, it uses the same way to determine the state coverage and energy as \textsc{mpfuzz}.

We run the baseline B4, B5, B6 and \textsc{mpfuzz} against a Geth client under various mempool sizes. We run the fuzzers for $16$ hours and report the time used that the first exploit is found. 

\begin{table}[!htbp] %force in current page, disable float.
\caption{Fuzzing Geth $v1.11.3$'s mempool (in minutes) by different approaches to detect Exploit $XT_3$. OT means overtime.}
\label{appdx:tab:vs:baselines}
\centering{\footnotesize
%p{1.5cm}
\begin{tabularx}{0.49\textwidth}{ |X|c|c|c|c|c|c|c| }
  \hline
Settings & B1 & B2  & B3 & B4 & B5 &B6&\textsc{mpfuzz} \\ \hline
$6$slot-$2$h & OT & $54$ & $8$ &$1.22$ & $0.10$& $34.61$ &$0.03$ 
\\ \hline
$16$slot-$16$h & OT & OT & $447$ & OT &$0.26$& OT& $0.06$ 
\\ \hline
\end{tabularx}
}
\end{table}

Table~\ref{appdx:tab:vs:baselines} presents the running time of different baselines in comparison to that of \textsc{mpfuzz}.

Figure~\ref{fig:ablation} reports the result under various mempool sizes. All the fuzzers of B4, B5, B6 and \textsc{mpfuzz} can find the first exploit in $10$ minutes when the mempool size is not larger than $6$ slots. For the settings that mempool size is larger than $6$ slots, B4 and B6 cannot find any attack in $16$ hours, while B5 and \textsc{mpfuzz} can find the first exploit (i.e., $XT_3$) with the setting of $512$ slots in $177$ and $1$ mutinus respectively. 

\begin{figure}[!tb]
  \centering
  \includegraphics[width=0.275\textwidth]{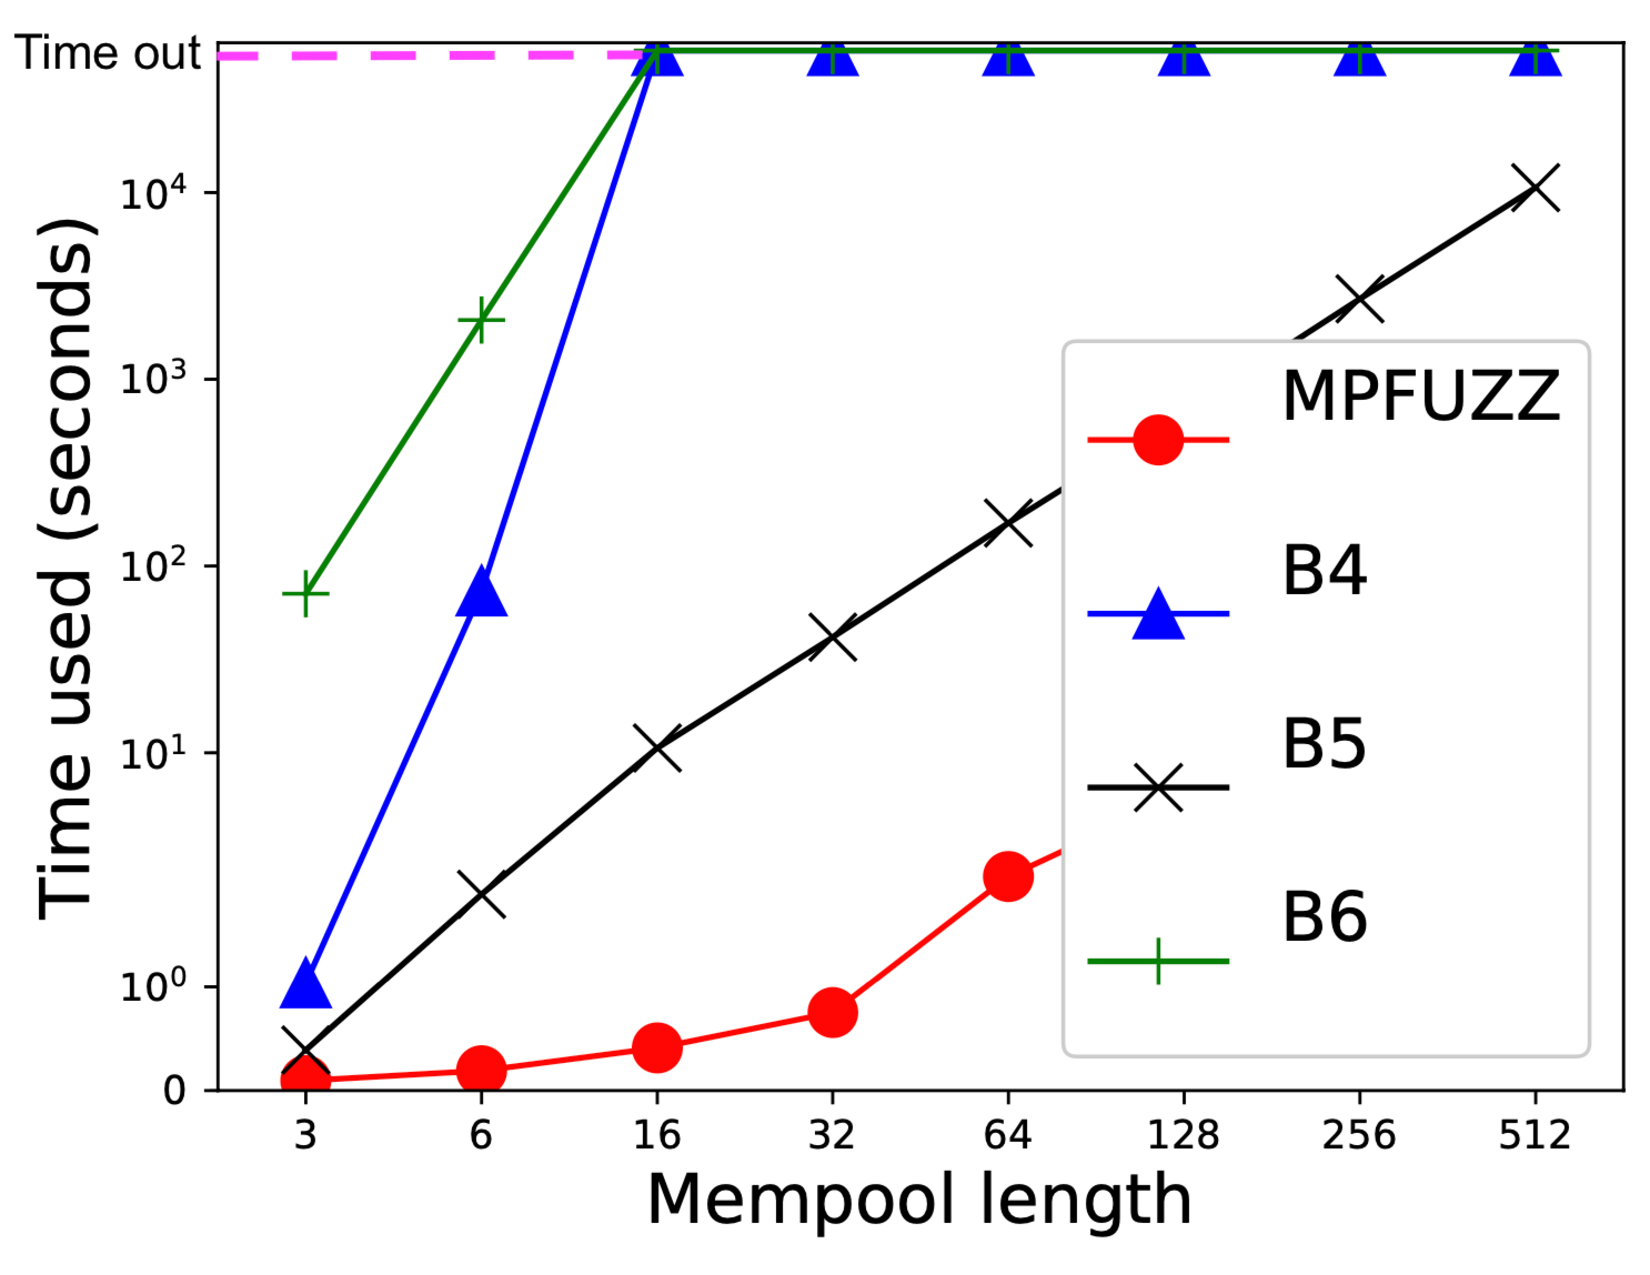}
  \caption{Ablation study}
  \label{fig:ablation}
  \end{figure}

As B5 is more performant compared to the other two baselines, it shows the mutation feedback improves efficiency less compared to that of the seed energy and input mutation. The result that B6 is more performant than B4 shows input mutation has the greatest improvement in efficiency.

\ignore{
\section{Evaluation of Exploit Detection with Varying $\epsilon$ and $\lambda$}
Recall the definition of the bug oracle in \S~\ref{sec:oracle}, this section evaluates the exploits discovery with varying $\epsilon$ and $\lambda$. We first change the value of $\epsilon$ and $\lambda$ in the bug oracle and run the \textsc{mpfuzz} to report the number of distinct exploits found in the MUT. 

%Then, we evaluate the value of $asym_E$ and $asym_D$ in the real-world attack that the mempool of default configuration runs in a node and receives Ethereum Mainnet workloads as normal transactions. The Mainnet workload collection is described in \S~\ref{sec:setup:singlenode}.

In the evaluation of $\epsilon$ in the eviction bug oracle, we run \textsc{mpfuzz} on a $16$-slot mempool of different clients, including Geth, Besu, Nethermind and Erigon. As shown in Figure~\ref{fig:evaluation-epsilon}, when the $\epsilon$ is set to $0.0001$, \textsc{mpfuzz} finds two exploits (i.e., $XT_1$ and $XT_6$) in Geth and one exploit (i.e., $XT_1$) in both Besu and Nethermind. As $\epsilon$ increases, more exploits are discovered. When the $\epsilon$ is set to $0.4$, all the exploits we reported are discovered. 

\begin{figure}[!ht]
  \centering
  \subfloat[Eviction attack]{%
  \includegraphics[width=0.225\textwidth]{figures/beta-evaluation.eps}
  \label{fig:evaluation-epsilon}
    }%
    \subfloat[Locking attack]{%
  \includegraphics[width=0.225\textwidth]{figures/lambda-evaluation.eps}
  \label{fig:evaluation-lambda}}
  \caption{Exploit evaluation with varying $\epsilon$ and $\lambda$}%
  \label{fig:erigon-local}
\end{figure}

In the evaluation of $\lambda$ in the locking bug oracle, we run \textsc{mpfuzz} on a $16$-slot mempool of Reth and OpenEthereum. As shown in Figure~\ref{fig:evaluation-lambda}, we found $XT_8$ on Reth and $XT_9$ on OpenEthereum with $\lambda$ setting to $0.34$ and $0.5$ respectively. 
}

\ignore{
\section{Appendix}
\label{appdx:sec:eval:asym}

In this section, we evaluate the value of $asym_E$ of a given attack with varying mempool sizes. Specifically, we evaluate the $asym_E$ of $XT_6$ and $XT_4$ on Geth and $XT_4$ on Nethermind, with the setting of $16$ slots, $32$ slots and default configuration. In the default mempool configuration, we drive the Mainnet workload we collected as normal transactions. The Mainnet workload collection is described in \S~\ref{sec:setup:singlenode}. As shown in Table~\ref{tab:beta-attack}, the $asym_E$ of a given attack is smaller than the $\epsilon$ we set in the bug oracle when fuzzing on MUT. In the attack of $XT_6$, the $asym_E$ is always $0$ as the attack has no Ether cost. In $XT_4$, as the mempool size increases, $asym_E$ becomes smaller which shows the damage caused by the attack will be magnified as the mempool size increases.

\newcommand\Tstrut{\rule{0pt}{2.2ex}} 
\newcommand\Bstrut{\rule[-1.5ex]{0pt}{0pt}}
\begin{table}[!htbp]
  \caption{The value of $\epsilon$ in attacks}
  \label{tab:beta-attack}
  \centering{\footnotesize
  \begin{tabularx}{0.47\textwidth}{ |X|l|l|l|l| }
  \hline
  Exploit & $\epsilon$ &\multicolumn{3}{c|}{$asym_E$}\Tstrut\Bstrut\\ \cline{2-5} 
  & $m = 16$ & $m = 16$ & $m = 32$& Default $m$\\\hline 
  $XT_1$-Geth & $0.0001$ & $0$ & $0$ & $0$ \\ \hline
  $XT_1$-Nethermind & $0.0001$ & $0$ & $0$ & $0$ \\ \hline
  $XT_3$-Geth & $0.09$ & $0.083$ & $0.042$ & $0.0002$ \\ \hline
  $XT_4$-Nethermind& $0.11$& $0.104$ & $0.052$ & $0.0008$\\ \hline 
  $XT_6$-Geth & $0.125$ & $0.125$ & $0.062$ & $0.0003$ \\ \hline
  $XT_2$-Geth & $0.2$ & $0.167$ & $0.084$ & $0.0698$ \\ \hline
  $XT_2$-Besu & $0.2$ & $0.167$ & $0.084$ & $0.0754$ \\ \hline
  $XT_4$-Geth & $0.23$ &$0.208$ & $0.105$ & $0.0768$\\ \hline 
  $XT_5$-Geth & $0.23$ &$0.208$ & $0.105$ & $0.0768$\\ \hline
  $XT_4$-Besu & $0.23$ & $0.208$ & $0.105$ & $0.0083$ \\ \hline
  $XT_4$-Erigon & $0.23$ & $0.208$ & $0.105$ & $0.0894$ \\ \hline
  $XT_7$-Nethermind & $0.36$ & $0.355$ & $0.344$ & $0.0012$ \\ \hline
\end{tabularx}
}
\end{table}

We then evaluate the $asym_D$ of $XT_8$ and $XT_9$ with varying mempool sizes. As shown in Table~\ref{tab:lambda-attack}, the $asym_D$ of $XT_8$ in default configuration is much smaller than the $\lambda$ we set in the bug oracle when fuzzing on MUT. In the default configuration, the attacker sends attack transactions with minimal price to decline higher-priced normal transactions, which means the price of the attack transactions is significantly lower than that of normal transactions. In $XT_9$, as the mempool size increases, $asym_D$ becomes smaller because low-price attack transactions lock more slots.

\begin{table}[!htbp]
  \caption{The value of $\lambda$ in attacks}
  \label{tab:lambda-attack}
  \centering{\footnotesize
  \begin{tabularx}{0.41\textwidth}{ |X|l|l|l|l| }
  \hline
 Exploit & $\lambda$ &\multicolumn{3}{c|}{$asym_D$}\Tstrut\Bstrut\\ \cline{2-5} 
  & $m = 16$ & $m = 16$ & $m = 32$& Default $m$\\\hline 
  $XT_8$ &$0.34$&$0.34$ & $0.34$ & $0.015$ \\ \hline 
  $XT_9$ &$0.46$ &$0.46$ & $0.39$ & $0.0439$\\ \hline 
\end{tabularx}
}
\end{table}
}

\ignore{}
\section{Discussion: Private and public transactions}
\label{sec:privatepool}

\begin{figure}[!tb]
  \centering
  \includegraphics[width=0.4\textwidth]{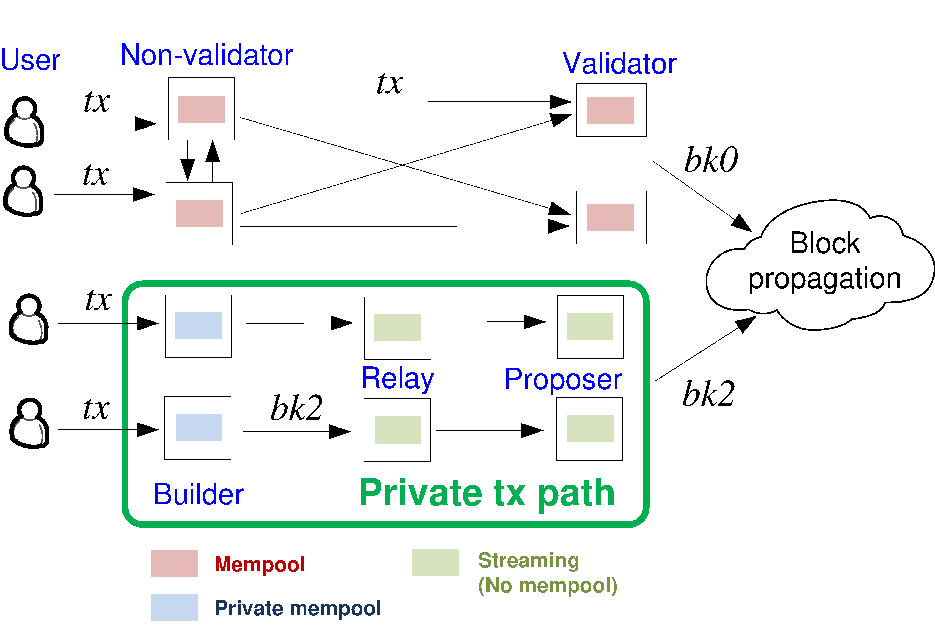}
  \caption{Two transaction routes to reach validators: A public transaction route by propagation to all validators and a private transaction route to participating validators without propagation (in the green box).}
  \label{fig:eth2:tworoutes}
  \end{figure}

\noindent{\bf Public and private transactions}:
In Ethereum 2.0, unconfirmed transactions follow two alternative paths to reach a validator. First, transactions are broadcast in the blockchain network by relay nodes to (eventually) reach {\it all} validators, among which the selected one proposes the next block, including the transaction in it. Along this path, each relay or validator node maintains its own mempool to buffer unconfirmed transactions.

Second, transactions can be sent to the PBS path (proposal builder separation) where transactions are propagated privately. That is, once a transaction is received by a builder node or a searcher node, as depicted in Figure~\ref{fig:eth2:tworoutes}, it will only be propagated to the relay node and proposer/validator specified by the builder or searcher. Other searchers and builders will not be able to see the transaction until the block including the transaction is broadcast in the network. This is in contrast to the public transaction path where the node receiving a transaction, be it either validator or non-validator, would propagate it to any other node in the network. The private transaction path is essential to protecting transactions under MEV. 

In PBS, builders maintain their mempools to buffer unconfirmed private transactions until they are included in a block or expired. Note that relays and proposers don’t need to buffer transactions/blocks or maintain no mempools since blocks are streamed and unselected blocks/transactions are dropped immediately.

\noindent{\bf Design of public mempool}: Because public transactions are broadcast, given $n$ users sending public transactions, the public mempool of any node receives $O(n)$ public transactions. Therefore, the public mempool needs to limit its capacity by a constant $O(1)$ so that it can scale w.r.t. $n$; otherwise, the computing resources of a node can be exhausted.

\noindent{\bf Design of private mempool}:
In PBS, a user can send a transaction to multiple block builders, or a block builder can receive transactions from multiple users. Thus, the mempool on a block builder can grow linearly with the number of users in the system. When scaling to high (private) transaction volume, a transaction pool of no capacity limit can be easily exhausted under normal transactions and be DDoS-attacked under adversarial transactions. 

A private mempool of limited capacity needs to handle the case of a full mempool. More specifically, it needs a policy to decide which transactions to evict upon a full mempool. In other words, designing a mempool in the private transaction path (specifically, on the block builders and searchers) is no different from designing that in the public transaction path.
