# Supplementary material for: Towards Automated Discovery of Asymmetric Mempool DoS in Blockchains
Source: arXiv:2312.02642 source file (2025-05-26)
Supplement: Supplementary file 3 [file wellmarked_appendix.tex]

\subsection{Further Rationale of Symbolization}
\label{appdx:sec:sym:rationale}

%\noindent{\bf Design rationale}: 
We now describe the design rationale of our symbolization technique. 
%We aim to explain why \textsc{mpfuzz} can instantiate a symbol to a much smaller subset (than the defining space), without losing the fuzzing utility (i.e., without missing exploits).

\begin{itemize}
\item
The first observation is that {\it real-world mempools admit transactions based on the symbolic value, not concrete value, of nonce and Ether amount}. Our design reflects this intuition. For instance, symbols of valid transactions, e.g., $\mathcal{P}, \mathcal{C}, \mathcal{N}$, are instantiated by \textsc{mpfuzz} to a minimal amount $1$ Ether. As long as the transferred Ether amount does not exceed the sender balance, transactions remain valid (i.e., no overdraft). Admission decisions remain the same for two valid transactions despite their difference in nonces or Ether amounts.  

Likewise, Symbol $\mathcal{F}$ is instantiated by \textsc{mpfuzz} to fixed nonce $n+1$: As long as the nonce is non-consecutive, no matter what specific value it takes (e.g., $3$ or $m+1$), the mempool would deem it as a future transaction and makes the same admission decision. 

\item
The second observation is that {\it restricting eviction/replacement victims to only parent transactions can facilitate finding exploits quickly}. Specifically, while any transactions can be evicted/replaced, \textsc{mpfuzz} evicts/replaces only parent transactions; such a strategy can cause maximal damage (i.e., the most child transactions turned) while saving the search space. Our symbol design reflects this idea. For instance, Symbol $\mathcal{R}$ covers any transaction of the same sender and nonce as a transaction in state $st$, but it is instantiated by \textsc{mpfuzz} to only the transaction of nonce $1$ (i.e., replacing a parent transaction).

For another instance, Symbol $\mathcal{C}$ is instantiated to a high Gas price $m+4$, Symbol $\mathcal{P}$ is instantiated to medium price $[4,m+3]$, and Symbol $\mathcal{N}$ is instantiated to a low price $3$. So, $\mathcal{C}$ can evict $\mathcal{P}$ or $\mathcal{N}$.
\end{itemize}

%\input{text/buffer2.tex}\clearpage
%\input{text/wellmarked_appendix-overpage.tex}

%%%%%%%%%%%%%%%%%%OVERPAGE%%%%%%%%%%%%%%%%%%%%%
